# Supplementary material for: Evolving Loop Programs: Discovering How Frozen Transformers Should Loop
Source: arXiv:2611.41108 source file (2026-12-03)
Supplement: Supplementary file 1 [file 5_supp.tex]

\makeatletter
\@namedef{suppbiblabel@fishman2026dory}{S1}
\@namedef{suppbiblabel@pyatkin2025ifbench}{S2}
\@namedef{suppbiblabel@tian2024scicode}{S3}
\@namedef{suppbiblabel@bae2025relaxed}{S4}
\@namedef{suppbiblabel@bai2019deq}{S5}
\@namedef{suppbiblabel@banino2021pondernet}{S6}
\@namedef{suppbiblabel@chen2024diffusionforcing}{S7}
\@namedef{suppbiblabel@chen2018neuralode}{S8}
\@namedef{suppbiblabel@chen2025itt}{S9}
\@namedef{suppbiblabel@deepseek2025r1}{S10}
\@namedef{suppbiblabel@elhoushi2024layerskip}{S11}
\@namedef{suppbiblabel@fan2025lengthgen}{S12}
\@namedef{suppbiblabel@gatmiry2024loopedgd}{S13}
\@namedef{suppbiblabel@giannou2023looped}{S14}
\@namedef{suppbiblabel@graves2016act}{S15}
\@namedef{suppbiblabel@hao2025coconut}{S16}
\@namedef{suppbiblabel@hu2025adas}{S17}
\@namedef{suppbiblabel@lan2020albert}{S18}
\@namedef{suppbiblabel@liu2025teacache}{S19}
\@namedef{suppbiblabel@liu2019darts}{S20}
\@namedef{suppbiblabel@liu2025taylorseer}{S21}
\@namedef{suppbiblabel@lu2022dpmsolver}{S22}
\@namedef{suppbiblabel@ma2025scalingdiff}{S23}
\@namedef{suppbiblabel@ma2024deepcache}{S24}
\@namedef{suppbiblabel@raposo2024mod}{S25}
\@namedef{suppbiblabel@schuster2022calm}{S26}
\@namedef{suppbiblabel@snell2025testtime}{S27}
\@namedef{suppbiblabel@song2025history}{S28}
\@namedef{suppbiblabel@wei2022cot}{S29}
\@namedef{suppbiblabel@yang2024looped}{S30}
\@namedef{suppbiblabel@yin2025causvid}{S31}
\@namedef{suppbiblabel@zhao2023unipc}{S32}
\@namedef{suppbiblabel@balaji2022ediffi}{S33}
\@namedef{suppbiblabel@chen2024gits}{S34}
\@namedef{suppbiblabel@choi2022p2}{S35}
\@namedef{suppbiblabel@esser2024sd3}{S36}
\@namedef{suppbiblabel@gurnee2026workspace}{S37}
\@namedef{suppbiblabel@kynkaanniemi2024interval}{S38}
\@namedef{suppbiblabel@liu2022pndm}{S39}
\@namedef{suppbiblabel@loshchilov2025ngpt}{S40}
\@namedef{suppbiblabel@lv2025fastercache}{S41}
\@namedef{suppbiblabel@sabour2024ays}{S42}
\@namedef{suppbiblabel@skean2025layer}{S43}
\@namedef{suppbiblabel@sun2025painters}{S44}
\@namedef{suppbiblabel@tml2026inkling2}{S45}
\@namedef{suppbiblabel@vendrell2026melt}{S46}
\@namedef{suppbiblabel@yang2026flashloop}{S47}
\@namedef{suppbiblabel@zhao2025pab}{S48}
\@namedef{suppbiblabel@ji2025memflow}{S49}
\DeclareRobustCommand{\citesupp}[1]{%
  [\begingroup\def\@suppsep{}%
  \@for\@suppkey:=#1\do{%
    \@suppsep\def\@suppsep{, }%
    \@ifundefined{suppbiblabel@\@suppkey}{?}{\hyperref[suppbib:\@suppkey]{\@nameuse{suppbiblabel@\@suppkey}}}%
  }\endgroup]}
\makeatother

\input{sec/appendix_vocabulary}
\input{sec/appendix_benchmark_results}
\input{sec/appendix_search_design}
\input{sec/appendix_looped_dit}

\clearpage
\input{sec/appendix_observations}

\clearpage
\input{sec/appendix_prompts}

\FloatBarrier
\input{sec/appendix_experiment_settings}

\FloatBarrier
\input{sec/appendix_human_alignment}

\FloatBarrier
\input{sec/appendix_related_work}

\FloatBarrier
\input{sec/appendix_references}
