# Supplementary material for: Evolving Loop Programs: Discovering How Frozen Transformers Should Loop
Source: arXiv:2611.41108 source file (2026-12-03)
Supplement: Supplementary file 2 [file fig_qualitative_supp.tex]

\begingroup
\input{figs/qualitative_layout}
\begin{tabular}{@{}ccccc@{\hspace{7pt}}ccccc@{}}
\qualcomparisonheader

\multicolumn{5}{p{0.474\textwidth}}{\footnotesize\textbf{Attribute binding}\quad\scriptsize\emph{``\ldots yellow rabbit \ldots red-framed glasses \ldots''}} &
\multicolumn{5}{p{0.474\textwidth}}{\footnotesize\textbf{Object composition}\quad\scriptsize\emph{``\ldots yellow school bus \ldots white van \ldots''}} \\[2pt]
\qualdetail{\includegraphics[width=\qualwidth]{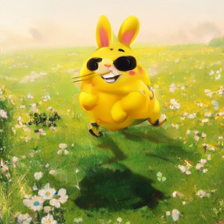}}{\includegraphics[width=\qscaledwidth]{figs/qualitative/sr_dpg_378_base_full.jpg}}{56}{32}{168}{120}{lpsReferenceDark} &
\qualdetail{\includegraphics[width=\qualwidth]{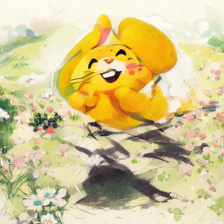}}{\includegraphics[width=\qscaledwidth]{figs/qualitative/sr_dpg_378_base_s10.jpg}}{56}{32}{168}{120}{lpsReferenceDark} &
\qualdetail{\includegraphics[width=\qualwidth]{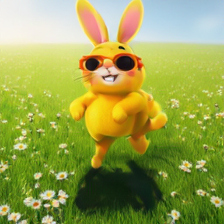}}{\includegraphics[width=\qscaledwidth]{figs/qualitative/sr_dpg_378_loop_nolg.jpg}}{56}{32}{168}{120}{lpsReferenceDark} &
\qualdetail{\includegraphics[width=\qualwidth]{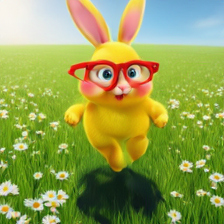}}{\includegraphics[width=\qscaledwidth]{figs/qualitative/sr_dpg_378_loop_lg.jpg}}{56}{32}{168}{120}{lpsReferenceDark} &
\qualdetail{\includegraphics[width=\qualwidth]{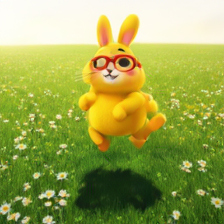}}{\includegraphics[width=\qscaledwidth]{figs/qualitative/sr_dpg_378_ours.jpg}}{56}{32}{168}{120}{lpsOurs} &
\qualdetail{\includegraphics[width=\qualwidth]{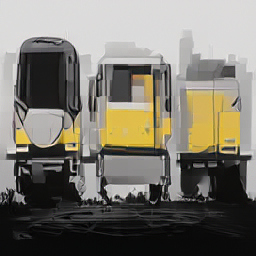}}{\includegraphics[width=\qscaledwidth]{figs/qualitative/rv_dpg_802_base_full.jpg}}{70}{60}{210}{170}{lpsReferenceDark} &
\qualdetail{\includegraphics[width=\qualwidth]{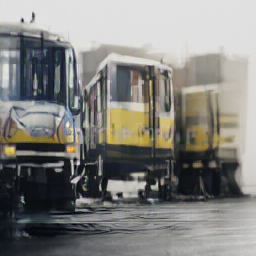}}{\includegraphics[width=\qscaledwidth]{figs/qualitative/rv_dpg_802_base_s10.jpg}}{70}{60}{210}{170}{lpsReferenceDark} &
\qualdetail{\includegraphics[width=\qualwidth]{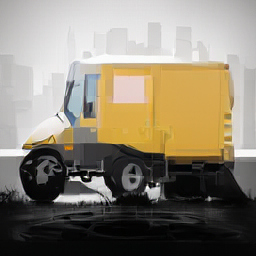}}{\includegraphics[width=\qscaledwidth]{figs/qualitative/rv_dpg_802_loop_nolg.jpg}}{70}{60}{210}{170}{lpsReferenceDark} &
\qualdetail{\includegraphics[width=\qualwidth]{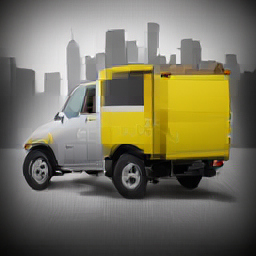}}{\includegraphics[width=\qscaledwidth]{figs/qualitative/rv_dpg_802_loop_lg.jpg}}{70}{60}{210}{170}{lpsReferenceDark} &
\qualdetail{\includegraphics[width=\qualwidth]{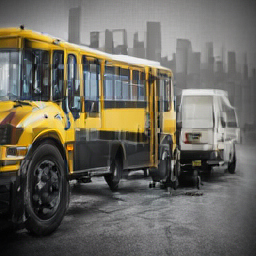}}{\includegraphics[width=\qscaledwidth]{figs/qualitative/rv_dpg_802_ours.jpg}}{70}{60}{210}{170}{lpsOurs} \\[1pt]
\scriptsize\qualbad{Dark lens (0.90)} & \scriptsize\qualbad{Blob (0.70)} & \scriptsize\qualbad{Dark lens (0.90)} & \scriptsize\qualbad{Warped (0.90)} & \scriptsize\qualgood{Red rim (1.00)} &
\scriptsize\qualbad{Blocks (0.10)} & \scriptsize\qualbad{Blocks (0.30)} & \scriptsize\qualbad{Toy cart (0.40)} & \scriptsize\qualbad{Pickup (0.20)} & \scriptsize\qualgood{Bus+van (1.00)} \\
\end{tabular}
\endgroup
