# Supplementary material for: Evolving Loop Programs: Discovering How Frozen Transformers Should Loop
Source: arXiv:2611.41108 source file (2026-12-03)
Supplement: Supplementary file 3 [file appendix_benchmark_results.tex]

\section{Complete Benchmark Results}
\label{sec:supp_benchmark_results}
\label{sec:supp_balanced_tables}

This section expands the text-to-image comparisons in RQ1, the long- and short-video evaluations in RQ3 (with the $60$\,s multi-prompt initial-context study in Appendix~\ref{sec:supp_context_ablation}), and text reasoning across pretrained looped (\texttt{Dory1.0-4B}) and unlooped (\texttt{Qwen3-4B}) language models in RQ4. We retain the main paper's distinction between models trained without loops and models trained with loops. All pretrained weights remain fixed during offline search and subsequent replay; selected programs execute without further calls to the search LLM. Speed, Balanced, and Quality name operating points with different priorities. DPG denotes DPG-Bench. Throughout the supplementary tables, \textbf{bold} and \underline{underlined} values mark best and second-best results within the displayed comparison group; gray shading identifies our programs. Reported costs are inference TFLOPs unless explicitly marked as measured wall-clock latency (s/img or s/video) and wall-clock speedup; all costs exclude offline search overhead. Appendix~\ref{sec:supp_exp_settings} details the evaluation scopes, dataset splits, and checkpoint provenance across all nine backbones.

\subsection{Text-to-Image Diffusion: Models Trained without Loops}
\label{sec:supp_unlooped_results}

\Cref{tab:supp_main_results_balanced} expands \cref{tab:main_results} with full GenEval subtasks, Scale-RAE's $12$-step Balanced program, matched $10$-step no-loop controls, held-out splits, and RTX~5090 wall-clock timings. Why do our $6$--$14$-step programs outperform $25$- and $50$-step Loop~+~LG while naive $10$-step inference collapses on both backbones? In text-to-image diffusion, compositional layout and object-attribute binding crystallize during the high-noise early half ($t/(T{-}1){\le}0.5$), whereas late outer steps mainly refine high-frequency texture; concentrating recurrence early while eliminating redundant outer evaluations via one-step guidance-correction reuse (Scale-RAE) or shared unlooped prefixes and cached conditioning (RAE) preserves layout fidelity at a fraction of the compute. Across the $1{,}298$ unseen held-out prompts, every Speed, Balanced, and Quality program sustains positive gains over standard inference and translates FLOPs savings directly into measured wall-clock acceleration (up to $4.48\times$ and $11.53\times$ over Loop~+~LG), with Speed and Quality offering complementary operating points across GenEval and DPG-Bench. For \texttt{RAE} (the DiffusionBench~\cite{leng2026diffusionbench} \texttt{RAE-SigLIP2-B/DDT} 615M adaptation), Appendix~\ref{sec:supp_rae_provenance} records checkpoint provenance and replay settings.

We reran standard inference (Baseline, plus matched $10$-step Baseline) and Train-Free Loop without and with LoopGuidance~\cite{yan2026trainingfree} (Loop w/o LG and Loop + LG) on both Scale-RAE and RAE under the main-paper protocol with frozen weights. Single and Two denote single- and two-object evaluation; Count, Colors, Pos., and C.\ Attr.\ denote counting, colors, position, and color attribution. The frozen Scale-RAE stock LoopGuidance implementation evaluates an additional full reference at every sampling step, including steps without loops. We therefore approximate its $25$-step cost as $56.04+31.58=87.62$\,TFLOPs, and Configuration Search Quality's $10$-step cost as $17.34+12.63=29.97$\,TFLOPs. These totals and dependent FLOPs speedups use rounded constituent costs; measured wall-clock results are unchanged.

\begin{table*}[!htbp]
\centering
\caption{\textbf{\rqhighlight{1}{\papershort{} improves overall compositional scores, held-out generalization, and measured wall-clock speed over both full- and $10$-step no-loop baselines.}} Panel~(a) expands Table~\ref{tab:main_results} with GenEval subtasks, Balanced, and $10$-step no-loop controls; panel~(b) reports development ($320$) and held-out ($1{,}298$) splits, held-out gains versus Baseline, and RTX~5090 latency (batch~$8$ for Scale-RAE, batch~$16$ for RAE). Rankings are within each backbone.}
\label{tab:supp_main_results_balanced}
\begin{subtable}[t]{\textwidth}
\centering
\caption{\textbf{Full-Benchmark GenEval Subtasks, DPG-Bench, and Inference FLOPs.}}
\renewcommand{\arraystretch}{1.04}
\scriptsize
\setlength{\tabcolsep}{2.6pt}
\begin{tabular*}{\textwidth}{@{\extracolsep{\fill}}l l r | c c c c c c | c | c | r c c@{}}
\toprule
\multirow{2}{*}{\textbf{Model}} & \multirow{2}{*}{\textbf{Method}} & \multirow{2}{*}{\textbf{\#step}} & \multicolumn{7}{c|}{\textbf{GenEval (\%) $\uparrow$}} & \textbf{DPG} & \multirow{2}{*}{\textbf{TFLOPs $\downarrow$}} & \textbf{Speedup $\uparrow$} & \textbf{Speedup $\uparrow$} \\
\cmidrule(lr){4-10}
 & & & \textbf{Single} & \textbf{Two} & \textbf{Count} & \textbf{Colors} & \textbf{Pos.} & \textbf{C. Attr.} & \textbf{Overall} & \textbf{(\%) $\uparrow$} &  & \textbf{vs.\ Base} & \textbf{vs.\ w/ LG} \\
\midrule
 & Baseline & 25 & 96.25 & 50.51 & 37.50 & 76.60 & 27.00 & 22.00 & 51.64 & 77.21 & 31.58 & $1.00\times$ & $2.77\times$ \\
 & Baseline ($10$-step) & 10 & 95.00 & 39.39 & 23.75 & 62.77 & 19.00 & 14.00 & 42.32 & 75.66 & \textbf{12.63} & $\boldsymbol{2.50\times}$ & $\boldsymbol{6.94\times}$ \\
 & Loop w/o LG~\cite{yan2026trainingfree} & 25 & 95.00 & 63.64 & 50.00 & 76.60 & \textbf{32.00} & 25.00 & 57.04 & 80.00 & 56.04 & $0.56\times$ & $1.56\times$ \\
 & Loop + LG~\cite{yan2026trainingfree} & 25 & \underline{97.50} & 65.66 & 53.75 & 74.47 & \underline{30.00} & \textbf{30.00} & 58.56 & 79.71 & 87.62 & $0.36\times$ & $1.00\times$ \\
 \rowcolor{gray!12}\cellcolor{white}
 & Ours (Speed) & 10 & \textbf{98.75} & \textbf{70.71} & \underline{60.00} & \textbf{79.79} & 26.00 & \underline{28.00} & \underline{60.54} & \underline{80.19} & \underline{19.56} & \underline{$1.61\times$} & \underline{$4.48\times$} \\
 \rowcolor{gray!12}\cellcolor{white}
 & Ours (Balanced) & 12 & 96.25 & 65.66 & \textbf{61.25} & 75.53 & 27.00 & 24.00 & 58.28 & \textbf{80.41} & 22.71 & $1.39\times$ & $3.86\times$ \\
 \rowcolor{gray!12}\cellcolor{white}\multirow{-7}{*}{\textbf{Scale-RAE}~\cite{tong2026scaling}}
 & Ours (Quality) & 14 & \underline{97.50} & \underline{67.68} & \underline{60.00} & \underline{78.72} & \textbf{32.00} & \textbf{30.00} & \textbf{60.98} & \underline{80.19} & 27.13 & $1.16\times$ & $3.23\times$ \\
\midrule
 & Baseline & 50 & 83.75 & 28.28 & \underline{32.50} & 63.83 & 10.00 & 13.00 & 38.56 & 70.91 & 29.07 & $1.00\times$ & $1.86\times$ \\
 & Baseline ($10$-step) & 10 & 78.75 & 24.24 & 27.50 & 62.77 & 6.00 & 10.00 & 34.88 & 70.69 & \underline{5.81} & \underline{$5.00\times$} & \underline{$9.32\times$} \\
 & Loop w/o LG~\cite{yan2026trainingfree} & 50 & 82.50 & 30.30 & \textbf{33.75} & 60.64 & 7.00 & 19.00 & 38.87 & 72.44 & 39.67 & $0.73\times$ & $1.37\times$ \\
 & Loop + LG~\cite{yan2026trainingfree} & 50 & 91.25 & \underline{41.41} & 30.00 & \textbf{67.02} & 9.00 & 21.00 & 43.28 & \underline{74.68} & 54.20 & $0.54\times$ & $1.00\times$ \\
 \rowcolor{gray!12}\cellcolor{white}
 & Ours (Speed) & 6 & \textbf{96.25} & 39.39 & 30.00 & 64.89 & \underline{11.00} & \underline{25.00} & \underline{44.42} & \textbf{74.96} & \textbf{5.60} & $\boldsymbol{5.19\times}$ & $\boldsymbol{9.68\times}$ \\
 \rowcolor{gray!12}\cellcolor{white}\multirow{-6}{*}{\textbf{RAE}~\cite{leng2026diffusionbench}}
 & Ours (Quality) & 10 & \underline{93.75} & \textbf{42.42} & 27.50 & \underline{65.96} & \textbf{13.00} & \textbf{27.00} & \textbf{44.94} & 74.47 & 9.33 & $3.12\times$ & $5.81\times$ \\
\bottomrule
\end{tabular*}
\end{subtable}
\par\medskip
\begin{subtable}[t]{\textwidth}
\centering
\caption{\textbf{Held-Out Generalization ($1{,}298$ Prompts) and Measured Wall-Clock Latency.} Deltas and wall-clock speedup ratios are computed from unrounded scores and latencies.}
\renewcommand{\arraystretch}{1.04}
\scriptsize
\setlength{\tabcolsep}{2.8pt}
\begin{tabular*}{\textwidth}{@{\extracolsep{\fill}}l l r | c | c | c c | r c@{}}
\toprule
\multirow{2}{*}{\textbf{Model}} & \multirow{2}{*}{\textbf{Method}} & \multirow{2}{*}{\textbf{\#step}} & \textbf{Dev ($320$) $\uparrow$} & \textbf{Held-out ($1{,}298$) $\uparrow$} & \multicolumn{2}{c|}{\textbf{Held-out $\boldsymbol{\Delta}$ vs.\ Base}} & \textbf{Wall $\downarrow$} & \textbf{Wall Speedup $\uparrow$} \\
\cmidrule(lr){4-5}\cmidrule(lr){6-7}
 & & & \textbf{G / D (\%)} & \textbf{G / D (\%)} & \textbf{GenEval (pp)} & \textbf{DPG (pp)} & \textbf{(s/img)} & \textbf{(Base / w/ LG)} \\
\midrule
 & Baseline & 25 & $53.80$ / $77.55$ & $51.14$ / $77.12$ & --- & --- & $0.283$ & $1.00\times$ / $2.77\times$ \\
 & Baseline ($10$-step) & 10 & $45.75$ / $76.68$ & $41.47$ / $75.42$ & $-9.67$ & $-1.71$ & \textbf{0.111} & $\boldsymbol{2.54\times}$ / $\boldsymbol{7.05\times}$ \\
 & Loop w/o LG~\cite{yan2026trainingfree} & 25 & $59.88$ / $79.70$ & $56.35$ / $80.08$ & $+5.21$ & $+2.95$ & $0.498$ & $0.57\times$ / $1.57\times$ \\
 & Loop + LG~\cite{yan2026trainingfree} & 25 & $60.42$ / $80.06$ & $57.90$ / $79.63$ & $+6.76$ & $+2.51$ & $0.784$ & $0.36\times$ / $1.00\times$ \\
 \rowcolor{gray!12}\cellcolor{white}
 & Ours (Speed) & 10 & $64.99$ / $80.66$ & \textbf{59.24} / $80.07$ & $+8.10$ & $+2.95$ & \underline{0.175} & \underline{$1.61\times$} / \underline{$4.48\times$} \\
 \rowcolor{gray!12}\cellcolor{white}
 & Ours (Balanced) & 12 & $63.31$ / $81.55$ & $56.89$ / \underline{80.14} & $+5.75$ & $+3.01$ & $0.203$ & $1.39\times$ / $3.87\times$ \\
 \rowcolor{gray!12}\cellcolor{white}\multirow{-7}{*}{\textbf{Scale-RAE}~\cite{tong2026scaling}}
 & Ours (Quality) & 14 & $69.33$ / $80.23$ & \underline{58.76} / \textbf{80.18} & $+7.62$ & $+3.06$ & $0.239$ & $1.18\times$ / $3.28\times$ \\
\midrule
 & Baseline & 50 & $44.02$ / $71.84$ & $36.78$ / $70.68$ & --- & --- & $0.313$ & $1.00\times$ / $1.88\times$ \\
 & Baseline ($10$-step) & 10 & $36.59$ / $71.69$ & $34.18$ / $70.45$ & $-2.60$ & $-0.23$ & \underline{0.063} & \underline{$4.97\times$} / \underline{$9.35\times$} \\
 & Loop w/o LG~\cite{yan2026trainingfree} & 50 & $42.22$ / $74.08$ & $37.81$ / $72.04$ & $+1.03$ & $+1.35$ & $0.434$ & $0.72\times$ / $1.36\times$ \\
 & Loop + LG~\cite{yan2026trainingfree} & 50 & $45.27$ / $75.42$ & $42.80$ / \underline{74.50} & $+6.01$ & $+3.81$ & $0.588$ & $0.53\times$ / $1.00\times$ \\
 \rowcolor{gray!12}\cellcolor{white}
 & Ours (Speed) & 6 & $50.22$ / $74.47$ & \underline{42.98} / \textbf{75.07} & $+6.19$ & $+4.39$ & \textbf{0.051} & $\boldsymbol{6.13\times}$ / $\boldsymbol{11.53\times}$ \\
 \rowcolor{gray!12}\cellcolor{white}\multirow{-6}{*}{\textbf{RAE}~\cite{leng2026diffusionbench}}
 & Ours (Quality) & 10 & $50.34$ / $75.29$ & \textbf{43.59} / $74.27$ & $+6.81$ & $+3.58$ & $0.085$ & $3.68\times$ / $6.93\times$ \\
\bottomrule
\end{tabular*}
\end{subtable}
\end{table*}

\paragraph{Qualitative comparison settings.}
\label{sec:supp_qualitative_protocol}
Figures~\ref{fig:qualitative} and~\ref{fig:supp_qualitative} compare matched GenEval and DPG-Bench examples on Scale-RAE (1.5B + 2.4B DiT) and RAE (Qwen3-0.6B + DDT). Read the five columns as full-step standard inference ($25$/$50$ steps), $10$-step standard inference, Train-Free Loop without and with LoopGuidance, and our $10$-step programs; compute appears below each heading. Our programs reduce FLOPs by $1.61\times$/$3.12\times$ versus full-step standard inference and approximately $4.48\times$/$5.81\times$ versus Loop + LG. The selected outputs illustrate text rendering, attribute binding, object composition, and color attribution, not the frequency of improvements. Each marked region is enlarged directly from the original image, with the same crop size across all five methods within an example.

\paragraph{Qualitative prompt excerpts.}
The figures shorten the displayed prompt excerpts to emphasize the attributes being compared. The longer excerpts are:
\begin{itemize}
\item \textbf{Text rendering:} ``An old, vibrant red heavy truck with visible signs of wear stands stationary near a weathered stop sign on a street lined with brick facades\ldots''
\item \textbf{Attribute binding:} ``A vibrant yellow rabbit \ldots\ bounds across a meadow of wildflowers, its sizeable, red-framed glasses slipping to the tip of its nose\ldots''
\item \textbf{Object composition:} ``A city scene where a yellow school bus stands on an asphalt road \ldots\ behind the stationary bus, a white van and city buildings stand.''
\item \textbf{Color attribution:} ``a photo of a purple wine glass and a black apple''
\end{itemize}

\begin{figure}[!htbp]
\centering
\input{figs/fig_qualitative_supp}
\caption{\textbf{Additional selected examples illustrate improved attribute binding and object composition with frozen loop programs.} Panels show Scale-RAE (a) and RAE (b), complementing Figure~\ref{fig:qualitative}. Boxes locate the enlarged details below; \textcolor{lpsOurs}{magenta} frames mark ours. Header numbers are TFLOPs per image; parenthesized values are the reported DPG scores ($0$--$1$, higher is better).}
\label{fig:supp_qualitative}
\end{figure}

\FloatBarrier
\subsection{Text-to-Image Diffusion: Models Trained with Loops}
\label{sec:supp_looped_results}

\Cref{tab:supp_looped_dit_full_subtasks} expands \cref{tab:looped_dit_main} with all baseline settings, core-pass counts, GenEval subtasks, and the $20$-step Balanced program. Even when a model is pretrained with recurrent blocks, uniform $K{=}4$ iteration wastes passes across flat mid-trajectory segments while under-resolving sharp early transitions. Combining curvature-warped timestep allocation, dual-stream extrapolation, and bounded late-loop residual reuse lifts every matched-step regime---most sharply under aggressive step budgets (up to $+4.07$\,pp GenEval and $+3.80$\,pp DPG at $14$ steps)---and allows Balanced ($20$ steps, $5.50\times$ FLOPs speedup) and Quality ($25$ steps) to surpass the $100$-step reference on overall GenEval while staying within $0.34$\,pp on DPG-Bench. Diagnostics, program design, and held-out confirmation appear in Appendix~\ref{sec:supp_looped_dit}.

We reran the Looped-DiT~\cite{chng2026looped} baselines using the published inference rule with the stated sampling steps and $K$ core passes per step. Core Passes counts core passes across sampling steps. Full reference denotes the $100$-step $K{=}4$ reference. The complete table ranks all displayed settings together, so its bold and underlined values can differ from the smaller matched-step groups in the main table.

\begin{table*}[!htbp]
\centering
\caption{\textbf{\rqhighlight{1}{\papershort{} improves every matched-step regime and recovers full-reference compositional quality with $4\times$--$7.8\times$ FLOPs speedup.}} This expands Table~\ref{tab:looped_dit_main} with all baseline settings, Balanced, and GenEval subtasks. Rankings cover the full displayed set.}
\label{tab:supp_looped_dit_full_subtasks}
\renewcommand{\arraystretch}{1.10}
\small
\setlength{\tabcolsep}{3pt}
\begin{tabular}{@{}l<{\hspace{3pt}} r c | c c c c c c | c | c | r c@{}}
\toprule
\multirow{2}{*}{\textbf{Method}} & \multirow{2}{*}{\textbf{\#step}} & \textbf{Core} & \multicolumn{7}{c|}{\textbf{GenEval (\%) $\uparrow$}} & \textbf{DPG} & \multirow{2}{*}{\textbf{TFLOPs $\downarrow$}} & \textbf{Speedup $\uparrow$} \\
\cmidrule(lr){4-10}
& & \textbf{Passes} & \textbf{Single} & \textbf{Two} & \textbf{Count} & \textbf{Colors} & \textbf{Pos.} & \textbf{C. Attr.} & \textbf{Overall} & \textbf{(\%) $\uparrow$} &  & \textbf{vs.\ Full} \\
\midrule
Looped-DiT~\cite{chng2026looped} ($K{=}4$) & 100 & 400 & 99.38 & 93.18 & \textbf{71.56} & 92.29 & \underline{81.50} & 70.00 & 84.65 & \textbf{85.34} & 53.18 & $1.00\times$ \\
Looped-DiT~\cite{chng2026looped} ($K{=}1$) & 100 & 100 & 99.38 & \underline{94.19} & 69.69 & \textbf{92.82} & \textbf{83.00} & 67.75 & 84.47 & 84.26 & 28.98 & $1.84\times$ \\
Looped-DiT~\cite{chng2026looped} ($K{=}4$) & 50 & 200 & \underline{99.69} & \underline{94.19} & 70.94 & 92.29 & 79.25 & \underline{72.25} & 84.77 & \underline{85.29} & 26.59 & $2.00\times$ \\
Looped-DiT~\cite{chng2026looped} ($K{=}4$) & 25 & 100 & \textbf{100.00} & 93.69 & 65.94 & \textbf{92.82} & 78.25 & 68.25 & 83.16 & 84.76 & 13.30 & $4.00\times$ \\
Looped-DiT~\cite{chng2026looped} ($K{=}4$) & 20 & 80 & \textbf{100.00} & 92.93 & 65.94 & 90.96 & 78.50 & 65.25 & 82.26 & 84.18 & 10.64 & $5.00\times$ \\
Looped-DiT~\cite{chng2026looped} ($K{=}4$) & 14 & 56 & \underline{99.69} & 89.39 & 63.12 & 86.44 & 76.75 & 60.75 & 79.36 & 81.31 & \underline{7.45} & \underline{$7.14\times$} \\
\midrule
 \rowcolor{gray!12}
Ours (Speed) & 14 & 48 & \textbf{100.00} & 93.43 & 67.81 & \underline{92.55} & 78.00 & 68.75 & 83.43 & 85.11 & \textbf{6.80} & $\boldsymbol{7.82\times}$ \\
 \rowcolor{gray!12}
Ours (Balanced) & 20 & 68 & 99.38 & \textbf{94.44} & 70.31 & 92.02 & 80.00 & \textbf{74.00} & \underline{85.03} & 85.00 & 9.67 & $5.50\times$ \\
 \rowcolor{gray!12}
Ours (Quality) & 25 & 100 & \textbf{100.00} & \textbf{94.44} & \underline{71.25} & 92.29 & \underline{81.50} & 71.00 & \textbf{85.08} & 85.09 & 13.30 & $4.00\times$ \\
\bottomrule
\end{tabular}
\end{table*}

\FloatBarrier
\subsection{Long-Video Consistency: Loop Window, Depth, and Mechanistic Analysis}
\label{sec:supp_longlive10_additional}
\Cref{tab:longlive10_loop_variants} expands the long-video evaluation along two axes: panel~(a) sweeps loop window placement and depth on LongLive~1.0 1.3B across all $100$ RememBench scenes (with all loops restricted to high-noise steps $\{0,1\}$), and panel~(b) isolates the $80$ unseen held-out scenes across LongLive~2.0, LongLive~1.0, and Self-Forcing. The controlled fixed-width sweep in~(a) reveals a clear functional stratification across network depth: shifting a seven-block middle window just one block past network center (from blocks $11$--$17$ to $12$--$18$ of $30$) consistently sharpens semantic and perceptual revisit fidelity at both $K{=}4$ and $K{=}8$ (lifting mean CLIP to $0.9403$ at $K{=}4$ and lowering LPIPS to $0.1334$ at $K{=}8$), whereas an earlier band ($9$--$15$) favors local frame-to-frame smoothness (highest TempSSIM). Once placed in this semantic sweet spot, increasing loop depth ($K{=}4 \to 8$) further tightens perceptual reconstruction at a slight CLIP trade-off. Panel~(b) confirms that these consistency gains transfer robustly to the $80$ unseen scenes across all three backbones, including an independent $20/80$ \papershort{} evaluation on Self-Forcing~1.3B under the unified $379$-frame protocol (blocks $14$--$19$, $K{=}6$; Appendix~\ref{sec:supp_exp_settings}).

\begin{table*}[!htbp]
\centering
\caption{\textbf{\rqhighlight{3}{Window/depth choices trade off long-video consistency, and frozen loop programs generalize to $80$ unseen RememBench scenes.}} Panel~(a) compares LongLive~1.0 1.3B loop windows across all $100$ scenes; panel~(b) reports $80$-scene held-out results for LongLive~2.0, LongLive~1.0, and Self-Forcing. Entries report mean (median); \textbf{bold}/\underline{underlined}: best/second-best in~(a), better per backbone pair in~(b).}
\label{tab:longlive10_loop_variants}
\label{tab:supp_longlive10_additional_all100}
\label{tab:supp_longlive10_additional_configs}
\begin{subtable}[t]{\textwidth}
\centering
\caption{\textbf{LongLive~1.0 1.3B Loop Window and Depth Study (All $100$ Scenes).}}
\small
\setlength{\tabcolsep}{7pt}
\renewcommand{\arraystretch}{1.08}
\begin{tabular}{@{}l c | c c c@{}}
\toprule
\textbf{Window} & $\boldsymbol{K}$ & \textbf{CLIP $\uparrow$} & \textbf{LPIPS $\downarrow$} & \textbf{TempSSIM $\uparrow$} \\
\midrule
Native~\cite{yang2026longlive} & --- & 0.8670 (0.8919) & 0.2609 (0.2591) & 0.9819 (0.9839) \\
$11$--$17$ & 8 & 0.9218 (\underline{0.9526}) & 0.1480 (0.1363) & 0.9869 (0.9903) \\
\midrule
$9$--$15$ & 8 & 0.9218 (0.9407) & 0.1533 (0.1404) & \textbf{0.9890} (0.9894) \\
$11$--$17$ & 4 & 0.9231 (0.9407) & 0.1592 (0.1213) & \underline{0.9876} (0.9888) \\
$12$--$18$ & 4 & \textbf{0.9403} (\textbf{0.9585}) & \underline{0.1387} (\underline{0.1107}) & 0.9875 (\textbf{0.9906}) \\
$12$--$18$ & 8 & \underline{0.9371} (0.9504) & \textbf{0.1334} (\textbf{0.0975}) & 0.9866 (\underline{0.9904}) \\
\bottomrule
\end{tabular}
\end{subtable}
\par\smallskip
\begin{subtable}[t]{\textwidth}
\centering
\caption{\textbf{$80$-Scene Held-Out Results for LongLive~2.0, LongLive~1.0, and Self-Forcing.} Self-Forcing reports an independent $20/80$ \papershort{} evaluation under the unified $379$-frame protocol alongside the $100$-scene comparison in Table~\ref{tab:world_model}.}
\small
\setlength{\tabcolsep}{6pt}
\renewcommand{\arraystretch}{1.08}
\begin{tabular}{@{}l l | c c c@{}}
\toprule
\textbf{Backbone} & \textbf{Method} & \textbf{CLIP $\uparrow$} & \textbf{LPIPS $\downarrow$} & \textbf{TempSSIM $\uparrow$} \\
\midrule
 & Native (no loop) & 0.8551 (0.8947) & 0.3907 (0.4033) & 0.9658 (0.9689) \\
\rowcolor{gray!12}\cellcolor{white}\multirow{-2}{*}{LongLive~2.0 5B~\cite{chen2026longlive2}} & ELP (Ours, $11$--$18$, $K{=}6$, Table~\ref{tab:world_model}) & \textbf{0.9213} (\textbf{0.9563}) & \textbf{0.1577} (\textbf{0.1017}) & \textbf{0.9900} (\textbf{0.9938}) \\
\midrule
 & Native (no loop) & 0.8676 (0.8919) & 0.2604 (0.2556) & 0.9819 (0.9835) \\
\rowcolor{gray!12}\cellcolor{white}\multirow{-2}{*}{LongLive~1.0 1.3B~\cite{yang2026longlive}} & ELP (Ours, $11$--$17$, $K{=}8$, Table~\ref{tab:world_model}) & \textbf{0.9173} (\textbf{0.9432}) & \textbf{0.1556} (\textbf{0.1380}) & \textbf{0.9861} (\textbf{0.9888}) \\
\midrule
 & Native (no loop) & 0.6465 (0.6416) & 0.5086 (0.5075) & 0.9771 (0.9799) \\
\rowcolor{gray!12}\cellcolor{white}\multirow{-2}{*}{Self-Forcing~1.3B~\cite{huang2025selfforcing}} & ELP (Ours, $14$--$19$, $K{=}6$) & \textbf{0.7375} (\textbf{0.7463}) & \textbf{0.3808} (\textbf{0.3765}) & \textbf{0.9788} (\textbf{0.9817}) \\
\bottomrule
\end{tabular}
\end{subtable}
\end{table*}

\paragraph{Additional LongLive~2.0 qualitative comparisons.}
Figure~\ref{fig:supp_longlive_examples} supplements Figure~\ref{fig:teaser}g and Figure~\ref{fig:qualitative}c with three additional RememBench T2V video sequences from the frozen LongLive~2.0~(5B) loop program in Table~\ref{tab:world_model} (block-group / windowwise recurrence with loop count $K{=}6$, blocks $11$--$18$, denoising steps $\{0,1,2\}$). Across these selected departure-to-revisit examples ($3.6\,\mathrm{s}$ to $15.8\,\mathrm{s}$), the baseline drifts or corrupts scene structure, whereas the frozen loop program closes each container mid-sequence and restores its original contents: in~(a), the baseline melts the hinged bread-maker lid into a deformed double slab while our program restores the loaf; in~(b), the baseline hallucinates a reflective screen inside the milk crate while our program closes the lid and recovers the newspapers; and in~(c), the baseline embeds dark arc artifacts into the cracker barrel and shifts viewpoint while our program seals cleanly and restores the crackers. As with other qualitative visualizations, these examples illustrate revisit recovery rather than improvement frequency.

\begin{figure}[!htbp]
\centering
\resizebox{\textwidth}{!}{\input{figs/fig_longlive_supp}}
\caption{\textbf{\rqhighlight{3}{Frozen LongLive~2.0~(5B) loop programs preserve container geometry and contents on revisit where the baseline drifts or hallucinates.}} Matched RememBench T2V frames compare the baseline and our Table~\ref{tab:world_model} program from departure ($3.6\,\mathrm{s}$, \textcolor[HTML]{0076C6}{blue}) to revisit ($15.8\,\mathrm{s}$, \textcolor{lpsReferenceDark}{slate} vs.\ \textcolor{lpsOurs}{magenta}) on selected examples: (a)~bread maker, (b)~milk crate, and (c)~cracker barrel.}
\label{fig:supp_longlive_examples}
\end{figure}

\paragraph{Middle-band recurrence and cache updates.}
Tables~\ref{tab:world_model}, \ref{tab:longlive10_loop_variants}, and~\ref{tab:supp_searched_solutions} show that independent LongLive~1.0 and LongLive~2.0 searches select contiguous middle-band (windowwise) Euler loops: blocks $11$--$17$ or $11$--$18$ of $30$, with updates $\Delta\mathbf{x}^{(r)}{=}\tfrac{1}{K}(W(\mathbf{x}^{(r)}){-}\mathbf{x}^{(r)})$ and causal key--value (KV) writes deferred to the final pass. Baseline diagnostics show negative input--residual alignment at early blocks (e.g., LongLive~2.0 block~$1$) and residual spikes at the terminal block~$29$, motivating exploration of middle bands. On LongLive~2.0 held-out scenes (Table~\ref{tab:longlive10_loop_variants}(b)), the frozen windowwise $K{=}6$ program reduces LPIPS by $59.6\%$ relative to Native ($0.3907 \to 0.1577$). Final-pass KV writes keep historical context fixed during refinement and prevent intermediate passes from committing states for future chunks.

\paragraph{Interactions between active steps and loop structure.}
The selected active steps correspond to high-noise portions of each schedule (Table~\ref{tab:supp_repro_details}): LongLive~1.0 uses steps $\{0,1\}$ of $[1000,750,500,250]$, whereas LongLive~2.0 uses $\{0,1,2\}$ of its shift-$5$ UniPC schedule $[999,937,833,624]$, whose step~$2$ remains at $t{=}833$. In LongLive~2.0 Round~$2$, while step~$0$ was excluded, raising $K$ or extending the window to start at block~$11$ degraded CLIP. After step~$0$ was activated, the block-$11$ boundary produced a further gain ($\Delta\mathrm{HV}{=}+0.036$). In LongLive~1.0, blocks $1$--$8$ initially led CLIP but saturated at higher $K$; the retained middle band ($11$--$17$) overtook it at $K{=}8$. These trajectories suggest interactions among active steps, window placement, and depth.

\paragraph{Gains on failure-prone scenes.}
Grouping the $100$ RememBench scenes by baseline-drift quartile shows that the hardest quartile receives the largest improvements: LPIPS falls by $63.0\%$ ($+0.158$ CLIP) on LongLive~2.0 and $58.9\%$ ($+0.127$ CLIP) on LongLive~1.0. Absolute CLIP and LPIPS gains are largest in the highest-drift quartile. Severe perceptual failures ($\mathrm{LPIPS}{>}0.40$) drop from $48$ to $5$ scenes on LongLive~2.0 ($41$ to $4$ on the $80$ held-out scenes) and from $12$ to $2$ on LongLive~1.0. Semantic failures ($\mathrm{CLIP}{<}0.80$) fall by more than half on both models. These observations locate the gains beyond the averages in Table~\ref{tab:world_model}; Table~\ref{tab:longlive10_loop_variants} retains the remaining trade-offs among CLIP, LPIPS, and TempSSIM as window and depth vary.

\FloatBarrier
\subsection{Short-Video Diffusion: Wan2.1-1.3B}
\label{sec:supp_video_results}

Table~\ref{tab:supp_video_vbench} reports the complete Wan2.1-1.3B short-video results for frozen programs searched separately from the autoregressive RememBench study, alongside our reruns of the native $50$- and $30$-step baselines under the local $256$-video VBench protocol (Appendix~\ref{sec:supp_local_protocols}). Panel~(a) presents the full $256$-video Quality, Semantic, and Overall scores together with temporal and visual sub-dimensions across all four selected programs (Quality names the Overall-selected program, while Quality-alt. is a second quality-focused representative). Panel~(b) separates the $48$-video development split from the $208$ videos outside the final development panel (including $16$ seen in earlier evaluations), the $192$ videos strictly unseen by prior search pools, and measured per-video wall-clock generation latency.

Table~\ref{tab:supp_video_vbench} reveals a clean mechanistic split between the two regimes uncovered on Wan2.1-1.3B. In the accelerated regime ($26$ steps), restricting loops to conditional cross-attention on middle blocks ($10$--$13$) while combining step reduction with interval guidance reuse cuts wall-clock generation time by more than half ($2.24\times$ faster than the $50$-step baseline and faster even than the $30$-step native control); notably, these streamlined trajectories improve every temporal-consistency axis (subject, background, flicker, and motion smoothness), indicating that fewer, smoother cross-attention-stabilized updates suppress high-frequency frame jitter at the expense of fine semantic detail. Conversely, in the full-$50$-step quality regime, multi-window spacetime curvature-lookahead looping targets semantic grounding---driving large Scene gains ($71.47$ vs.\ $52.17$) and preserving a $+0.88$\,pp Semantic advantage on the $208$ mixed-exposure videos---yet because VBench partitions prompts across $16$ heterogeneous dimensions (leaving only $4$--$5$ videos per semantic dimension in the $48$-video development panel), overall aggregates sit near parity on the Mixed $208$ and Unseen $192$ splits. The speedups and temporal gains belong to Speed/Balanced, while semantic gains belong to Quality; the mixed-exposure $208$-video split is not independent confirmation. FLOPs speedup uses the $50$-step Baseline ($28{,}300.2$\,TFLOPs), and VBench~\cite{huang2024vbench} sub-dimension abbreviations denote subject consistency, background consistency, temporal flickering, motion smoothness, aesthetic quality, and temporal style.

\begin{table*}[!htbp]
\centering
\caption{\textbf{\rqhighlight{3}{Wan2.1-1.3B programs offer distinct speed and quality trade-offs.}} Panel~(a) expands VBench aggregates and sub-dimensions on all $256$ videos; panel~(b) separates Development ($48$), Mixed ($208$, including $16$ previously seen videos), and Unseen ($192$) splits alongside measured generation latency (s/video). \textbf{Bold}/\underline{underlined}: best/second-best.}
\label{tab:supp_video_vbench}
\label{tab:video_vbench}
\label{tab:video_remembench}
\begin{subtable}[t]{\textwidth}
\centering
\caption{\textbf{Full $256$-Video VBench Sub-Dimensions and Inference FLOPs.}}
\scriptsize
\setlength{\tabcolsep}{2.8pt}
\renewcommand{\arraystretch}{1.08}
\begin{tabular*}{\textwidth}{@{\extracolsep{\fill}}l r | c c c c c c c | c c c | r c@{}}
\toprule
\multirow{2}{*}{\textbf{Method}} & \multirow{2}{*}{\textbf{\#step}} & \multicolumn{7}{c|}{\textbf{VBench Sub-Dimensions (\%) $\uparrow$}} & \multicolumn{3}{c|}{\textbf{VBench (\%) $\uparrow$}} & \multirow{2}{*}{\textbf{TFLOPs $\downarrow$}} & \textbf{Speedup $\uparrow$} \\
\cmidrule(lr){3-9}\cmidrule(lr){10-12}
& & \shortstack{\textbf{Subj.}\\\textbf{Cons.}} & \shortstack{\textbf{Bg.}\\\textbf{Cons.}} & \shortstack{\textbf{Temp.}\\\textbf{Flick.}} & \shortstack{\textbf{Motion}\\\textbf{Smooth.}} & \shortstack{\textbf{Aesth.}\\\textbf{Quality}} & \textbf{Scene} & \shortstack{\textbf{Temp.}\\\textbf{Style}} & \textbf{Quality} & \textbf{Semantic} & \textbf{Overall} &  & \textbf{vs.\ Base} \\
\midrule
Wan2.1~\cite{wan2025wan} & 50 & 94.20 & 98.09 & 99.53 & 98.52 & \underline{67.82} & 52.17 & 26.42 & \textbf{85.39} & 83.04 & 84.92 & 28{,}300.2 & $1.00\times$ \\
Wan2.1~\cite{wan2025wan} & 30 & 94.48 & 98.10 & \underline{99.57} & 98.55 & 67.81 & 57.07 & 26.54 & \underline{85.33} & 80.54 & 84.37 & 16{,}980.1 & $1.67\times$ \\
\midrule
 \rowcolor{gray!12}
Ours (Speed) & 26 & \underline{95.46} & \textbf{98.60} & \textbf{99.63} & \textbf{98.68} & 67.11 & 55.43 & \underline{26.84} & 84.85 & 80.32 & 83.94 & \textbf{11{,}916.1} & $\boldsymbol{2.37\times}$ \\
 \rowcolor{gray!12}
Ours (Balanced) & 26 & \textbf{95.54} & \underline{98.57} & \textbf{99.63} & \textbf{98.68} & 67.24 & 65.22 & \textbf{26.87} & 84.90 & 82.03 & 84.33 & \underline{12{,}765.1} & \underline{$2.22\times$} \\
 \rowcolor{gray!12}
Ours (Quality-alt.) & 50 & 94.14 & 97.91 & 99.53 & 98.56 & \textbf{68.10} & \underline{65.76} & 26.55 & 85.32 & \underline{83.57} & \underline{84.97} & 30{,}903.6 & $0.92\times$ \\
 \rowcolor{gray!12}
Ours (Quality) & 50 & 94.01 & 98.00 & 99.53 & \underline{98.57} & 67.71 & \textbf{71.47} & 26.56 & 85.25 & \textbf{84.61} & \textbf{85.12} & 30{,}903.6 & $0.92\times$ \\
\bottomrule
\end{tabular*}
\end{subtable}
\par\medskip
\begin{subtable}[t]{\textwidth}
\centering
\caption{\textbf{Split Breakdown (Dev $48$ / Mixed $208$ / Unseen $192$ / Full $256$) and Measured Wall-Clock Latency.}}
\scriptsize
\setlength{\tabcolsep}{3.5pt}
\renewcommand{\arraystretch}{1.08}
\begin{tabular*}{\textwidth}{@{\extracolsep{\fill}}l r | c c c | c c c | c | c | r c@{}}
\toprule
\multirow{2}{*}{\textbf{Method}} & \multirow{2}{*}{\textbf{\#step}} & \multicolumn{3}{c|}{\textbf{Dev $48$ (\%) $\uparrow$}} & \multicolumn{3}{c|}{\textbf{Mixed $208$ (\%) $\uparrow$}} & \textbf{Unseen $192$} & \textbf{Full $256$} & \textbf{Wall $\downarrow$} & \textbf{Wall $\uparrow$} \\
\cmidrule(lr){3-5}\cmidrule(lr){6-8}
 & & \textbf{Qual.} & \textbf{Sem.} & \textbf{Ov.} & \textbf{Qual.} & \textbf{Sem.} & \textbf{Ov.} & \textbf{Ov.\ (\%) $\uparrow$} & \textbf{Ov.\ (\%) $\uparrow$} & \textbf{(s/vid)} & \textbf{Speedup} \\
\midrule
Wan2.1~\cite{wan2025wan} & 50 & 85.71 & 83.00 & 85.17 & \textbf{85.31} & \underline{83.05} & \textbf{84.86} & \underline{84.92} & 84.92 & $117.4$ & $1.00\times$ \\
Wan2.1~\cite{wan2025wan} & 30 & 85.70 & 74.51 & 83.46 & \underline{85.23} & 81.80 & 84.55 & 84.83 & 84.37 & $72.4$ & $1.62\times$ \\
\midrule
 \rowcolor{gray!12}
Ours (Speed) & 26 & 86.19 & 86.44 & 86.24 & 84.51 & 78.94 & 83.39 & 83.46 & 83.94 & \textbf{52.4} & $\boldsymbol{2.24\times}$ \\
 \rowcolor{gray!12}
Ours (Balanced) & 26 & \textbf{86.35} & \textbf{89.14} & \textbf{86.91} & 84.54 & 80.44 & 83.72 & 83.80 & 84.33 & \underline{55.7} & \underline{$2.11\times$} \\
 \rowcolor{gray!12}
Ours (Quality-alt.) & 50 & \underline{86.30} & 86.72 & 86.38 & 85.08 & 82.89 & 84.64 & 84.90 & \underline{84.97} & $129.2$ & $0.91\times$ \\
 \rowcolor{gray!12}
Ours (Quality) & 50 & 86.11 & \underline{87.78} & \underline{86.44} & 85.03 & \textbf{83.93} & \underline{84.81} & \textbf{84.94} & \textbf{85.12} & $129.4$ & $0.91\times$ \\
\bottomrule
\end{tabular*}
\end{subtable}
\end{table*}

\FloatBarrier
\input{sec/appendix_dory}

\FloatBarrier
\subsection{Text Reasoning: Models Trained without Loops (Qwen3-4B)}
\label{sec:supp_text_representatives}

Table~\ref{tab:supp_llm_representatives} expands Table~\ref{tab:llm_reasoning} with $3{,}316$-question held-out aggregates alongside the full $4{,}145$-question suite. Contrasting Qwen3-4B with Dory1.0-4B (Section~\ref{sec:supp_dory}) clarifies how pretraining shapes test-time loop headroom in language models: without recurrent pretraining, Qwen3-4B's frozen residual blocks operate within a tighter multi-pass stability envelope, limiting how aggressively hidden states can be iterated. Even so, pairing a non-overlapping dual-window schedule with third-order RK3 updates and read-only intermediate passes (Table~\ref{tab:supp_searched_solutions}) delivers consistent held-out gains over Non-looped inference ($+1.42$\,pp Micro Acc, $+1.56$\,pp Macro Domain), concentrated on knowledge-intensive multi-step questions (GPQA-Main and MMLU-STEM). On unseen questions, the program matches or narrowly edges past the strong Fixed Loop~\cite{chen2026trainingfreelooped} baseline across key aggregates (trailing slightly on Micro Acc Norm), with tighter margins than on development prompts. Because \papershort{} simultaneously expands Fixed Loop's single middle Euler window ($15$--$18$) into a dual-window RK3 program ($[14]{+}[15..18]$ and $25$--$28$), this gain reflects the combined edit; controlled evidence for window shifting alone comes from the LongLive~1.0 sweep (Appendices~\ref{sec:supp_longlive10_additional} and~\ref{sec:supp_programs}). All methods are evaluated identically on the same $4{,}145$-question split (Appendix~\ref{sec:supp_local_protocols}).

\begin{table}[!htbp]
\centering
\caption{\textbf{The frozen Qwen3-4B program transfers held-out gains over Non-looped inference and matches or improves upon Fixed Loop across key aggregates.} \papershort{} (Ours) matches the single task-balanced (Macro) program column in Table~\ref{tab:llm_reasoning}. Full covers $4{,}145$ questions ($829$ dev + $3{,}316$ held-out). \textbf{Bold}/\underline{underlined}: best/second-best within each row.}
\label{tab:supp_llm_representatives}
\small
\setlength{\tabcolsep}{7.5pt}
\renewcommand{\arraystretch}{1.12}
\begin{tabular}{@{}l | c c >{\columncolor{gray!12}[\tabcolsep][4pt]}c@{\hspace{4pt}}}
\toprule
\textbf{Metric (\%) $\uparrow$} & \shortstack{\textbf{Non-}\\\textbf{looped}~\cite{yang2025qwen3}} & \shortstack{\textbf{Fixed}\\\textbf{Loop}~\cite{chen2026trainingfreelooped}} & \shortstack{\textbf{\papershort{}}\\\textbf{(Ours)}} \\
\midrule
\multicolumn{4}{@{}l}{\textit{Individual benchmarks (Full, $4{,}145$ questions)}} \\
MMLU-STEM Acc & 62.43 & \underline{64.20} & \textbf{64.72} \\
GPQA-Main Acc & 31.92 & \underline{33.26} & \textbf{34.82} \\
ARC Acc & \underline{50.60} & \textbf{51.71} & \textbf{51.71} \\
ARC Acc Norm & 54.18 & \textbf{54.95} & \underline{54.61} \\
SciQ Acc & 95.70 & \underline{96.20} & \textbf{96.50} \\
\midrule
\multicolumn{4}{@{}l}{\textit{Full-benchmark aggregates ($4{,}145$ questions)}} \\
Micro Acc & 63.81 & \underline{65.04} & \textbf{65.48} \\
Micro Acc Norm & 64.27 & \underline{65.72} & \textbf{65.91} \\
Macro Group & 60.16 & \underline{61.34} & \textbf{61.94} \\
Macro Domain & 58.37 & \underline{59.60} & \textbf{60.36} \\
\midrule
\multicolumn{4}{@{}l}{\textit{Held-out aggregates ($3{,}316$ unseen questions)}} \\
Micro Acc & 63.93 & \underline{65.26} & \textbf{65.35} \\
Micro Acc Norm & 64.35 & \textbf{65.77} & \underline{65.65} \\
Macro Group & \underline{60.24} & \textbf{61.60} & \textbf{61.60} \\
Macro Domain & 58.46 & \underline{59.81} & \textbf{60.02} \\
\bottomrule
\end{tabular}
\end{table}
