# Supplementary material for: Evolving Loop Programs: Discovering How Frozen Transformers Should Loop
Source: arXiv:2611.41108 source file (2026-12-03)
Supplement: Supplementary file 4 [file appendix_dory.tex]

\subsection{Text Reasoning: Models Trained with Loops (Dory1.0-4B)}
\label{sec:supp_dory}

Analogous to Looped-DiT-B32~\cite{chng2026looped} in image generation, we also evaluate \papershort{} on Dory1.0-4B~\citesupp{fishman2026dory}, an open-weight $4$B language model pretrained with elastic recurrent depth over a weight-tied recurrent block. All pretrained weights remain frozen while offline search discovers inference-time loop programs modifying recurrent depth, inter-loop state transitions, and KV-cache reuse. Each evaluation below reports complete benchmark scores alongside unseen held-out confirmation splits.

\paragraph{Open-ended generative reasoning, coding, and instruction following.}
\label{sec:supp_dory_gen}

We first evaluate open-ended reasoning, instruction following, and coding across IFBench~\citesupp{pyatkin2025ifbench}, GPQA Diamond~\cite{rein2024gpqa}, and SciCode~\citesupp{tian2024scicode}, averaging eight stochastic runs per prompt on both the full benchmarks and the unseen $80\%$ held-out split (Table~\ref{tab:supp_dory_gen}). Because Dory1.0-4B operates on a normalized hypersphere, Euclidean shortcuts distort state norms, whereas applying bounded geodesic extrapolation after just two recurrent passes ($K{=}2$) captures much of the representational progress of deeper iteration at zero extra core passes. Consequently, both $K{=}2$ programs outperform native $K{=}2$ and even native $K{=}4$ on full and held-out averages while cutting FLOPs and wall-clock time by roughly $1.7\times$ relative to native $K{=}4$. Comparing KV-cache policies reveals a second principle: committing only the \emph{converged last-loop} KV state beats per-loop caching across every benchmark on both splits (notably $+1.74$\,pp over native $K{=}2$ on held-out GPQA Diamond), showing that consolidated recurrent memory improves reasoning accuracy rather than trading accuracy for efficiency, whereas per-loop KV retains native-$K{=}2$ wall-clock speed ($1.00\times$) at minimal FLOPs.

\begin{table*}[!htbp]
\centering
\caption{\textbf{\rqhighlight{4}{At $K{=}2$-level compute, both \papershort{} programs improve the three-benchmark mean over native $K{=}2$ and $K{=}4$ on full and held-out evaluations.}} Means across eight runs per prompt on the full benchmarks ($300$ IFBench, $198$ GPQA-D, $65$ SciCode) and the unseen $80\%$ held-out split ($240$, $158$, and $52$ tasks); GPQA-D denotes GPQA Diamond. Speedups use ratios of full-set means relative to native $K{=}2$ and $K{=}4$. Gray shading: ours; \textbf{bold}/\underline{underlined}: best/second-best per column (ties bolded only).}
\label{tab:supp_dory_gen}
\scriptsize
\setlength{\tabcolsep}{1.8pt}
\renewcommand{\arraystretch}{1.15}
\begin{tabular*}{\textwidth}{@{\extracolsep{\fill}}l | c c c c | c c c c | r c c@{}}
\toprule
\multirow{2}{*}{\textbf{Method}} & \multicolumn{4}{c|}{\textbf{Full Benchmarks (\%) $\uparrow$}} & \multicolumn{4}{c|}{\textbf{Held-out ($\mathbf{80\%}$) (\%) $\uparrow$}} & \multirow{2}{*}{\shortstack{\textbf{Total}\\\textbf{TFLOPs $\downarrow$}}} & \multirow{2}{*}{\shortstack{\textbf{Wall Speedup}\\($\boldsymbol{K{=}2}$ \textbf{/} $\boldsymbol{K{=}4}$) $\boldsymbol{\uparrow}$}} & \multirow{2}{*}{\shortstack{\textbf{FLOPs Speedup}\\($\boldsymbol{K{=}2}$ \textbf{/} $\boldsymbol{K{=}4}$) $\boldsymbol{\uparrow}$}} \\
\cmidrule(lr){2-5}\cmidrule(lr){6-9}
 & \textbf{IFBench} & \textbf{GPQA-D} & \textbf{SciCode} & \textbf{Avg.} & \textbf{IFBench} & \textbf{GPQA-D} & \textbf{SciCode} & \textbf{Avg.} & & & \\
\midrule
Native ($K{=}2$, per-loop KV) & 78.48 & 70.39 & 33.90 & 60.92 & \underline{79.30} & 70.57 & \underline{35.61} & 61.82 & 96{,}300 & $\boldsymbol{1.00\times}$ / $\boldsymbol{1.72\times}$ & $1.00\times$ / $1.67\times$ \\
Native ($K{=}4$, per-loop KV) & 78.71 & 71.02 & 33.81 & 61.18 & 79.27 & 71.44 & 34.90 & 61.87 & 161{,}198 & $0.58\times$ / $1.00\times$ & $0.60\times$ / $1.00\times$ \\
\midrule
\rowcolor{gray!12}
ELP (Ours, $K{=}2$, last-loop KV) & \textbf{78.94} & \textbf{71.72} & \textbf{34.07} & \textbf{61.58} & \textbf{79.48} & \textbf{72.31} & \textbf{35.71} & \textbf{62.50} & \underline{95{,}719} & $0.96\times$ / $1.65\times$ & $\boldsymbol{1.01\times}$ / \underline{$1.68\times$} \\
\rowcolor{gray!12}
ELP (Ours, $K{=}2$, per-loop KV) & \underline{78.88} & \underline{71.53} & \underline{33.94} & \underline{61.45} & 79.06 & \underline{72.15} & 35.06 & \underline{62.09} & \textbf{95{,}223} & $\boldsymbol{1.00\times}$ / $\boldsymbol{1.72\times}$ & $\boldsymbol{1.01\times}$ / $\boldsymbol{1.69\times}$ \\
\bottomrule
\end{tabular*}
\end{table*}

\paragraph{Multiple-choice STEM reasoning.}
\label{sec:supp_dory_stem}

Table~\ref{tab:supp_dory_stem4145} next evaluates matched recurrent depths ($K{\in}\{2,3,4\}$) under the $4{,}145$-question zero-shot STEM suite used for Qwen3-4B~\cite{yang2025qwen3} (Appendix~\ref{sec:supp_local_protocols}; ARC~N., M.~Norm, M.~Grp, and M.~Dom abbreviate normalized ARC, Micro Acc Norm, Macro Group, and Macro Domain). Even in a language model pretrained with elastic recurrence, uniform native iteration under-utilizes each pass: tailoring state-transition dynamics to the recurrent manifold unlocks consistent gains across every depth. At $K{=}2$, span-based recurrence cuts per-token compute by $1.17\times$ while lifting held-out Macro Domain accuracy, led by harder multi-step reasoning (GPQA-Main $+1.56$\,pp). At $K{=}3$ and $K{=}4$, geometry-aware transitions---spherical velocity extrapolation at $K{=}3$ and annealed input injection with depth-wise continuation at $K{=}4$---improve every individual benchmark and held-out aggregate at identical compute. Most tellingly, our $K{=}3$ program already surpasses native $K{=}4$ across both Micro and held-out Macro aggregates ($60.68\%$ vs.\ $60.29\%$ Micro Acc), demonstrating that well-matched state dynamics can directly substitute for extra recurrent depth.

\begin{table*}[!htbp]
\centering
\caption{\textbf{\rqhighlight{4}{\papershort{} improves matched-$K$ STEM accuracy--compute trade-offs on Dory1.0-4B.}} Held-out reports Macro Group / Macro Domain on the $3{,}316$ unseen questions. Speedup reports per-token GFLOPs speedup vs.\ each matched native-$K$ baseline. Gray shading: ours; \textbf{bold}: better within each matched-$K$ pair (ties unbolded).}
\label{tab:supp_dory_stem4145}
\scriptsize
\setlength{\tabcolsep}{2.4pt}
\renewcommand{\arraystretch}{1.15}
\begin{tabular*}{\textwidth}{@{\extracolsep{\fill}}l l | r c | c c c c c | c c c c | c@{}}
\toprule
\multirow{2}{*}{\textbf{Setting}} & \multirow{2}{*}{\textbf{Method}} & \multirow{2}{*}{\shortstack{\textbf{GFLOPs}\\\textbf{/ tok $\downarrow$}}} & \multirow{2}{*}{\shortstack{\textbf{Speedup}\\\textbf{(vs.\ $K$) $\uparrow$}}} & \multicolumn{5}{c|}{\textbf{Individual Benchmarks (\%) $\uparrow$}} & \multicolumn{4}{c|}{\textbf{Aggregates (\%) $\uparrow$}} & \multirow{2}{*}{\shortstack{\textbf{Held-out}\\\textbf{M.\ Grp / M.\ Dom $\uparrow$}}} \\
\cmidrule(lr){5-9}\cmidrule(lr){10-13}
 & & & & \textbf{MMLU} & \textbf{GPQA} & \textbf{ARC} & \textbf{ARC N.} & \textbf{SciQ} & \textbf{Micro} & \textbf{M.\ Norm} & \textbf{M.\ Grp} & \textbf{M.\ Dom} & \\
\midrule
 & Native & 11.03 & $1.00\times$ & 54.69 & 28.57 & \textbf{47.78} & \textbf{49.66} & 95.00 & 59.64 & \textbf{60.14} & 56.51 & 51.98 & 56.86 / 52.53 \\
\rowcolor{gray!12}
\cellcolor{white}\multirow{-2}{*}{\shortstack[l]{Matched\\$K{=}2$}} & ELP (Ours) & \textbf{9.45} & $\boldsymbol{1.17\times}$ & \textbf{55.02} & \textbf{30.13} & 46.76 & 48.21 & \textbf{95.20} & \textbf{59.69} & 60.07 & \textbf{56.78} & \textbf{52.93} & \textbf{56.95} / \textbf{53.27} \\
\midrule
 & Native & 14.74 & $1.00\times$ & 55.02 & 28.79 & 47.95 & 49.83 & 94.90 & 59.81 & 60.29 & 56.67 & 52.15 & 57.18 / 52.85 \\
\rowcolor{gray!12}
\cellcolor{white}\multirow{-2}{*}{\shortstack[l]{Matched\\$K{=}3$}} & ELP (Ours) & 14.74 & $1.00\times$ & \textbf{55.67} & \textbf{30.13} & \textbf{49.32} & \textbf{50.85} & \textbf{95.30} & \textbf{60.68} & \textbf{60.97} & \textbf{57.61} & \textbf{53.05} & \textbf{57.93} / \textbf{53.45} \\
\midrule
 & Native & 18.44 & $1.00\times$ & 55.54 & 29.69 & 48.89 & 49.91 & 94.60 & 60.29 & 60.68 & 57.18 & 53.02 & 57.50 / 53.43 \\
\rowcolor{gray!12}
\cellcolor{white}\multirow{-2}{*}{\shortstack[l]{Matched\\$K{=}4$}} & ELP (Ours) & 18.44 & $1.00\times$ & \textbf{56.07} & \textbf{30.80} & \textbf{49.49} & \textbf{50.51} & \textbf{95.10} & \textbf{60.89} & \textbf{61.21} & \textbf{57.86} & \textbf{53.96} & \textbf{58.24} / \textbf{54.45} \\
\bottomrule
\end{tabular*}
\end{table*}
