# Supplementary material for: Evolving Loop Programs: Discovering How Frozen Transformers Should Loop
Source: arXiv:2611.41108 source file (2026-12-03)
Supplement: Supplementary file 5 [file appendix_evaluation_details.tex]

\paragraph{Evaluation protocols.}
Table~\ref{tab:supp_evaluation_protocols} separates the evaluated datasets from their subset-selection rules. Table~\ref{tab:supp_evaluator_implementations} records evaluator versions and numerical settings, and Table~\ref{tab:supp_reasoning_subsets} gives the subject-level counts for the STEM suite. Development subsets are used during search; the evaluation scope reported for each experiment is specified in Table~\ref{tab:supp_exp_settings}.

\begingroup
\small
\setlength{\tabcolsep}{4pt}
\renewcommand{\arraystretch}{1.15}
\par\medskip\noindent
\begin{minipage}{\linewidth}
\centering
\small
\captionof{table}{\textbf{Evaluation protocols separate benchmark coverage from development-subset selection.} Counts refer to prompts, questions, or videos as indicated.}\label{tab:supp_evaluation_protocols}
\begin{tabular}{@{}>{\raggedright\arraybackslash}p{0.20\linewidth} >{\raggedright\arraybackslash}p{0.30\linewidth} >{\raggedright\arraybackslash}p{0.46\linewidth}@{}}
\toprule
\textbf{Evaluation} & \textbf{Dataset and size} & \textbf{Scoring or subset selection} \\
\midrule
GenEval & 553 prompts & All prompts scored. \\
\addlinespace[3pt]
DPG-Bench & 1,065 prompts & All prompts scored. \\
\addlinespace[3pt]
Qwen3-4B STEM & 4,145 questions; 829 development & Zero-shot log-likelihood evaluation; stratified $20\%$ development subset with baseline-informed calibration (\texttt{seed=1234}); no candidate scores used. \\
\addlinespace[3pt]
Dory1.0-4B STEM & Same 4,145-question suite & Reuses the STEM benchmarks listed in Table~\ref{tab:supp_reasoning_subsets}. \\
\addlinespace[3pt]
Dory1.0-4B generation & IFBench~\citesupp{pyatkin2025ifbench}, GPQA Diamond~\cite{rein2024gpqa}, SciCode~\citesupp{tian2024scicode} & Open-ended generation evaluation. \\
\addlinespace[3pt]
RememBench & \texttt{t2v/test} & Departure/revisit frames $86$/$378$; CLIP features, LPIPS, and TempSSIM. \\
\addlinespace[3pt]
MemFlow $60$\,s & 100 six-prompt $60$\,s narratives; 20 stratified dev, 80 held-out & VBench-Long (Quality, Consistency, Aesthetic, Dynamic Degree) and six per-$10$\,s CLIP ViT-L/14 intervals~\citesupp{ji2025memflow}. \\
\addlinespace[3pt]
VBench-1.0 & 256 videos; 48 development & Extended prompts sampled from a 946-prompt pool with \texttt{selection\_seed=42}. See the VBench subset explanation. \\
\bottomrule
\end{tabular}
\end{minipage}
\par\medskip
\endgroup

\paragraph{Aggregation.}
\textit{Macro Domain} is the unweighted mean accuracy across $15$ domains: the ten MMLU Hard-STEM subjects, SciQ, ARC-Challenge, and the three GPQA domains. This differs from the four-benchmark mean described above.

\paragraph{VBench subset construction.}
The $48$-video development panel is selected from a $64$-video, $50$-step baseline pool within the $256$-video evaluation set. The $208$ videos outside the final panel ($256-48$) comprise $16$ previously agent-visible videos and $192$ candidate-unseen videos ($256-64$). Thus the $208$-video split is a mixed-exposure validation set, not wholly independent held-out confirmation.

\begingroup
\small
\setlength{\tabcolsep}{4pt}
\renewcommand{\arraystretch}{1.15}
\def\UrlBreaks{\do\/\do\_\do\-\do\.\do\:\do\,\do\=}
\par\medskip\noindent
\begin{minipage}{\linewidth}
\centering
\small
\captionof{table}{\textbf{Evaluator identities and numerical settings are fixed for reproducible scoring.} Dataset revisions and scorer commits are listed separately.}\label{tab:supp_evaluator_implementations}
\begin{tabular}{@{}>{\raggedright\arraybackslash}p{0.17\linewidth} >{\raggedright\arraybackslash}p{0.35\linewidth} >{\raggedright\arraybackslash}p{0.44\linewidth}@{}}
\toprule
\textbf{Evaluator} & \textbf{Implementation or checkpoint} & \textbf{Version and numerical settings} \\
\midrule
GenEval & \texttt{mmdetection 2.28.2}; Mask2Former Swin-S; OpenCLIP ViT-L/14\newline Checkpoint: \nolinkurl{timm/vit_large_patch14_clip_224.openai} & FP32.\newline Repository: \nolinkurl{djghosh13/geneval}\newline Commit: \texttt{af4902f2}. \\
\addlinespace[4pt]
DPG-Bench & mPLUG VQA & Crop resolutions: $224$/$256$/$512$.\newline Repository: \nolinkurl{TencentQQGYLab/ELLA}\newline Commit: \texttt{3c228f1d}. \\
\addlinespace[4pt]
Qwen3-4B STEM & \texttt{lm\_eval 0.4.11} & \texttt{apply\_chat\_template=False}. \\
\addlinespace[4pt]
RememBench data & \nolinkurl{mosaichunk/RememBench}\newline Split: \texttt{t2v/test} & Dataset revision:\newline \nolinkurl{cdeabf0fce9c075876a903a1d5234483ad677fd5}. \\
\addlinespace[4pt]
RememBench scoring & MosaiChunk \texttt{ClipFeatures};\newline \nolinkurl{LPIPS(net="alex", version="0.1")};\newline \nolinkurl{score\_tempssim.\_win()} & Scorer commit: \texttt{0eafcb91}.\newline TempSSIM: \texttt{allow\_tf32=False}. \\
\addlinespace[4pt]
VBench-1.0 & Vendored VBench evaluator & Revision: \nolinkurl{VBench-official-fd18b3d}. \\
\addlinespace[4pt]
MemFlow $60$\,s & VBench-Long ($7$ sub-dimensions); CLIP ViT-L/14 & Six $10$\,s prompt intervals per $59.875$\,s video ($1{,}437$ frames at $24$\,fps); evaluated with matched native controls. \\
\bottomrule
\end{tabular}
\end{minipage}
\par\medskip
\endgroup

\begingroup
\small
\setlength{\tabcolsep}{4pt}
\renewcommand{\arraystretch}{1.12}
\par\medskip\noindent
\begin{minipage}{\linewidth}
\centering
\small
\captionof{table}{\textbf{The STEM suite contains 4,145 questions, including 829 development questions.} Full and development counts are shown for each subject or domain; MMLU, SciQ, and ARC-Challenge use their \texttt{test} splits.}\label{tab:supp_reasoning_subsets}
\begin{tabular}{@{}>{\raggedright\arraybackslash}p{0.32\linewidth} >{\raggedright\arraybackslash}p{0.42\linewidth}|rr@{}}
\toprule
\textbf{Subject or domain} & \textbf{Exact task identifier} & \textbf{Full} & \textbf{Dev.} \\
\midrule
\multicolumn{4}{@{}l}{\textbf{MMLU Hard-STEM}}\\
College physics & \nolinkurl{college_physics} & 102 & 20 \\
High-school physics & \nolinkurl{high_school_physics} & 151 & 30 \\
High-school mathematics & \nolinkurl{high_school_mathematics} & 270 & 54 \\
Abstract algebra & \nolinkurl{abstract_algebra} & 100 & 20 \\
College chemistry & \nolinkurl{college_chemistry} & 100 & 20 \\
High-school statistics & \nolinkurl{high_school_statistics} & 216 & 43 \\
Econometrics & \nolinkurl{econometrics} & 114 & 23 \\
College computer science & \nolinkurl{college_computer_science} & 100 & 20 \\
Professional medicine & \nolinkurl{professional_medicine} & 272 & 55 \\
Medical genetics & \nolinkurl{medical_genetics} & 100 & 20 \\
\textbf{MMLU subtotal} & & \textbf{1,525} & \textbf{305} \\
\midrule
SciQ & \nolinkurl{sciq} & 1,000 & 200 \\
ARC-Challenge & \nolinkurl{arc_challenge} & 1,172 & 234 \\
\midrule
\multicolumn{4}{@{}l}{\textbf{GPQA-Main}}\\
Chemistry & \nolinkurl{gpqa_main_zeroshot} & 183 & 37 \\
Physics & \nolinkurl{gpqa_main_zeroshot} & 187 & 37 \\
Biology & \nolinkurl{gpqa_main_zeroshot} & 78 & 16 \\
\textbf{GPQA subtotal} & & \textbf{448} & \textbf{90} \\
\midrule
\textbf{Total} & & \textbf{4,145} & \textbf{829} \\
\bottomrule
\end{tabular}
\end{minipage}
\par\medskip
\endgroup
