# Supplementary material for: Evolving Loop Programs: Discovering How Frozen Transformers Should Loop
Source: arXiv:2611.41108 source file (2026-12-03)
Supplement: Supplementary file 6 [file appendix_experiment_settings.tex]

\section{Experiment Settings and Reproduction Details}
\label{sec:supp_exp_settings}

\subsection{Search Protocols, Inference Specifications, and Hardware}
\label{sec:supp_exp_tables}

Tables~\ref{tab:supp_exp_settings} and~\ref{tab:supp_repro_details} summarize search settings and replay specifications for all nine frozen backbones. Read the modality groups in Table~\ref{tab:supp_exp_settings} to compare edit scope, data partitions, and objectives; Table~\ref{tab:supp_repro_details} records sampling, hardware, and native compute references. Full evaluations combine development and validation partitions and therefore include search examples.

\paragraph{Shared search budgets and LLMs.}
Unless noted here, each search evaluates $80$ unique candidates over nine rounds ($16+8\times8$). Dory open-ended search instead uses five rounds of eight candidates ($40$ total), and the $60$\,s multi-prompt LongLive~2.0 initial-context searches evaluate $32$ unique candidates over four rounds ($4\times8$) with up to two diagnostic probes per round. Across backbones, video and world-model searches (LongLive~1.0/2.0 RememBench, Self-Forcing, Wan2.1, and LongLive~2.0 $60$\,s Minimal) use Minimal initial search context $\mathcal{C}_0$ (except the Matched and Library-only ablation regimes), whereas image and text-reasoning backbones mostly use Matched priors pairing domain guidance with starter operators and measured loop anchors (Section~\ref{sec:supp_context_ablation}). Anchor counts in Table~\ref{tab:supp_exp_settings} are per run; ``2 + 1 synthetic'' means two measured anchors plus one shifted target. The table abbreviates \texttt{GPT-6-Astra} (\texttt{xhigh}) as \texttt{Astra}, \texttt{Gemini-4-Argon} (\texttt{high}) as \texttt{Argon}, and \texttt{Gemini-4-Carbon} (\texttt{high}) as \texttt{Carbon}. ``Program + probes'' denotes program editing with diagnostics; the configuration and zero-probe ablations are marked explicitly.

\paragraph{Image-search objectives and confirmation.}
Here, $s_{\mathrm{lat}}$ denotes measured warm-batch latency speedup; the joint image objective is the three-dimensional Pareto vector of GenEval, DPG, and $s_{\mathrm{lat}}$. Replay tables report inference FLOPs separately. GenEval-only and DPG-only optimize one score, retain latency only as telemetry, and cross-evaluate the other benchmark. Held-out and full results are reported for every setting; development results are also reported for Scale-RAE main/\texttt{Argon}, RAE, Looped-DiT, Qwen, and Wan. RAE uses the DiffusionBench \texttt{RAE-SigLIP2-B/DDT} 615M adaptation documented below.

\paragraph{Text- and video-search objectives.}
Qwen's five quality coordinates are \nolinkurl{acc_norm}, \nolinkurl{accuracy}, \nolinkurl{macro_group_accuracy}, \nolinkurl{margin_score}, and \nolinkurl{logprob_score}; no cost coordinate is optimized. Mild/Strong/Extreme shift the target by $+1.57/+3.02/+6.03$\,pp. Qwen and Dory STEM use the four-benchmark local suite detailed below; Dory open-ended uses IFBench, GPQA Diamond, and SciCode, with eight runs per prompt. Its STEM cost is measured in GFLOPs/token. Long-video RememBench search optimizes \nolinkurl{clip_mean} and $1/(1+\text{\nolinkurl{lpips_mean}})$, excludes cost, and reports TempSSIM post hoc. On $60$\,s multi-prompt LongLive~2.0, the $2{\times}2$ initial-context searches optimize a 5D Pareto vector of normalized VBench-Long Quality, Consistency, mean CLIP ViT-L/14, worst-$10$\,s-segment CLIP shift, and wall-clock diffusion speedup against the zero reference; the restricted fixed-schedule comparator optimizes the 3D quality-only tuple of normalized Quality, Consistency, and mean CLIP ViT-L/14. Wan uses the local \nolinkurl{vbench_expanded_text_v1} collection and a native $50$-step anchor. Speed/Balanced target higher \nolinkurl{quality_score} and \nolinkurl{semantic_score} with lower measured latency; Quality/Quality-alt. target those scores plus \nolinkurl{total_score}, without cost.

\input{sec/table_search_settings}

\input{sec/table_replay_settings}

\subsection{Evaluation Scopes, Asset Provenance, and Rollout Conventions}
\label{sec:supp_eval_scopes}

\paragraph{Text and short-video evaluation scope.}
\label{sec:supp_local_protocols}
The text suite contains a local $1{,}525$-question STEM subset of
MMLU~\cite{hendrycks2021measuring}, $448$ GPQA-Main questions,
$1{,}172$ ARC-Challenge questions, and $1{,}000$ SciQ questions.
``MMLU-STEM'' in the tables denotes this local subset, rather than a
separate benchmark defined by the original MMLU paper.
The benchmark families follow Training-Free Looped Transformers~\cite{chen2026trainingfreelooped};
its reported gains on knowledge-intensive tasks motivate our STEM focus.
The local subset and aggregate summaries are specific to this study,
rather than an exact reproduction of that paper's evaluation suite.
The $829$-question development panel uses stratified quotas and baseline-informed
calibration on metadata and full-suite baseline outputs (seed $1234$), without
using Fixed Loop or candidate scores; the remaining $3{,}316$ questions are
excluded from candidate search.
With benchmark accuracy $a_b$ and count $n_b$, Micro Acc weights each
question equally, $\sum_b n_b a_b / 4{,}145$, whereas Macro Group gives
each of the four benchmarks equal weight, $\frac{1}{4}\sum_b a_b$.
These definitions reproduce the displayed aggregates up to rounding.
Micro Acc Norm averages correctness after selecting answers by
character-length-normalized likelihood on ARC-Challenge and SciQ, and
ordinary likelihood on the other benchmarks. Macro Domain is a separate evaluator-reported
aggregate and is not interchangeable with the four-benchmark mean
(the breakdown below details the $10$ MMLU Hard-STEM subjects, \texttt{SciQ}
\texttt{test} split, answer scoring, and $15$-domain unweighted aggregation).

The short-video results use VBench scoring on a local $256$-video
collection. This count identifies the evaluated sample, not coverage of
all prompts in the official benchmark. All Wan2.1-1.3B baselines and frozen programs are compared
under this common $256$-video protocol (see Tables~\ref{tab:supp_exp_settings}--\ref{tab:supp_repro_details}
and the breakdown below for resolution, frame count, seed, evaluator revision, and baseline reference).

\paragraph{RAE checkpoint and replay provenance.}
\label{sec:supp_rae_provenance}
RAE denotes the DiffusionBench~\cite{leng2026diffusionbench} RAE-SigLIP2-B/DDT 615M text-to-image
adaptation evaluated here, not the official RAEv2 release.
The asset manifest records the source and checkpoint identities below.
\begingroup
\small\raggedright
\noindent\textbf{Source:} \nolinkurl{diffusion-bench/diffusion-bench}\par
\noindent\textbf{Revision:} \nolinkurl{a4a0f5c22e70f7f253f47a5250b478ae5084acd7}\par
\noindent\textbf{EMA checkpoint:} \nolinkurl{t2i-ddt-en28d1152hd72-dn2d2048hd128-rae-siglip2-vit-b-vpred-t4-v1.pt}\par
\noindent\textbf{Recorded SHA-256:} \nolinkurl{557c878ed8ab288dadc62a6b08ac21ad720c56165c1ba9d88b77d9dc59a7ef00}\par
\endgroup
\noindent Text conditioning uses \texttt{Qwen/Qwen3-0.6B}; decoding uses the
SigLIP2-ViT-B decoder. Generation retains the stored checkpoint tensor
dtypes with BF16 autocast, seed $42$, and generation/decode batches of
$16$ at native $256\times256$ resolution. GenEval uses batch size $4$;
DPG uses question batch size $32$ and crop resolution $256$.
The three control rows and the six-/ten-step programs in
Table~\ref{tab:supp_main_results_balanced} match the saved full-replay
reports under this protocol. These results establish behavior of this
evaluated checkpoint, not of a later official RAEv2 model.

\input{sec/appendix_evaluation_details}

\paragraph{Selection and replay.}
After the final search round, the coordinator records frontier recommendations and freezes candidate snapshots in replay manifests before confirmation. Section~\ref{sec:supp_selection_records} identifies the selected source snapshots and replay records; Tables~\ref{tab:supp_exp_settings} and~\ref{tab:supp_repro_details} specify the evaluation scopes and execution settings.

\paragraph{Video rollout and compute conventions.}
LongLive 2.0, LongLive 1.0, and Self-Forcing generate chunks autoregressively with diffusion denoising within each chunk. Under the unified RememBench rollout protocol, videos follow the official T2V test prompt-switching schedule aligned to chunk boundaries ($379$ frames at $24$\,fps, scoring departure/revisit frames $86$ and $378$). Figure~\ref{fig:teaser}d reports $100(o-b)/b$ for CLIP and $100(b-o)/b$ for LPIPS, where $b$ and $o$ are the baseline and program scores. LongLive 2.0 repeats blocks $11$--$18$ with $K{=}6$; LongLive 1.0 uses $K{=}8$ over blocks $11$--$17$ in the first two denoising steps of each chunk; Self-Forcing uses a $21$-frame attention window and evaluates an independent $20/80$ \papershort{} program (blocks $14$--$19$, $K{=}6$) under the same $379$-frame protocol in Table~\ref{tab:longlive10_loop_variants}(b). For the $60$\,s multi-prompt MemFlow evaluation on LongLive~2.0~5B, each video runs $45$ chunks of $8$ latent frames ($1{,}437$ decoded frames at $24$\,fps = $59.875$\,s) at $1280{\times}704$ resolution across six $10$\,s prompt segments (switching every $7$--$8$ chunks), with $4$-step native UniPC totaling $30{,}086$\,TFLOPs ($4.54$\,TFLOPs per full CausalWan block vs.\ $0.33$\,TFLOPs per cross-attention sublayer).

\paragraph{Text loop configurations.}
The Fixed Loop baseline follows the frozen-checkpoint, damped-Euler approach of Training-Free Looped Transformers~\cite{chen2026trainingfreelooped}, repeating Qwen3-4B blocks $[15,18]$ with $K{=}3$. Searched programs use dual-window RK3 updates on Qwen3-4B and elastic recurrent-depth updates with KV reuse on Dory1.0-4B; Table~\ref{tab:supp_searched_solutions} records their detailed settings.

\FloatBarrier
\subsection{Search Cost and Token Usage}
\label{sec:supp_search_cost}

Search is performed offline for each setting. Search LLM usage is similar across tasks, while candidate evaluation runtime varies with the backbone and task. Per nine-round ($80$-candidate) search, reasoning and code generation by the search LLM take roughly $0.7$--$2$\,hours of wall-clock time ($2.7$\,hours with extra diagnostic turns on Looped-DiT-B32). Over a full executable-program search, \texttt{GPT-6-Astra} processes roughly $6$--$20$\,M input tokens (about $90\%$ served from prompt cache in the image searches; $1.8$\,M for restricted configuration search) and generates $0.07$--$0.19$\,M output tokens, including reasoning, whereas \texttt{Gemini-4-Argon} uses roughly $11$--$33$\,M uncached input tokens ($31$--$187$\,M cached reads) and $1.9$--$4.4$\,M output tokens, including thinking ($85$\,M and $8.1$\,M in the $22$-turn Looped-DiT-B32 run). For the four $32$-candidate $60$\,s LongLive~2.0 context searches (\texttt{Gemini-4-Argon}, $11$--$15$ turns, $3$--$7$ diagnostic probes), search-LLM reasoning takes $0.67$--$0.99$\,hours ($4.0$--$6.8$\,hours end-to-end across $32{\times}$\,H100 GPUs including evaluation rounds and probes), using $11.4$--$31.9$\,M uncached input tokens ($52.8$--$148.3$\,M cached reads) and $1.28$--$2.42$\,M output tokens including $0.85$--$1.46$\,M thinking.

Candidate evaluation on the development split accounts for the remaining runtime: on a single RTX~5090 GPU, evaluating $80$ candidates plus the two measured anchors takes $1.3$--$1.8$\,hours for Qwen3-4B; candidate evaluation takes $4.0$--$5.9$\,hours for RAE and joint Scale-RAE ($3.4$--$7.2$\,hours end-to-end per search), whereas Looped-DiT-B32 ($0.9$\,hours evaluation, $3.8$\,hours end-to-end) and the video searches distribute candidate rollouts across $32$~H100 GPUs.

All search time and token costs are incurred once offline per setting; at deployment, the frozen program runs inside the backbone without calls to the search LLM or associated token overhead.
