# Supplementary material for: Evolving Loop Programs: Discovering How Frozen Transformers Should Loop
Source: arXiv:2611.41108 source file (2026-12-03)
Supplement: Supplementary file 7 [file appendix_human_alignment.tex]

\section{Do Discovered Loop Programs Align with Human-Designed Principles?}
\label{sec:supp_human_alignment}

A natural question raised by automated program discovery is whether \papershort{} uncovers genuinely general inference mechanisms or merely backbone-specific heuristics. Comparing the frozen programs in Table~\ref{tab:supp_searched_solutions} across six independent design axes reveals a deeper answer: without closed-form derivations or hand-engineered recipes, diagnostic-guided search repeatedly rediscovers core structural, dynamical, and systems laws established independently by human researchers---yet also pinpoints where naive rules of thumb fail and must be co-adapted jointly across axes. Table~\ref{tab:supp_human_alignment} maps each discovered mechanism to its human-designed literature; below, we distill these alignments into four mechanistic insights.

\begin{table*}[!htbp]
\centering
\caption{\textbf{\papershort{} independently rediscovers six human-designed inference principles across depth, time, geometry, scheduling, memory, and reuse, while refining or falsifying brittle heuristics via diagnostics.} Main-paper references use~\cite{chen2026trainingfreelooped} numbering; supplementary-only works use~\citesupp{fishman2026dory}.}
\label{tab:supp_human_alignment}
\footnotesize
\setlength{\tabcolsep}{3pt}
\renewcommand{\arraystretch}{1.15}
\begin{tabular*}{\textwidth}{@{}@{\extracolsep{\fill}}>{\raggedright\arraybackslash}p{0.145\textwidth} >{\raggedright\arraybackslash}p{0.275\textwidth} >{\raggedright\arraybackslash}p{0.265\textwidth} >{\raggedright\arraybackslash}p{0.255\textwidth}@{}}
\toprule
\textbf{Design Axis} & \textbf{\papershort{}-Discovered Mechanism} & \textbf{Aligned Human-Designed Literature} & \textbf{Convergence vs.\ Refinement} \\
\midrule
\textbf{1. Depth placement} &
Interior middle-to-slightly-post-center bands across unlooped backbones (LongLive~1.0 $12$--$18/30$, LongLive~2.0 $11$--$18/30$ \& $60$\,s $13$--$18$ / cross-attention blocks $8$--$24/30$, Self-Forcing $14$--$19/30$, Scale-RAE $12$--$27/32$, RAE $19$--$22/28$, Qwen3-4B $[14]{+}[15..18]$ + $25$--$28/36$). &
Layers as Painters~\citesupp{sun2025painters}; Layer by Layer~\citesupp{skean2025layer}; Global Workspace / J-space~\citesupp{gurnee2026workspace}; Train-Free Looped~\cite{chen2026trainingfreelooped}; Inkling~2 Mini~\citesupp{tml2026inkling2}. &
\textbf{Aligns} on avoiding boundary layers and targeting middle semantic layers; \textbf{refines} via controlled LongLive~1.0 sweep showing metric-dependent post-center gains ($11$--$17 \to 12$--$18$). \\[3pt]
\textbf{2. Noise / temporal gating} &
Concentrate loops in high-noise early steps and skip low-noise steps ($K_t{=}0$): $t/T{\le}0.5$ on Scale-RAE/RAE, $t/T{\in}[0.05,0.40)$ on Wan2.1, noise-tracked $\{0,1\}$ vs.\ $\{0,1,2\}$ on LongLive~1.0/2.0. &
P2 Weighting~\citesupp{choi2022p2}; eDiff-I~\citesupp{balaji2022ediffi}; Limited-Interval Guidance~\citesupp{kynkaanniemi2024interval}; Flow-Matching Looping~\cite{yan2026trainingfree}. &
\textbf{Aligns} with hierarchical denoising (high noise = layout/identity; low noise = texture) and bounded guidance intervals; automatically tracks noise-schedule shifts rather than raw step index. \\[3pt]
\textbf{3. State-update dynamics} &
Damped Euler ($\lambda/K$); higher-order RK3 (Qwen3-4B), RK2 (Wan2.1), and tapered $x_0$ AB2 (Looped-DiT); spherical/geodesic extrapolation on hyperspherical Dory1.0-4B ($K{=}2$/$3$ beating native $K{=}4$/$6$). &
Neural ODEs~\citesupp{chen2018neuralode}; PNDM~\citesupp{liu2022pndm}; DPM-Solver~\citesupp{lu2022dpmsolver}; UniPC~\citesupp{zhao2023unipc}; Train-Free Looped~\cite{chen2026trainingfreelooped}; Rectified Loop~\cite{li2026rectified}; nGPT~\citesupp{loshchilov2025ngpt}. &
\textbf{Aligns} with ODE integration and hyperspherical geometry (nGPT geodesics on Dory1.0); \textbf{extends} by matching solver order and manifold geometry to each frozen checkpoint. \\[3pt]
\textbf{4. Timestep \& depth allocation} &
Curvature-warped SNR schedule ($s{\in}[1.30,1.38]$, $c_u{\in}[0.04,0.05]$) paired with adaptive $K_t{\in}\{4,2\}$ on Looped-DiT-B32, guided by velocity second-difference probes ($0.836$ at $t{=}0.02$ vs.\ $0.018$ mid-trajectory). &
Align Your Steps~\citesupp{sabour2024ays}; GITS Trajectory Regularity~\citesupp{chen2024gits}; SD3 SNR Shift~\citesupp{esser2024sd3}; Adaptive Loop Depth (Ouro~\cite{zhu2025ouro}, MoR~\cite{bae2025mixture}, LiFT~\cite{derakhshani2026lift}). &
\textbf{Aligns} with curvature-proportional discretization and non-uniform recurrent depth; \textbf{co-designs} schedule warping jointly with latent extrapolation and residual reuse ($+1.32$\,pp over schedule-only). \\[3pt]
\textbf{5. Recurrent KV-cache control} &
Read-only intermediate loop passes with deferred final-pass / converged last-loop KV commits across LongLive~1.0/2.0, Self-Forcing, Qwen3-4B, and Dory1.0-4B. &
Self-Forcing~\cite{huang2025selfforcing} \& LongLive~\cite{yang2026longlive} exposure bias; Huginn~\cite{geiping2025recurrent}, MoR~\cite{bae2025mixture}, MELT~\citesupp{vendrell2026melt}, FlashLoop~\citesupp{yang2026flashloop} KV consolidation. &
\textbf{Aligns} on avoiding linear per-loop KV bloat and error compounding; \textbf{improves} over first-pass KV sharing by committing the converged last pass, boosting accuracy rather than trading it off. \\[3pt]
\textbf{6. Modality split \& bounded reuse} &
Cache slow conditioning streams (RAE $\Delta_{\mathrm{cond}}$, Looped-DiT text preamble, Wan2.1 \& $60$\,s LongLive~2.0 cross-attention); cap reuse lag ($\le\!1$ step in Scale-RAE, age $\le\!2$ in Looped-DiT); reject cross-step CFG reuse. &
DeepCache~\citesupp{ma2024deepcache}; TeaCache~\citesupp{liu2025teacache}; TaylorSeer~\citesupp{liu2025taylorseer}; PAB~\citesupp{zhao2025pab}; FasterCache~\citesupp{lv2025fastercache}. &
\textbf{Aligns} on slow text/cross-attention dynamics and smooth mid-trajectory residuals; \textbf{falsifies} blanket CFG/multi-step reuse when probes reveal high branch variance ($0.528$--$0.735$). \\
\bottomrule
\end{tabular*}
\end{table*}

\paragraph{1. A shared spatial--temporal law: repeat only inside the malleable, globally consequential core.}
Across both network depth and denoising/reasoning time, \papershort{} allocates extra passes only where representations remain plastic yet determine global structure. Spatially, every unlooped backbone avoids boundary layers and places recurrence in contiguous middle-to-slightly-post-center blocks (Section~\ref{sec:supp_programs}). This converges with mechanistic interpretability and pretraining studies showing that early/final layers are specialized input/output interfaces while middle layers share a unified latent canvas---\emph{Transformer Layers as Painters}~\citesupp{sun2025painters} demonstrates middle-layer interchangeability, \emph{Layer by Layer}~\citesupp{skean2025layer} finds intermediate layers peak in compressed semantic fidelity, Gurnee et~al.~\citesupp{gurnee2026workspace} localize verbalizable multi-hop reasoning (``J-space'') to an intermediate band whose ablation collapses multi-step reasoning, Training-Free Looped Transformers~\cite{chen2026trainingfreelooped} place frozen-LLM loops near mid-depth, and Inkling~2 Mini~\citesupp{tml2026inkling2} confirms that looping middle layers ($7$--$18$ of $24$) beats late layers ($13$--$24$) on $27$ of $28$ evaluations at equal compute ($1.51\times$--$1.91\times$ vs.\ $1.24\times$--$1.36\times$ compute-equivalent gain). \papershort{}'s own diagnostics explain the boundary pathology directly (negative input--residual alignment at block~$1$ and a terminal residual spike at block~$29$ in LongLive~2.0), while our controlled fixed-width, fixed-$K$ LongLive~1.0 sweep (Table~\ref{tab:longlive10_loop_variants}(a)) adds precision: shifting the same seven-block window slightly past exact center ($11$--$17 \to 12$--$18$ of $30$) sharpens CLIP and LPIPS, whereas earlier $9$--$15$ maximizes TempSSIM, establishing metric dependence within the middle band (while Qwen3-4B's dual window $[14]{+}[15..18]$ and $25$--$28$ reflects a combined program edit that also changes the state update to RK3). Temporally, \papershort{} enforces the exact dual of this spatial rule: it turns loops on only in high-noise or high-curvature phases---skipping low-noise texture refinement ($K_t{=}0$ past $t/T{=}0.5$ in Scale-RAE/RAE, outside $t/T{\in}[0.05,0.40)$ in Wan2.1 Speed, and tracking the shift-$5$ noise schedule from $\{0,1\}$ in LongLive~1.0 to $\{0,1,2\}$ in LongLive~2.0) while concentrating outer steps where Round~$0$ probes detect an order-of-magnitude velocity-curvature spike near early steps on Looped-DiT-B32 (Appendix~\ref{sec:supp_looped_dit}). This unifies hierarchical noise specialization (P2~\citesupp{choi2022p2}, eDiff-I~\citesupp{balaji2022ediffi}), Limited-Interval Guidance~\citesupp{kynkaanniemi2024interval}, flow-matching loop gating~\cite{yan2026trainingfree}, curvature-proportional discretization (Align Your Steps~\citesupp{sabour2024ays}, GITS~\citesupp{chen2024gits}, SD3 SNR shifts~\citesupp{esser2024sd3}), and adaptive recurrent compute~\cite{zhu2025ouro,bae2025mixture,derakhshani2026lift} under one allocation principle.

\paragraph{2. Manifold geometry and integrator order substitute for raw loop depth.}
A recurring lesson across human solvers and \papershort{}'s discovered rules is that repeating a block naively degrades frozen checkpoints because unscaled residual feedback pushes hidden states off their trained norm and trajectory manifold~\cite{chen2026trainingfreelooped}. Consistent with the continuous-depth Neural ODE formulation~\citesupp{chen2018neuralode} and high-order diffusion integrators (PNDM~\citesupp{liu2022pndm}, DPM-Solver~\citesupp{lu2022dpmsolver}, UniPC~\citesupp{zhao2023unipc}), \papershort{} systematically replaces raw repetition with step-normalized Euler ($\lambda/K$), higher-order multi-stage integrators (tapered/anchored RK3 on Qwen3-4B; spacetime curvature-lookahead RK2 on Wan2.1; tapered $x_0$ AB2 on Looped-DiT-B32), and stabilized substeps or endpoint interpolation~\cite{chen2026trainingfreelooped,li2026rectified}. Crucially, the search adapts the solver to the native geometry of the pretrained weights: on Dory1.0-4B~\citesupp{fishman2026dory}---a looped normalized-GPT built on nGPT's unit-hypersphere representation~\citesupp{loshchilov2025ngpt}---\papershort{} abandons Euclidean extrapolation and independently discovers \emph{spherical velocity and bounded geodesic extrapolation}. Because moving along geodesics respects the hyperspherical manifold where Dory1.0's residual updates live, a $K{=}2$ or $K{=}3$ geodesic rule outperforms deeper native $K{=}4$ and $K{=}6$ iteration (Tables~\ref{tab:supp_dory_gen}--\ref{tab:supp_dory_stem4145}), showing that geometry-matched dynamics can substitute for raw recurrent compute.

\paragraph{3. Decoupling transient refinement from persistent memory and slow context.}
In both autoregressive rollouts and multimodal diffusion, naive looping wastes compute or corrupts state when transient inner-loop iterations contaminate persistent state or re-evaluate slowly varying inputs. Across every autoregressive model (LongLive~1.0/2.0, Self-Forcing, Qwen3-4B, and Dory1.0-4B), \papershort{} keeps intermediate loop passes read-only and commits only the final converged state to the KV cache. In causal video diffusion, this prevents intermediate loop transients from compounding across future chunks via exposure bias~\cite{huang2025selfforcing,yang2026longlive}, cutting severe revisit collapse nearly tenfold ($48 \to 5$ scenes) with zero weight updates. In recurrent-depth language models, it converges with the systems drive in Huginn~\cite{geiping2025recurrent}, Mixture-of-Recursions (MoR)~\cite{bae2025mixture}, MELT~\citesupp{vendrell2026melt}, and FlashLoop~\citesupp{yang2026flashloop} to eliminate linear per-loop KV memory bloat---yet improves upon MoR's first-pass KV-sharing compromise by committing the \emph{converged last-loop} KV state on Dory1.0-4B, which lifts held-out GPQA Diamond by $+1.74$\,pp over native $K{=}2$ per-loop KV rather than trading accuracy for memory. The exact dual appears in diffusion acceleration: mirroring DeepCache~\citesupp{ma2024deepcache}, TeaCache~\citesupp{liu2025teacache}, TaylorSeer~\citesupp{liu2025taylorseer}, and Pyramid Attention Broadcast (PAB)~\citesupp{zhao2025pab}, \papershort{} separates slow conditioning from fast spatial refinement---caching $\Delta_{\mathrm{cond}}$ and sharing unlooped prefix blocks $0$--$18$ in RAE, caching the text preamble in Looped-DiT, and restricting Wan2.1 Speed and Minimal-context $60$\,s LongLive~2.0 loops to cross-attention ($0.33$ vs.\ $4.54$\,TFLOPs per block, consistent with PAB's hierarchy of slow cross-attention vs.\ rapid spatial updates).

\paragraph{4. Beyond rediscovery: diagnostic falsification and non-additive cross-axis co-design.}
If \papershort{} only reproduced isolated rules from prior papers, manual composition might suffice. Instead, our ablations reveal two reasons why diagnostic-guided program search outperforms hand-assembled heuristics. First, passive probes \emph{falsify plausible caching rules when a backbone violates their assumptions}: whereas FasterCache~\citesupp{lv2025fastercache} reuses CFG differences across steps on several video DiTs, \papershort{}'s Round~$0$ probes on Looped-DiT-B32 detect large cross-step CFG variance (and Scale-RAE probes detect lag-$\ge\!2$ guidance drift despite ${>}0.994$ output cosine), explaining why blind CFG reuse or unconditional-loop pruning collapsed GenEval whereas short-horizon late-loop residual reuse (cosine ${>}0.997$) succeeded. Second, effective loop programs rely on \emph{non-additive coupling across axes}: in LongLive~2.0, shifting the loop boundary to block~$11$ failed until step~$0$ was co-activated ($\Delta\mathrm{HV}{=}+0.036$, Section~\ref{sec:supp_longlive10_additional}); on Looped-DiT-B32, co-designing latent/$x_0$ dynamics and bounded residual reuse with curvature-matched scheduling adds $+1.32$\,pp GenEval and $+1.13$\,pp DPG over the matched-compute schedule-only control (Table~\ref{tab:supp_looped_dit_splits}); and on Scale-RAE and RAE, co-adapting middle-band loops with bounded reuse reverses prior training-free looping's latency penalty~\cite{yan2026trainingfree} into $1.61\times$--$5.19\times$ FLOPs speedups with higher compositional accuracy. Offline program search therefore functions as a diagnostic-driven scientific loop: rediscovering sound principles, rejecting mismatched heuristics, and co-tuning the surviving mechanisms into one coherent inference program.
