# Supplementary material for: Evolving Loop Programs: Discovering How Frozen Transformers Should Loop
Source: arXiv:2611.41108 source file (2026-12-03)
Supplement: Supplementary file 8 [file appendix_looped_dit.tex]

\FloatBarrier
\section{Looped-DiT Case Study: From Diagnostics to Frozen Programs}
\label{sec:supp_looped_dit}

This case study expands the pretrained-looped image-model comparison in RQ1 (Appendix~\ref{sec:supp_looped_results}) and illustrates how programmable diagnostics drive executable edits in structure, dynamics, and control. We run \paper{} offline on frozen Looped-DiT-B32~\cite{chng2026looped} ($6$ pre-loop blocks, a weight-tied $5$-block core repeated $K{=}4$ times per step, and $6$ post-loop blocks; effective depth $32$, with a $100$-step / $400$-core-pass native reference) using \texttt{Gemini-4-Argon} over $80$ unique candidates across nine rounds on $320$ stratified development prompts ($112$ GenEval, $208$ DPG-Bench; $4$ seeds per prompt), holding out $1{,}298$ prompts ($441$ GenEval, $857$ DPG-Bench) strictly for post-search confirmation. Pretrained weights remain frozen throughout, and full protocol details appear in Appendix~\ref{sec:supp_exp_settings}.

\subsection{Diagnostics, Program Design, and Search Evolution}
\label{sec:supp_looped_dit_diag}
\label{sec:supp_looped_dit_setup}

\paragraph{Programmable diagnostics.}
Before proposing candidates in $\text{R0}$, the search LLM wrote lightweight diagnostic collectors (defined formally in Appendix~\ref{sec:supp_observations}) and verified bit-exact image parity on $16$ anchor prompts. The recorded trajectory statistics separated stable vs.\ unstable reuse axes:
\begin{itemize}
    \item \textbf{Velocity curvature.} Relative velocity second-difference curvature is concentrated sharply near trajectory endpoints (peaking at $0.836$ at $t{=}0.02$) and collapses by over an order of magnitude across the flat mid-trajectory ($t \in [0.15, 0.50]$), immediately motivating curvature-warped rather than uniform timestep allocation.
    \item \textbf{Loop-residual stability.} Late-loop increments $(\mathbf h^{(4)}-\mathbf h^{(2)})$ remain tightly aligned across adjacent steps (cosine similarity ${>}0.997$ beyond $t{=}0.10$) while within-step updates progressively align with depth, confirming that late-loop residuals can be safely cached over short horizons.
    \item \textbf{Guidance-branch variation.} By contrast, cross-step relative variation in the classifier-free guidance difference stays high throughout sampling ($0.53$--$0.74$), directly falsifying naive cross-step guidance reuse and explaining why early $\text{R0}$ pruning attempts collapsed GenEval and were discarded.
\end{itemize}

\paragraph{Discovered program mechanisms.}
Guided by these diagnostics (complementing the direct diagnostic-access ablation on Scale-RAE in Table~\ref{tab:ablation_diagnostics}), the search LLM co-designed four complementary mechanisms across structure, dynamics, and control:
\begin{enumerate}[nosep,leftmargin=*]
    \item \textbf{Control: curvature-based timestep allocation.} An SNR shift ($s \in [1.30, 1.38]$) paired with a sinusoidal curvature warp ($c_u \in [0.04, 0.05]$) concentrates steps in early high-curvature regions, raising $25$-step development GenEval at fixed $K{=}4$ from $84.56\%$ to $85.49\%$ ($+0.93$\,pp).
    \item \textbf{Dynamics: latent extrapolation in both streams.} On full $4$-loop refresh steps, starting at $t{=}0.12$--$0.15$ depending on the program and ending before $t{=}0.90$, both image and text states extrapolate along their last core increment $\Delta\mathbf h^{(4)}=\mathbf h^{(4)}-\mathbf h^{(3)}$ ($\alpha \in [0.18, 0.22]$) with zero extra core passes.
    \item \textbf{Dynamics: tapered $x_0$ extrapolation.} A step-size-aware second-order Adams--Bashforth update ($\beta \in [0.32, 0.35]$) tapers linearly over $t \in [0.80, 0.94]$ to prevent late-step oversharpening as $(1-t)\rightarrow0$, lifting the $25$-step program to $86.34\%$ development GenEval.
    \item \textbf{Structure and control: bounded residual reuse.} Alternating $K_t\in\{2,4\}$ steps along an LCM-aligned stride reuses cached $(\mathbf h^{(4)}-\mathbf h^{(2)})$ in both streams with cache age capped at $\le2$ steps, reducing core passes from $80$ to $68$ at $20$ steps and from $56$ to $48$ at $14$ steps.
\end{enumerate}

\paragraph{Search evolution.}
Across the $80$ validated candidates (excluding exact duplicates and three failed attempts), cumulative development hypervolume over GenEval, DPG, and FLOPs speedup roughly doubles ($+102.1\%$). Nearly all of this frontier jump (${\sim}97\%$) arrives in the first two rounds ($\text{R0}$--$\text{R1}$, $24$ evaluations), showing that once upfront diagnostics separate high-curvature scheduling and stable late-loop reuse from unstable guidance caching, the search locks onto the right structural family immediately. Subsequent rounds refine the frontier through tapered multistep $x_0$ updates ($\text{R4}$) and stale-cache-age pruning ($\text{R6}$). (Absolute hypervolume is specific to this backbone and reference, distinct from Scale-RAE in Figure~\ref{fig:teaser}e; full-benchmark evaluations appear in Tables~\ref{tab:looped_dit_main} and~\ref{tab:supp_looped_dit_full_subtasks}.)

\subsection{Held-Out Confirmation and Schedule-Only Comparison}
\label{sec:supp_looped_dit_confirm}

\Cref{tab:supp_looped_dit_splits} evaluates frozen Speed, Balanced, and Quality programs alongside native inference and a $15$-step Schedule-only comparator ($46$ core passes) that omits residual reuse and latent/$x_0$ extrapolation. Two insights emerge on the $1{,}298$ unseen held-out prompts. First, analytical compute savings translate nearly one-to-one into hardware acceleration: measured $32\times\text{H100}$ wall-clock speedups track FLOPs ratios within ${\sim}1\%$ (up to $7.86\times$ for Speed), while Balanced surpasses the $100$-step native reference on held-out GenEval at $5.53\times$ wall-clock speedup and Speed lifts matched-$14$-step native scores by over $+4$\,pp GenEval and $+3.9$\,pp DPG. Second, schedule warping alone is insufficient: at matched compute (${\sim}6.8$\,TFLOPs), the complete Speed program beats the Schedule-only comparator by $+1.32$\,pp GenEval and $+1.13$\,pp DPG, confirming the value of jointly co-designing dynamics and bounded reuse without isolating each sub-component. As in RQ1, the $100$-step native reference keeps a slight held-out DPG edge at $4\times$--$7.8\times$ higher compute, and Full combines development and held-out splits ($\Delta_{\mathrm{step}}$ gives full-benchmark gains over matched-step native $K{=}4$).

\begin{table*}[!htbp]
\centering
\caption{\textbf{\rqhighlight{1}{The complete Speed program outperforms the schedule-only comparator at similar compute on held-out prompts.}} $\Delta_{\mathrm{step}}$ reports full-benchmark gains vs.\ matched-step native inference; Speedup gives FLOPs and $32\times\text{H100}$ wall-clock ratios ($0.814$\,s/img at $100$ steps). Rankings cover all rows; gray marks ours.}
\label{tab:supp_looped_dit_splits}
\scriptsize
\renewcommand{\arraystretch}{0.96}
\setlength{\tabcolsep}{2.7pt}
\begin{tabular}{@{}l r c | c c c c | c c c c | r c@{}}
\toprule
\multirow{2}{*}{\textbf{Method}} & \multirow{2}{*}{\textbf{\#step}} & \textbf{Core} & \multicolumn{4}{c|}{\textbf{GenEval (\%) $\uparrow$}} & \multicolumn{4}{c|}{\textbf{DPG (\%) $\uparrow$}} & \multirow{2}{*}{\textbf{TFLOPs $\downarrow$}} & \textbf{Speedup $\uparrow$} \\
\cmidrule(lr){4-7}\cmidrule(lr){8-11}
 & & \textbf{Passes} & \textbf{Dev.} & \textbf{Held-out} & \textbf{Full} & $\boldsymbol{\Delta}_{\mathrm{step}}$ & \textbf{Dev.} & \textbf{Held-out} & \textbf{Full} & $\boldsymbol{\Delta}_{\mathrm{step}}$ &  & \textbf{(FLOPs / Wall)} \\
\midrule
Native ($K{=}4$)~\cite{chng2026looped} & 100 & 400 & \underline{85.89} & 84.43 & 84.65 & $+0.00$ & \textbf{84.64} & \textbf{85.52} & \textbf{85.34} & $+0.00$ & 53.18 & $1.00\times$ / $1.00\times$ \\
Native ($K{=}1$)~\cite{chng2026looped} & 100 & 100 & 84.21 & 84.68 & 84.47 & $-0.18$ & 83.18 & 84.53 & 84.26 & $-1.08$ & 28.98 & $1.84\times$ / --- \\
Native ($K{=}4$)~\cite{chng2026looped} & 50 & 200 & 85.12 & 84.78 & 84.77 & $+0.00$ & 84.41 & \underline{85.50} & \underline{85.29} & $+0.00$ & 26.59 & $2.00\times$ / --- \\
Native ($K{=}4$)~\cite{chng2026looped} & 25 & 100 & 84.56 & 82.88 & 83.16 & $+0.00$ & \underline{84.51} & 84.82 & 84.76 & $+0.00$ & 13.30 & $4.00\times$ / $4.00\times$ \\
Native ($K{=}4$)~\cite{chng2026looped} & 20 & 80 & 83.21 & 82.06 & 82.26 & $+0.00$ & 84.14 & 84.19 & 84.18 & $+0.00$ & 10.64 & $5.00\times$ / $5.00\times$ \\
Native ($K{=}4$)~\cite{chng2026looped} & 15 & 60 & 81.27 & 79.46 & 79.80 & $+0.00$ & 82.77 & 82.35 & 82.44 & $+0.00$ & 7.98 & $6.67\times$ / $6.67\times$ \\
Native ($K{=}4$)~\cite{chng2026looped} & 14 & 56 & 80.26 & 79.18 & 79.36 & $+0.00$ & 81.26 & 81.32 & 81.31 & $+0.00$ & 7.45 & $7.14\times$ / $7.14\times$ \\
\midrule
\rowcolor{gray!12}
Ours (Speed) & 14 & 48 & 83.77 & 83.39 & 83.43 & \textbf{$+4.07$} & 84.40 & 85.28 & 85.11 & \textbf{$+3.80$} & \textbf{6.80} & $\boldsymbol{7.82\times}$ / \underline{$7.86\times$} \\
\rowcolor{gray!12}
Ours (Balanced) & 20 & 68 & 85.72 & \textbf{84.92} & \underline{85.03} & \underline{$+2.76$} & \underline{84.51} & 85.12 & 85.00 & $+0.82$ & 9.67 & $5.50\times$ / $5.53\times$ \\
\rowcolor{gray!12}
Ours (Quality) & 25 & 100 & \textbf{86.34} & \underline{84.84} & \textbf{85.08} & $+1.92$ & 84.36 & 85.27 & 85.09 & $+0.33$ & 13.30 & $4.00\times$ / $4.01\times$ \\
\rowcolor{gray!12}
Ours (Schedule-only) & 15 & 46 & 83.99 & 82.07 & 82.44 & $+2.65$ & 83.78 & 84.15 & 84.08 & \underline{$+1.64$} & \underline{6.85} & \underline{$7.77\times$} / $\boldsymbol{7.87\times}$ \\
\bottomrule
\end{tabular}
\end{table*}

\FloatBarrier
