# Supplementary material for: Evolving Loop Programs: Discovering How Frozen Transformers Should Loop
Source: arXiv:2611.41108 source file (2026-12-03)
Supplement: Supplementary file 9 [file appendix_observations.tex]

\section{Runtime Observation Definitions}
\label{sec:supp_observations}

Table~\ref{tab:supp_observations} formalizes representative runtime probes used in the RQ2 diagnostic loop of Section~\ref{sec:method} and Section~\ref{sec:exp_design_choices}---spanning Scale-RAE configuration probes (Appendix~\ref{sec:supp_prompts}) and guidance or Looped-DiT probes written during program search (Appendix~\ref{sec:supp_looped_dit_diag})---to diagnose local block changes, core-pass dynamics, late-loop residual stability, and guidance temporal reuse. The search LLM inspects these diagnostics offline and can revise the collectors; deployed programs run without collecting this full observation suite.

\smallskip
\noindent\textbf{Notation.} At sampling step $j$, let $\mathbf a,\mathbf b$ be an observed block's input and output. Let $\mathbf h_j^{(k)}$ and $\mathbf z_j^{(k)}$ be the conditional image and text states after core pass $k$, with increments $\Delta\mathbf h_j^{(k)}=\mathbf h_j^{(k)}-\mathbf h_j^{(k-1)}$ and $\Delta\mathbf z_j^{(k)}=\mathbf z_j^{(k)}-\mathbf z_j^{(k-1)}$. The late-loop residual is $\mathbf r_j=\mathbf h_j^{(4)}-\mathbf h_j^{(2)}$. For Scale-RAE guidance, $\mathbf p_j^{L}$ and $\mathbf p_j^{R}$ denote looped and reference predictions; $\mathbf d_j=\mathbf p_j^{L}-\mathbf p_j^{R}$ is their difference and $w$ is the LoopGuidance weight.

\smallskip
\noindent\textbf{Reductions and availability.} Write $\operatorname{rms}(\mathbf u)=\sqrt{\operatorname{mean}(\mathbf u^2)}$, $\rho(\mathbf u)=\max(\operatorname{rms}(\mathbf u),\epsilon)$, and $\epsilon=10^{-8}$. Norms and means cover the observed tensor elements within one example; $\langle\cdot\rangle_B$ averages per-example measurements over a batch. The Scale-RAE guidance probe subsamples up to $4096$ flattened elements per example and reports means over finite observations. For cosine similarity, Scale-RAE clamps the product of norms below at $10^{-12}$; Looped-DiT clamps each norm below at $\epsilon$. History-dependent measurements require previous observations; late-loop measurements require four passes. Records include step/time and applicable branch/block identifiers.

\begin{table}[!htbp]
\centering
\small
\renewcommand{\arraystretch}{1.3}
\setlength{\tabcolsep}{5pt}
\begin{tabular}{@{}>{\raggedright\arraybackslash}p{0.43\linewidth}>{\raggedright\arraybackslash}p{\dimexpr0.57\linewidth-10pt\relax}@{}}
\toprule
\textbf{Observation} & \textbf{Definition} \\
\midrule
\multicolumn{2}{@{}l}{\textbf{Local block changes (Scale-RAE)}} \\
delta\_rms
& $\operatorname{rms}(\mathbf b-\mathbf a)$ \\
relative\_delta\_rms
& $\displaystyle\frac{\operatorname{rms}(\mathbf b-\mathbf a)}{\max(\operatorname{rms}(\mathbf a),10^{-12})}$ \\[5pt]
cosine
& $\cos(\mathbf a,\mathbf b)$ \\
selected\_fraction
& $\operatorname{mean}(\mathbf m)$, for the binary token-selection mask $\mathbf m$ \\
\midrule
\multicolumn{2}{@{}l}{\textbf{Changes across core passes (Looped-DiT-B32)}} \\
img\_loop\_rel\_delta\_cond
& $\displaystyle\left\langle\frac{\|\Delta\mathbf h_j^{(k)}\|_2}{\max(\|\mathbf h_j^{(k-1)}\|_2,\epsilon)}\right\rangle_B$ \\[5pt]
txt\_loop\_rel\_delta\_cond
& $\displaystyle\left\langle\frac{\|\Delta\mathbf z_j^{(k)}\|_2}{\max(\|\mathbf z_j^{(k-1)}\|_2,\epsilon)}\right\rangle_B$ \\[5pt]
img\_loop\_delta\_cos
& $\left\langle\cos(\Delta\mathbf h_j^{(k)},\Delta\mathbf h_j^{(k-1)})\right\rangle_B$, $k\geq2$ \\
\midrule
\multicolumn{2}{@{}l}{\textbf{Late-loop residual stability (Looped-DiT-B32)}} \\
res\_r2\_to\_r4\_cos\_prev
& $\left\langle\cos(\mathbf r_j,\mathbf r_{j-1})\right\rangle_B$ \\
res\_r2\_to\_r4\_rel\_err
& $\displaystyle\left\langle\frac{\|\mathbf r_j-\mathbf r_{j-1}\|_2}{\max(\|\mathbf r_j\|_2,\epsilon)}\right\rangle_B$ \\[5pt]
\midrule
\multicolumn{2}{@{}l}{\textbf{Guidance magnitude and temporal reuse (Scale-RAE)}} \\
delta\_to\_loop\_ratio
& $\displaystyle\frac{\rho(\mathbf d_j)}{\rho(\mathbf p_j^{L})}$ \\[5pt]
guidance\_extra\_to\_loop\_ratio
& $\displaystyle|w-1|\,\frac{\rho(\mathbf d_j)}{\rho(\mathbf p_j^{L})}$ \\[5pt]
lag$\ell$\_cosine
& $\cos(\mathbf d_j,\mathbf d_{j-\ell})$, $\ell\in\{1,2,3\}$ \\
lag$\ell$\_relative\_error
& $\displaystyle\frac{\operatorname{rms}(\mathbf d_{j-\ell}-\mathbf d_j)}{\rho(\mathbf d_j)}$, $\ell\in\{1,2,3\}$ \\[5pt]
\bottomrule
\end{tabular}
\caption{\textbf{\rqhighlight{2}{Diagnostics measure block updates, loop dynamics, and the stability of reusable corrections.}} Field names follow the implemented collectors. Scale-RAE formulas give per-example measurements; Looped-DiT formulas include the batch reduction. These passive probes preserve candidate outputs.}
\label{tab:supp_observations}
\end{table}
\FloatBarrier
