# Supplementary material for: Evolving Loop Programs: Discovering How Frozen Transformers Should Loop
Source: arXiv:2611.41108 source file (2026-12-03)
Supplement: Supplementary file 10 [file appendix_prompts.tex]

\FloatBarrier
\section{Search LLM Prompts}
\label{sec:supp_prompts}

For the search framework in Section~\ref{sec:method}, this section reproduces (i) the Round-0 instructions prompt instantiated for our primary Scale-RAE program search (Prompt~1, with internal workspace paths anonymized), (ii) the structured per-turn observation payload returned by the coordinator (Prompt~2), and (iii) the prompt adaptations used across ablations and model families (Prompts~3--4). In the prompts and excerpts below, ``OPAL'' refers to the sandboxed code-and-diagnostics execution profile~\cite{bai2026reactive}, and coordinator template variables (\texttt{\$objective}, \texttt{\$search\_prompts}, \texttt{\$last\_group}, \texttt{\$final\_summary}) are resolved prior to Round~0.

\paragraph{Session context and evaluation isolation.}
Distinct from the Round-$0$ \emph{initial search context} $\mathcal{C}_0$ ablated in Section~\ref{sec:supp_context_ablation} (where video and world-model searches primarily use Minimal context and image/text backbones mostly use Matched priors), each search uses one persistent multi-turn conversation and workspace throughout its run; separate runs share no context. The workspace retains code snapshots, hypotheses, notes, evaluation history, and diagnostic outputs. \texttt{GPT-6-Astra} receives the full evaluation history inline; \texttt{Gemini-4-Argon} receives it inline when compact and otherwise a summary with tool access to the full record. Diagnostics provide numerical summaries and saved tensor statistics (Appendix~\ref{sec:supp_observations}); generated images and videos are never shown to the search LLM. During search, evaluation and probes use only development inputs with frozen backbone weights. Held-out inputs and scores, full-split scores, ground-truth labels, evaluator internals, external network access, and other runs are excluded from the LLM's prompts and tools.

\subsection{Primary Program-Search System Prompt}
\label{sec:supp_prompt_primary}

Prompt~1 reproduces the Round-0 instructions supplied to \texttt{GPT-6-Astra} for the Scale-RAE joint program search (instantiated with $320$ development prompts across canonical batch groups \texttt{0..39}, evaluating $16 + 8\times 8 = 80$ unique candidates over Rounds~0--8).

\begin{nolinenumbers}
\begin{lpsprompt}{Prompt 1: Primary Program Search Instructions (Scale-RAE, Joint Objective)}
You are the research agent for a NEW open-code Scale-RAE loop experiment.
Use one persistent gpt-6-astra / xhigh session for the whole experiment.
Optimize GenEval, DPG and inference speed jointly on the fixed development panel using Pareto tradeoffs.
First round: 16 NEW candidates. Then 8 rounds of 8 NEW candidates, 80 total successful candidates.
Use paired feedback. Every candidate needs a
testable loop-related hypothesis. Both single and combined changes are allowed.

The old discrete action space DOES NOT APPLY. You may change the copied loop source code,
add loop methods, change schedules, steps, layers, K/lambda, guidance, token selection/reuse,
state-dependent mechanisms, and add arbitrary diagnostic code. Stay related to loop inference.
Do not change pretrained model weights, language conditions/prompts, noise/seed, precision,
AMP, batch size, decoder, output validation, timing/reporting or official scoring semantics.
Do not train, memorize prompt-specific answers, hard-code benchmark-item behavior, fetch
external weights/data, or optimize the evaluator. Use runtime features for general mechanisms.
Fixed execution: checkpoint tensor dtypes, BF16 AMP, seed42, generation/decode batch8.
Each formal candidate uses 16 warmups followed by 320 scored images, canonical batch groups.
Timing includes candidate hook setup/cleanup. Diagnostics are separate and their cost is logged.
The executor also checks 8 unchanged no-loop images before and after each formal round;
these controls are unscored and do not consume the 80 candidate slots. Preserve disabled-loop
behavior and restore cross-candidate state; a failed control invalidates the round.

You can see the SAME permitted anchors as the previous search: 25-step no-loop and paper
dense loop without LoopGuidance, measured on THIS fixed search panel. Full/held-out results,
other experiments, scorer code/target annotations, private notes, credentials and other sessions
are inaccessible. Do not try to infer or request those files.

You have native shell, file reads, apply_patch and file writes in your isolated workspace.
Use these tools directly to inspect, implement and test loop code; you do not need to ask
the coordinator to read/edit files for you. Following official OPAL, shell network access,
Web search, browser/apps/plugins and reading authentication/session files are disabled.
Model-service connectivity belongs to the transport, not your shell. No sandbox escape.
Your shell uses the supplied PyTorch interpreter on CPU, as in official OPAL. Task-specific
additions include model assets, the selected 320 conditions and a GPU diagnostic/evaluation worker.
The environment supplies python, torch, numpy and ordinary shell tools. Read-only reference
generation code is at /reference; the selected cache is /inputs/conditions.sqlite3.
Your own experiment's runtime results are read-only at /experiment_results.
You may implement arbitrary feature collectors and run local analysis scripts directly.
The managed diagnostic runner below executes your custom code on the GPU in the exact
generation pipeline, returns observations and records its cost. It is not a fixed list of
allowed features. Returned tensors/statistics can also be analyzed by your own shell scripts.
Source, notes and small results can live in this workspace; use scratch/ for large temporary
outputs. Reference inputs and official evaluation infrastructure are not editable.

Use native tools freely during each turn. End the turn with one JSON object for the
coordinator, containing experiment_id, round, rationale and ONE request below. This final
JSON schedules evaluation/diagnostics or closes the experiment; it does not restrict your
intermediate tool calls. Read/edit requests remain optional compatibility helpers.

1. Optional read-code helper (native shell reads are preferred):
{"request":"read","files":[{"path":"<loop_patch_module>","start_line":1,"line_count":250}]}
Read at most 6 files/request, up to 500 lines each. The observation includes available file names.

2. Optional edit helper (native apply_patch/shell edits are preferred):
{"request":"edit","edits":[{"path":"candidate.py","content":"complete UTF-8 Python source"}]}
Or exact replacement: {"path":"...","old":"exact existing text","new":"replacement"}.
Editable: candidate module, loop library modules, and notes.
Do not edit immutable interface/reference files. Changes are syntax checked and snapshotted.

3. Run your diagnostic code on any fixed-panel groups 0..39:
{"request":"diagnostic","batch_groups":[0],"actions":[ACTION,...],"question":"specific hypothesis"}
Use only as many samples as needed. Write results under context["output_dir"] from your
hook's close() method. Any data observed during a DiT forward is available to your custom
collector: inputs, outputs, intermediate activations, Q/K/V, attention logits/probabilities,
AdaLN/modulation values, residuals, guidance branches, token decisions, or other internal
tensors and state. These examples are not an allowlist. Add hooks or instrument the copied
code wherever necessary. You may save full tensors, e.g. .pt/.npy/.npz/.safetensors files,
and inspect them with your native shell/PyTorch tools after the worker returns. Small JSON
summaries are inlined; large JSON/tensor files are returned by path under
/experiment_results/<run_id>/diagnostics/. Message-size limits do not restrict feature
content or file size. Prefer selective capture when sufficient for iteration efficiency.
Diagnostics return real runtime artifacts plus costs; no hypothetical features.
Start by installing a lightweight DiT feature collector and requesting the no-loop and paper
anchors on group0. Confirm those images are unchanged before the first formal 16 candidates.
Then request more diagnostics whenever they can inform the next decision; there is no old
fixed feature allowlist. Full tensors are expensive: summarize meaningful norms/deltas/cosines,
attention/token statistics, guidance branches or convergence first. You may implement new probes.

4. Run this round's candidates:
{"request":"evaluate","actions":[ACTION,...],"decision_summary":"why these candidates"}
Exactly 16 actions in round0 and 8 in rounds1..8. The executor freezes the entire current code
snapshot plus every action before running. Later rounds may edit the code again. Use params to
support multiple algorithm variants in one snapshot. Never silently apply one candidate's hooks
to another. Restore overrides/hooks and reset transient state on close().

ACTION schema:
{"id":"unique_lowercase_id","step_count":10,
 "base_variant":"step25_b12-27_euler_k4_lam100_t0-50_full",
 "runtime":{"num_loops":3,"block_indices":[12,13,14,15,16,17,18,19,20,21,22,23]},
 "params":{"arbitrary_new_loop_parameter":1.2},
 "hypothesis":"mechanism and expected effect on the search objective", "changed_fields":["..."],
 "parent_id":"anchor or earlier candidate"}
base_variant supplies built-in defaults; runtime may override any existing LoopConfig field.
step_count is any positive integer, not the previous discrete list. Put NEW fields in params.
Custom code sees them via candidate.configure(model, params, context). Return None or an object
with close(). configure() is called once per generation batch after built-in loop patching;
the returned handle is closed after inference. context contains step_count, variant, diagnostic,
output_dir. Calls execute under the existing AMP context. You can also modify the loop modules
directly. Your hooks must not disable AMP or mutate fixed dtype/weight policies.

5. After all rounds:
{"request":"finish","summary":"quality, speed and balanced representatives, evidence, limitations"}

If an executor defect outside your editable code prevents progress, return
{"request":"blocked","reason":"exact failure and required runtime repair"}.
The coordinator will retain this session without claiming completion or forcing more
GPU/model-call retries. Do not resubmit an unchanged infrastructure failure repeatedly.

Always identify expected changes, observed evidence, failures and uncertainty. Missing results
are not zeros. Do not call the development subset a held-out test. Do not assert significance
from overlapping confidence intervals or repeated adaptive selection. Avoid repeated identical
code+effective configurations. Failures return observations and may be repaired; do not pretend
they succeeded. Input/output tokens, public responses/reasoning summaries, requests, code diffs,
configuration/source hashes, GPU metrics and wall times are recorded. Hidden reasoning is not
requested or exported. Prioritize GPU iteration efficiency.
\end{lpsprompt}
\end{nolinenumbers}

\subsection{Per-Turn Observation Payload}
\label{sec:supp_prompt_observation}

On every turn, the coordinator serializes the current experiment state into a structured JSON observation payload and passes it as the user message. Single-objective runs replace \texttt{pareto} with \texttt{best\_geneval} or \texttt{best\_dpg}, and no-diagnostics runs withhold \texttt{worker\_log\_tail} on infrastructure failures. Prompt~2 shows the canonical JSON turn payload at Round~0 initialization together with the \texttt{feedback} fields updated after subsequent \texttt{diagnostic} and \texttt{evaluate} turns.

\begin{nolinenumbers}
\begin{lpsprompt}{Prompt 2: Per-Turn Observation JSON Schema and Round-0 Initialization Payload}
{
  "protocol": {
    "experiment_id": "<run_id>",
    "agent_backend": "codex",
    "model": "gpt-6-astra",
    "effort": "xhigh",
    "round_sizes": [16, 8, 8, 8, 8, 8, 8, 8, 8],
    "batch_size": 8,
    "amp": "bf16",
    "precision": "checkpoint_actual",
    "seed": 42,
    "search_prompts": 320,
    "scored_splits": ["geneval", "dpg"],
    "diagnostics_enabled": true,
    "objectives": ["geneval", "dpg", "speed_ratio"],
    "action_space": "unrestricted_loop_code_and_configuration",
    "anchors": ["step25_disabled", "step25_b12-27_euler_k4_lam100_t0-50_full"],
    "anchor_run": "<anchor_run_id>",
    "synthetic_anchor_tier": null,
    "held_out_access": false,
    "old_experiment_access": false,
    "evaluator_access": false,
    "panel_sha256": "<sha256_of_320_prompt_manifest>"
  },
  "round": 0,
  "available_trial_slots": 16,
  "files": [["<candidate_module>", "<sha256>"], ["<loop_patch_module>", "<sha256>"], "..."],
  "trials": [
    {"variant": "step25_disabled", "run_id": "<anchor_run_id>",
     "geneval": 0.5380, "dpg": 0.7755, "seconds_per_image": 0.2828, "speed_ratio": 1.0000},
    {"variant": "step25_b12-27_euler_k4_lam100_t0-50_full", "run_id": "<anchor_run_id>",
     "geneval": 0.5988, "dpg": 0.7970, "seconds_per_image": 0.5042, "speed_ratio": 0.5609}
  ],
  "pareto": ["step25_disabled", "step25_b12-27_euler_k4_lam100_t0-50_full"],
  "feature_chain_verified": false,
  "completed_rounds": [],
  "feedback": {
    "phase": "initialize",
    "anchors": {"...": "subtask/domain scores and timing for measured anchors on dev split"},
    "instruction": "Read needed loop code, implement an informative lightweight feature collector, request both anchors on group0; then propose 16 new candidates."
  }
}

// After a "diagnostic" request:
//   feedback = {"both_anchors_exact": true, "artifacts": {...}, "artifact_files": [...], "cost": {...}}
//   (when both_anchors_exact && non-empty artifacts, feature_chain_verified becomes true)
// After an "evaluate" request completes Round r:
//   completed_rounds.append({"round": r, "run_id": "<id>", "configs": N, "code_revision": "<sha256>", "joint_hypervolume_increment": <delta_hv>})
//   feedback = {
//     "last_round": {"trials": [...], "comparisons": {"vs_baseline": {...}, "vs_paper": {...}}, "subtask_breakdowns": {...}},
//     "instruction": "Iterate on the loop code/configuration using evidence; diagnose when useful. Finish only after all 9 rounds."
//   }
\end{lpsprompt}
\end{nolinenumbers}

\subsection{Backbone and Ablation Prompt Adaptations}
\label{sec:supp_prompt_adaptations}

Prompts~3a--3c record the RQ2 ablations (Table~\ref{tab:agent_pareto}, Figure~\ref{fig:teaser}e, and Table~\ref{tab:rae_synthetic_target_ablation}) and Prompt~4d records the supplementary initial-search-context ablation (Section~\ref{sec:supp_context_ablation}, Table~\ref{tab:memflow_context}); Prompts~4a--4c record the backbone-specific instructions for the remaining image, text-reasoning, and video architectures in RQ1, RQ3, and RQ4.

\begin{nolinenumbers}
\begin{lpsprompt}{Prompt 3a: \papershort{} w/o Diagnostics Adaptation (RQ2)}
Diagnostics are disabled. Submit formal candidates directly. Do not run exploratory
model forwards, add instrumentation to collect activations or internal statistics,
or try to recover worker logs or artifacts. Static code inspection and CPU unit tests
of your inference code are available. Candidate inference may use its internal state
to compute its output within the forward pass. The evaluator returns formal benchmark
feedback only.
\end{lpsprompt}
\end{nolinenumbers}

Prompt~3a replaces lines~60--76 (\texttt{diagnostic} interface) in Prompt~1 and omits \texttt{feature\_chain\_verified} checks, while retaining the identical 9-round, 80-candidate budget and editable loop source rules. Prompt~3b shows the coordinator substitutions for the two single-objective runs (GenEval-only and DPG-only) and the anchor blocks distinguishing the \texttt{Gemini-4-Argon} search-target calibration runs (True, Strong, and Ultra).

\begin{nolinenumbers}
\begin{lpsprompt}{Prompt 3b: Single-Objective and Search-Target Calibration Adaptations (RQ2)}
--- Variant A: GenEval-only search ($search_prompts = 112, $last_group = 13) ---
$objective := Maximize official GenEval overall (equal-task macro mean) on the fixed GenEval development panel. GenEval is the sole selection objective. Inference timing is reported as telemetry.
$final_summary := top GenEval programs, evidence, limitations

--- Variant B: DPG-only search ($search_prompts = 208, $last_group = 25) ---
$objective := Maximize official DPG-Bench overall (mean official per-prompt score) on the fixed DPG-Bench development panel. DPG-Bench is the sole selection objective. Inference timing is reported as telemetry.
$final_summary := top DPG-Bench programs, evidence, limitations

--- Variant C: Search-target anchor blocks (Gemini-4-Argon, 320-prompt dev panel) ---
[True target (2 anchors):]
1. step25_disabled: 25-step no-loop baseline (GenEval=0.5380, DPG=0.7755, 0.2828 s/img, speed_ratio=1.0000).
2. step25_b12-27_euler_k4_lam100_t0-50_full: 25-step paper dense loop without LoopGuidance
   (GenEval=0.5988, DPG=0.7970, 0.5042 s/img, speed_ratio=0.5609).

[Strong target (3 anchors, target strength +17.86%):]
3. step20_open_ref_strong_loop: 20-step strong reference loop baseline
   (GenEval=0.6517, DPG=0.8121, 0.3535 s/img, speed_ratio=0.8000).

[Ultra target (3 anchors, target strength +29.28%):]
3. step18_open_ref_ultra_loop: 18-step strong reference loop baseline
   (GenEval=0.7131, DPG=0.8326, 0.3074 s/img, speed_ratio=0.9200).
NOTE: For the initial group0 diagnostic verification (both_anchors_exact), still request the two
built-in physical anchors (base_variant="step25_disabled" and
base_variant="step25_b12-27_euler_k4_lam100_t0-50_full", both with step_count=25 and no runtime
overrides) so the coordinator can verify exact byte preservation against the physical reference images.
\end{lpsprompt}
\end{nolinenumbers}

For Configuration Search (RQ2), the session prompt locks the Scale-RAE weights, $320$-prompt panel, $9$-round schedule ($16 + 8\times 8 = 80$ candidates), and BF16 AMP settings, but prohibits shell access, file edits, and custom feature hooks. Instead, proposals are restricted to the fixed discrete action grid and JSON response schema in Prompt~3c, with fixed \texttt{dit\_features} summary queries capped at $\le 2$ diagnostic calls per round after initial anchor parity verification.

\begin{nolinenumbers}
\begin{lpsprompt}{Prompt 3c: Configuration-Search Discrete Action Space and JSON Turn Schema (RQ2)}
--- Permitted discrete action space (28 loopable DiT blocks 0..27; loop_operator="euler") ---
step_count: [10, 15, 20, 25, 30]
layer_start: [8, 10, 12, 14, 16, 18, 20, 22, 24, "all"]
layer_count: [4, 8, 12, 16]   # null when layer_start="all" (expands to b0-27)
k: [2, 3, 4, 6, 8]
total_lambda_pct: 100
loop_schedule: ["t0-30", "t0-40", "t0-50", "t0-60", "t0-75"]
token_operator: ["full", "abaCB"]
selector: ["r", "rt", "adaln", "aorwn"]   # required for abaCB; null for full
aratio_pct: [50, 70, 85]   # required for abaCB; null for full
loop_guidance: ["off", 1.5, 2.0, 2.8, 4.0, 6.0, 9.0]

--- Strict JSON-only turn response schema (no shell or file editing; <= 2 fixed probes/round) ---
{
  "experiment_id": "<run_id>",
  "round": 0,
  "analysis_summary": "...",
  "diagnostics": [{"type": "dit_features", "variants": ["known_variant"],
                   "layers": [12, 20], "steps": [0, 6, 12], "batch_groups": [0], "hypothesis": "..."}],
  "next_actions": [{"variant": "<variant_grammar>", "parent_variant": "<id_or_null>",
                    "role": "improvement|exploration|control", "changed_fields": ["..."],
                    "hypothesis": "...", "decision_rationale": "..."}],
  "hypothesis_register_updates": [],
  "final_summary": ""
}
\end{lpsprompt}
\end{nolinenumbers}

Prompt~4a gives the image-backbone adaptations to Prompt~1.

\begin{nolinenumbers}
\begin{lpsprompt}{Prompt 4a: RAE (615M DDT) and Looped-DiT-B32 Backbone Protocols (RQ1)}
--- RAE-SigLIP2-B/DDT 615M (GPT-6-Astra, 320-prompt dev panel) ---
The permitted anchors are measured on THIS search panel: 50-step no-loop, paper Dense Loop,
and paper Dense LoopGuidance9. The paper loop uses encoder blocks 15..22, K4, total strength 1,
layerwise Euler residuals and sampling progress [0,0.5]. CFG is disabled; output is 256x256.
The model has 28 encoder blocks processing 256 image + 4 time + 256 text tokens, then 2 decoder blocks.

candidate.configure(model,params,context), called once per generation batch AFTER the built-in loop patch.
Return None or a handle with close(). The handle may also expose model_fn to wrap context['model_fn'].

--- Looped-DiT-B32 (Gemini-4-Argon, 320-prompt dev panel, 4 measured native anchors) ---
- Model: sensenova/Looped-DiT-B32 (LoopedMMDiT, 512x512 pixel-space flow-matching MMDiT,
  patch_size=32, 16x16=256 image tokens, 256 FLAN-T5-large text tokens, 2 text preamble blocks,
  loop_split=(6, 5, 6) pre/core/post DoubleStreamBlocks, trained with num_loops=4 and deep supervision).
- Checkpoint dtype: BF16 EMA weights with BF16 CUDA autocast; noise_scale=2.0, official cfg_scale=6.0,
  samples_per_prompt=4, prompt_batch_size=16 (effective image batch = 64, fused CFG batch = 128).
- 4 initial anchors: steps100_loops4, steps50_loops4, steps25_loops4, steps100_loops1.
- Custom sampler hook: optional handle.sample_batch(model, text, text_mask, x_init, *, step_count,
  cfg_scale, num_loops, context) -> Tensor returning [B, 3, 512, 512] in [-1, 1]; step_count in 1..200,
  runtime.num_loops in 1..32; Pareto HV over (geneval, dpg, min(t_steps100_loops4 / t_candidate, 8.0)).
\end{lpsprompt}
\end{nolinenumbers}

Prompt~4b specifies Qwen3-4B's quality-only objective and mandatory recurrence. The target-calibration ablation in Table~\ref{tab:llm_pressure_ablation} shifts the paper-anchor \texttt{acc\_norm} target by $+1.57$, $+3.02$, or $+6.03$ percentage points without changing these rules.

\begin{nolinenumbers}
\begin{lpsprompt}{Prompt 4b: Autoregressive Text Reasoning Instructions (Qwen3-4B, RQ4)}
You are the research agent for an open-code training-free LLM loop experiment on Qwen/Qwen3-4B (Qwen3-4B-Instruct, 36 decoder layers 0..35).
Use this one persistent session for all rounds on the frozen 829-question (20%) multi-task zero-shot multiple-choice loglikelihood search panel:
- mmlu_hard_stem (10 subjects, 305 questions)
- sciq (200 questions)
- arc_challenge (234 questions)
- gpqa_main (Biology, Chemistry, Physics, 90 questions)

The two initial anchors are:
1. "baseline": unmodified Qwen/Qwen3-4B (loop_config: null)
2. "paper": paper Euler loop at inclusive zero-based layers [15, 18], num_loops=3, strategy="euler", iteration_mode="block", cache_strategy="first", decode_mode="full"
Anchors do not consume candidate slots.

CRITICAL OPTIMIZATION OBJECTIVE -- QUALITY ONLY (TIME IS NOT INCLUDED):
- Inference time / latency is NOT part of the optimization objective (optimization_objective = "quality_only_no_time").
- Timing fields are intentionally excluded from the trial observations, and there is NO accuracy-vs-time hypervolume or latency penalty.
- Do NOT propose reduced-loop, shallow, or early-exit candidates merely to save inference time.
- Optimize prediction quality purely across: acc_norm, accuracy, macro_group_accuracy, margin_score, logprob_score.

OPEN-CODE ALGORITHM FREEDOM & MANDATORY LOOP REQUIREMENT (require_loop = true):
- You may edit the candidate module, loop library modules, and notes.
- EVERY formal candidate MUST contain a real, substantive loop that repeatedly applies a transformer layer, window, or model-derived operator to an evolving hidden state, and the iterated result must contribute to the returned hidden states/logits.
- Pure layer skipping/pruning, single-pass depth changes, static residual scaling without recurrence, or dummy discarded loops are ineligible.
- Every evaluate action MUST include a "loop_mechanism" object:
  {"operator": "...", "state_update": "...", "output_dependency": "...", "scope": "..."}
- Original decoder layer/submodule forwards are observed automatically by the loop audit. For a custom functional loop body that bypasses original module forwards, wrap its substantive loop body via context['loop_trace']('body_name', body_callable) during configure and call the returned callable each iteration.
\end{lpsprompt}
\end{nolinenumbers}

Prompt~4c specifies the residual-strength and architecture-specific causal-cache contracts for video search.

\begin{nolinenumbers}
\begin{lpsprompt}{Prompt 4c: Video Diffusion Loop Contracts (Wan2.1-1.3B, Self-Forcing 1.3B, LongLive 1.0/2.0, RQ3)}
--- Wan2.1-1.3B Short Video (unit-sum residual rule) ---
Total loop residual lambda is FIXED at 1 (strength=1, total_lambda_pct=100). Each of K equal residual
substeps uses 1/K. Unequal/adaptive executed residual weights must still sum to 1 for every enabled
loop. Do not change total lambda via per-layer/per-step scaling or early stopping. LoopGuidance is a
separate coefficient, not residual lambda. Include a concise lambda_contract explaining the executed
coefficient sum with every evaluate request; code is retained for protocol review.

--- Self-Forcing 1.3B Causal Chunked Video (pure AST-checked loop API + KV transaction) ---
Implement:
  def loop(x, evaluate, info, params, memory):
      ...
      return {"residuals": [r0, r1, ...], "weights": [w0, w1, ...]}
Only imports torch and math are allowed. Weights must be finite scalar numbers summing to 1 (lambda=1);
negative coefficients are allowed for LoopGuidance or secant corrections (magnitude <= 8). Self/block
repeated evaluations use a cache transaction: the first evaluation commits native current-chunk K/V;
subsequent refinement evaluations restore that committed slice and indices. Clean-context refresh always
runs the native model through all 30 layers; it is never looped, skipped or approximated.

--- LongLive 1.0 1.3B / 2.0 5B RememBench (20 dev scenes; 80 candidates) ---
Propose recurrent loop programs over the 30-layer causal denoiser to improve departure-to-revisit
consistency (maximizing mean CLIP and minimizing mean LPIPS) on the frozen 20-scene development split.
Loop either individual layers (layerwise) or a contiguous sequence of layers (windowwise) for K in
2..8 passes, applying unit-budget Euler updates x_next = x + (F(x) - x) / K across selected denoising
steps (0..3) and autoregressive chunks (0..11 for 2.0; 0..31 for 1.0). Defer causal KV-cache commits
to the final logical pass of each physical layer, and leave native clean-context refreshes unmodified.
On-demand read-only diagnostics may probe layer activations, residuals, alignment, repeat dynamics,
and KV boundaries between rounds without consuming candidate slots.
\end{lpsprompt}
\end{nolinenumbers}

Prompt~4d summarizes the shared search specification and the two initial-context factors (algorithmic guidance and starter operator library) used in the $2{\times}2$ ablation on $60$\,s multi-prompt LongLive~2.0~5B (Table~\ref{tab:memflow_context}, Section~\ref{sec:supp_context_ablation}).

\begin{nolinenumbers}
\begin{lpsprompt}{Prompt 4d: 60s Multi-Prompt Video Initial Search Context Ablation (LongLive 2.0 5B, Sec. C.5)}
--- Shared specification across all 4 regimes (Gemini-4-Argon high, 4 rounds x 8 = 32 candidates) ---
Backbone: LongLive-2.0-5B (30 causal layers), 45 chunks x 8 latent frames (1,437 frames at 24 fps,
59.875s), 6 successive 10s prompt segments, native 4-step UniPC denoising.
Objectives: 5D Pareto optimization over normalized VBench-Long Quality, Consistency, mean CLIP ViT-L/14,
worst-segment CLIP shift, and speed ratio on the frozen 20-video development split, with up to 2
read-only diagnostic probes per round.
Validity: Every candidate must implement genuine transformer loop recurrence (repeated block or sublayer
passes inside denoising) with frozen weights, unmodified kernels, and verified baseline equivalence.

--- Factor 1: Algorithmic guidance (Minimal / Library only vs. Guidance only / Matched prior) ---
[Without Guidance]:
  Neutral task instructions requesting genuine transformer loop recurrence and strictly algorithmic
  efficiency improvements, with Round-0 diagnostics checking unmodified baseline behavior.
[With Guidance]:
  Names candidate loop forms (block, window, sublayer, or predictor loops) and algorithmic efficiency
  mechanisms (loop-compensated step reduction, selective token looping, adaptive step/layer/chunk
  scheduling, and cached residual reuse), and encourages Round-0 diagnostics to profile layer, chunk,
  and step dynamics.

--- Factor 2: Starter operator library (Minimal / Guidance only vs. Library only / Matched prior) ---
[Without Library]:
  Starts from an empty program template; the search LLM designs and implements loop operators and
  parameterizations from scratch.
[With Library]:
  Pre-populates editable starter operators adapted from our image-diffusion experiments: ODE integrators
  (Euler, Heun, Midpoint), masked and alternating token-update schedules, token-importance selectors,
  and reusable block/window loop primitives, all freely modifiable or replaceable.
\end{lpsprompt}
\end{nolinenumbers}
