# Supplementary material for: Evolving Loop Programs: Discovering How Frozen Transformers Should Loop
Source: arXiv:2611.41108 source file (2026-12-03)
Supplement: Supplementary file 11 [file appendix_references.tex]

\section*{Supplementary References}
\addcontentsline{toc}{section}{Supplementary References}
\begingroup
\small
\setlength{\parskip}{2.5pt}
\setlength{\parindent}{0pt}
\newcommand{\suppbibentry}[3]{%
  \par\goodbreak\begingroup\interlinepenalty=10000\noindent\hangindent=2.5em\hangafter=1%
  \makebox[2.5em][l]{[{#1}]}\phantomsection\label{suppbib:#2}\ignorespaces#3\par\endgroup}

\suppbibentry{S1}{fishman2026dory}{%
Maxim Fishman, Simeng Sun, Shantanu Acharya, Faisal Ladhak, Brian Chmiel, Santiago~Akle Serano, Ron Banner, Boris Ginsburg, and Krishna~C. Puvvada.
\newblock {Dory1.0-4B}: A looped normalized-{GPT}.
\newblock \emph{arXiv preprint arXiv:2611.03998}, 2026.}

\suppbibentry{S2}{pyatkin2025ifbench}{%
Valentina Pyatkin, Saumya Malik, Victoria Graf, Hamish Ivison, Shengyi Huang, Pradeep Dasigi, Nathan Lambert, and Hannaneh Hajishirzi.
\newblock Generalizing verifiable instruction following.
\newblock In \emph{NeurIPS Datasets and Benchmarks}, 2025.}

\suppbibentry{S3}{tian2024scicode}{%
Minyang Tian, Luyu Gao, Shizhuo~Dylan Zhang, et~al.
\newblock {SciCode}: A research coding benchmark curated by scientists.
\newblock \emph{arXiv preprint arXiv:2407.13168}, 2024.}

\suppbibentry{S4}{bae2025relaxed}{%
Sangmin Bae, Adam Fisch, Hrayr Harutyunyan, Ziwei Ji, Seungyeon Kim, and Tal Schuster.
\newblock Relaxed recursive transformers: Effective parameter sharing with layer-wise {LoRA}.
\newblock In \emph{ICLR}, 2025.}

\suppbibentry{S5}{bai2019deq}{%
Shaojie Bai, J.~Zico Kolter, and Vladlen Koltun.
\newblock Deep equilibrium models.
\newblock In \emph{NeurIPS}, 2019.}

\suppbibentry{S6}{banino2021pondernet}{%
Andrea Banino, Jan Balaguer, and Charles Blundell.
\newblock {PonderNet}: Learning to ponder.
\newblock \emph{arXiv preprint arXiv:2107.05407}, 2021.}

\suppbibentry{S7}{chen2024diffusionforcing}{%
Boyuan Chen, Diego Mart{\'\i}~Mons{\'o}, Yilun Du, Max Simchowitz, Russ Tedrake, and Vincent Sitzmann.
\newblock Diffusion forcing: Next-token prediction meets full-sequence diffusion.
\newblock In \emph{NeurIPS}, 2024.}

\suppbibentry{S8}{chen2018neuralode}{%
Ricky T.~Q. Chen, Yulia Rubanova, Jesse Bettencourt, and David Duvenaud.
\newblock Neural ordinary differential equations.
\newblock In \emph{NeurIPS}, 2018.}

\suppbibentry{S9}{chen2025itt}{%
Yilong Chen, Junyuan Shang, Zhenyu Zhang, Yanxi Xie, Jiawei Sheng, Tingwen Liu, Shuohuan Wang, Yu Sun, Hua Wu, and Haifeng Wang.
\newblock Inner thinking transformer: Leveraging dynamic depth scaling to foster adaptive internal thinking.
\newblock In \emph{ACL}, 2025.}

\suppbibentry{S10}{deepseek2025r1}{%
{DeepSeek-AI}, Daya Guo, Dejian Yang, Haowei Zhang, Junxiao Song, et~al.
\newblock {DeepSeek-R1}: Incentivizing reasoning capability in {LLMs} via reinforcement learning.
\newblock \emph{arXiv preprint arXiv:2501.12948}, 2025.}

\suppbibentry{S11}{elhoushi2024layerskip}{%
Mostafa Elhoushi, Akshat Shrivastava, Diana Liskovich, Basil Hosmer, Bram Wasti, Liangzhen Lai, Anas Mahmoud, Bilge Acun, Saurabh Agarwal, Ahmed Roman, Ahmed~A. Aly, Beidi Chen, and Carole-Jean Wu.
\newblock {LayerSkip}: Enabling early exit inference and self-speculative decoding.
\newblock In \emph{ACL}, 2024.}

\suppbibentry{S12}{fan2025lengthgen}{%
Ying Fan, Yilun Du, Kannan Ramchandran, and Kangwook Lee.
\newblock Looped transformers for length generalization.
\newblock In \emph{ICLR}, 2025.}

\suppbibentry{S13}{gatmiry2024loopedgd}{%
Khashayar Gatmiry, Nikunj Saunshi, Sashank~J. Reddi, Stefanie Jegelka, and Sanjiv Kumar.
\newblock Can looped transformers learn to implement multi-step gradient descent for in-context learning?
\newblock In \emph{ICML}, 2024.}

\suppbibentry{S14}{giannou2023looped}{%
Angeliki Giannou, Shashank Rajput, Jy-Yong Sohn, Kangwook Lee, Jason~D. Lee, and Dimitris Papailiopoulos.
\newblock Looped transformers as programmable computers.
\newblock In \emph{ICML}, 2023.}

\suppbibentry{S15}{graves2016act}{%
Alex Graves.
\newblock Adaptive computation time for recurrent neural networks.
\newblock \emph{arXiv preprint arXiv:1603.08983}, 2016.}

\suppbibentry{S16}{hao2025coconut}{%
Shibo Hao, Sainbayar Sukhbaatar, DiJia Su, Xian Li, Zhiting Hu, Jason~E. Weston, and Yuandong Tian.
\newblock Training large language models to reason in a continuous latent space.
\newblock In \emph{COLM}, 2025.}

\suppbibentry{S17}{hu2025adas}{%
Shengran Hu, Cong Lu, and Jeff Clune.
\newblock Automated design of agentic systems.
\newblock In \emph{ICLR}, 2025.}

\suppbibentry{S18}{lan2020albert}{%
Zhenzhong Lan, Mingda Chen, Sebastian Goodman, Kevin Gimpel, Piyush Sharma, and Radu Soricut.
\newblock {ALBERT}: A lite {BERT} for self-supervised learning of language representations.
\newblock In \emph{ICLR}, 2020.}

\suppbibentry{S19}{liu2025teacache}{%
Feng Liu, Shiwei Zhang, Xiaofeng Wang, Yujie Wei, Haonan Qiu, Yuzhong Zhao, Yingya Zhang, Qixiang Ye, and Fang Wan.
\newblock Timestep embedding tells: It's time to cache for video diffusion model.
\newblock In \emph{CVPR}, 2025.}

\suppbibentry{S20}{liu2019darts}{%
Hanxiao Liu, Karen Simonyan, and Yiming Yang.
\newblock {DARTS}: Differentiable architecture search.
\newblock In \emph{ICLR}, 2019.}

\suppbibentry{S21}{liu2025taylorseer}{%
Jiacheng Liu, Chang Zou, Yuanhuiyi Lyu, Junjie Chen, and Linfeng Zhang.
\newblock From reusing to forecasting: Accelerating diffusion models with {TaylorSeers}.
\newblock In \emph{ICCV}, 2025.}

\suppbibentry{S22}{lu2022dpmsolver}{%
Cheng Lu, Yuhao Zhou, Fan Bao, Jianfei Chen, Chongxuan Li, and Jun Zhu.
\newblock {DPM-Solver}: A fast {ODE} solver for diffusion probabilistic model sampling in around 10 steps.
\newblock In \emph{NeurIPS}, 2022.}

\suppbibentry{S23}{ma2025scalingdiff}{%
Nanye Ma, Shangyuan Tong, Haolin Jia, Hexiang Hu, Yu-Chuan Su, Mingda Zhang, Xuan Yang, Yandong Li, Tommi Jaakkola, Xuhui Jia, and Saining Xie.
\newblock Inference-time scaling for diffusion models beyond scaling denoising steps.
\newblock In \emph{CVPR}, 2025.}

\suppbibentry{S24}{ma2024deepcache}{%
Xinyin Ma, Gongfan Fang, and Xinchao Wang.
\newblock {DeepCache}: Accelerating diffusion models for free.
\newblock In \emph{CVPR}, 2024.}

\suppbibentry{S25}{raposo2024mod}{%
David Raposo, Sam Ritter, Blake Richards, Timothy Lillicrap, Peter~Conway Humphreys, and Adam Santoro.
\newblock Mixture-of-depths: Dynamically allocating compute in transformer-based language models.
\newblock \emph{arXiv preprint arXiv:2404.02258}, 2024.}

\suppbibentry{S26}{schuster2022calm}{%
Tal Schuster, Adam Fisch, Jai Gupta, Mostafa Dehghani, Dara Bahri, Vinh~Q. Tran, Yi Tay, and Donald Metzler.
\newblock Confident adaptive language modeling.
\newblock In \emph{NeurIPS}, 2022.}

\suppbibentry{S27}{snell2025testtime}{%
Charlie Snell, Jaehoon Lee, Kelvin Xu, and Aviral Kumar.
\newblock Scaling {LLM} test-time compute optimally can be more effective than scaling parameters for reasoning.
\newblock In \emph{ICLR}, 2025.}

\suppbibentry{S28}{song2025history}{%
Kiwhan Song, Boyuan Chen, Max Simchowitz, Yilun Du, Russ Tedrake, and Vincent Sitzmann.
\newblock History-guided video diffusion.
\newblock In \emph{ICML}, 2025.}

\suppbibentry{S29}{wei2022cot}{%
Jason Wei, Xuezhi Wang, Dale Schuurmans, Maarten Bosma, Brian Ichter, Fei Xia, Ed Chi, Quoc~V. Le, and Denny Zhou.
\newblock Chain-of-thought prompting elicits reasoning in large language models.
\newblock In \emph{NeurIPS}, 2022.}

\suppbibentry{S30}{yang2024looped}{%
Liu Yang, Kangwook Lee, Robert~D. Nowak, and Dimitris Papailiopoulos.
\newblock Looped transformers are better at learning learning algorithms.
\newblock In \emph{ICLR}, 2024.}

\suppbibentry{S31}{yin2025causvid}{%
Tianwei Yin, Qiang Zhang, Richard Zhang, William~T. Freeman, Fr{\'e}do Durand, Eli Shechtman, and Xun Huang.
\newblock From slow bidirectional to fast autoregressive video diffusion models.
\newblock In \emph{CVPR}, 2025.}

\suppbibentry{S32}{zhao2023unipc}{%
Wenliang Zhao, Lujia Bai, Yongming Rao, Jie Zhou, and Jiwen Lu.
\newblock {UniPC}: A unified predictor-corrector framework for fast sampling of diffusion models.
\newblock In \emph{NeurIPS}, 2023.}

\suppbibentry{S33}{balaji2022ediffi}{%
Yogesh Balaji, Seungjun Nah, Xun Huang, Arash Vahdat, Jiaming Song, Qinsheng Zhang, Karsten Kreis, Miika Aittala, Timo Aila, Samuli Laine, Bryan Catanzaro, Tero Karras, and Ming-Yu Liu.
\newblock {eDiff-I}: Text-to-image diffusion models with an ensemble of expert denoisers.
\newblock \emph{arXiv preprint arXiv:2211.01324}, 2022.}

\suppbibentry{S34}{chen2024gits}{%
Defang Chen, Zhenyu Zhou, Can Wang, Chunhua Shen, and Siwei Lyu.
\newblock On the trajectory regularity of {ODE}-based diffusion sampling.
\newblock In \emph{ICML}, 2024.}

\suppbibentry{S35}{choi2022p2}{%
Jooyoung Choi, Jungbeom Lee, Chaehun Shin, Sungwon Kim, Hyunwoo Kim, and Sungroh Yoon.
\newblock Perception prioritized training of diffusion models.
\newblock In \emph{CVPR}, 2022.}

\suppbibentry{S36}{esser2024sd3}{%
Patrick Esser, Sumith Kulal, Andreas Blattmann, Rahim Entezari, Jonas M{\"u}ller, Harry Saini, Yam Levi, Dominik Lorenz, Axel Sauer, Frederic Boesel, Dustin Podell, Tim Dockhorn, Zion English, Kyle Lacey, Alex Goodwin, Yannik Marek, and Robin Rombach.
\newblock Scaling rectified flow transformers for high-resolution image synthesis.
\newblock In \emph{ICML}, 2024.}

\suppbibentry{S37}{gurnee2026workspace}{%
Wes Gurnee, Nicholas~J. Sofroniew, Adam Pearce, Mateusz Piotrowski, Isaac Kauvar, Run-Jin Chen, Anna Soligo, Paul~C. Bogdan, Euan Ong, Rowan Wang, Ben Thompson, David Abrahams, Subhash Kantamneni, Emmanuel Ameisen, Joshua Batson, and Jack Lindsey.
\newblock Verbalizable representations form a global workspace in language models.
\newblock \emph{arXiv preprint arXiv:2607.15495}, 2026.}

\suppbibentry{S38}{kynkaanniemi2024interval}{%
Tuomas Kynk{\"a}{\"a}nniemi, Miika Aittala, Tero Karras, Samuli Laine, Timo Aila, and Jaakko Lehtinen.
\newblock Applying guidance in a limited interval improves sample and distribution quality in diffusion models.
\newblock In \emph{NeurIPS}, 2024.}

\suppbibentry{S39}{liu2022pndm}{%
Luping Liu, Yi Ren, Zhijie Lin, and Zhou Zhao.
\newblock Pseudo numerical methods for diffusion models on manifolds.
\newblock In \emph{ICLR}, 2022.}

\suppbibentry{S40}{loshchilov2025ngpt}{%
Ilya Loshchilov, Cheng-Ping Hsieh, Simeng Sun, and Boris Ginsburg.
\newblock {nGPT}: Normalized transformer with representation learning on the hypersphere.
\newblock In \emph{ICLR}, 2025.}

\suppbibentry{S41}{lv2025fastercache}{%
Zhengyao Lv, Chenyang Si, Junhao Song, Zhenyu Yang, Yu Qiao, Ziwei Liu, and Kwan-Yee~K. Wong.
\newblock {FasterCache}: Training-free video diffusion model acceleration with high quality.
\newblock In \emph{ICLR}, 2025.}

\suppbibentry{S42}{sabour2024ays}{%
Amirmojtaba Sabour, Sanja Fidler, and Karsten Kreis.
\newblock Align your steps: Optimizing sampling schedules in diffusion models.
\newblock In \emph{ICML}, 2024.}

\suppbibentry{S43}{skean2025layer}{%
Oscar Skean, Md~Rifat Arefin, Dan Zhao, Niket Patel, Jalal Naghiyev, Yann LeCun, and Ravid Shwartz-Ziv.
\newblock Layer by layer: Uncovering hidden representations in language models.
\newblock In \emph{ICML}, 2025.}

\suppbibentry{S44}{sun2025painters}{%
Qi Sun, Marc Pickett, Aakash~Kumar Nain, and Llion Jones.
\newblock Transformer layers as painters.
\newblock In \emph{AAAI}, 2025.}

\suppbibentry{S45}{tml2026inkling2}{%
{Thinking Machines Lab}.
\newblock Inkling 2 {Mini}.
\newblock Technical blog / model release, Nov.\ 2026.}

\suppbibentry{S46}{vendrell2026melt}{%
Victor~Conchello Vendrell, Arnau~Padres Masdemont, Niccol{\`o} Grillo, Jordi Ros-Giralt, Arash Behboodi, and Fabio~Valerio Massoli.
\newblock Memory-efficient looped transformer: Decoupling compute from memory in looped language models.
\newblock \emph{arXiv preprint arXiv:2605.07721}, 2026.}

\suppbibentry{S47}{yang2026flashloop}{%
Wanqi Yang and Shiwei Liu.
\newblock {FlashLoop}: Fast and memory-efficient looped transformers via lazy updates.
\newblock \emph{arXiv preprint arXiv:2609.29812}, 2026.}

\suppbibentry{S48}{zhao2025pab}{%
Xuanlei Zhao, Xiaolong Jin, Kai Wang, and Yang You.
\newblock Real-time video generation with pyramid attention broadcast.
\newblock In \emph{ICLR}, 2025.}

\suppbibentry{S49}{ji2025memflow}{%
Sihui Ji, Xi Chen, Shuai Yang, Xin Tao, Pengfei Wan, and Hengshuang Zhao.
\newblock {MemFlow}: Flowing adaptive memory for consistent and efficient long video narratives.
\newblock \emph{arXiv preprint arXiv:2512.14699}, 2025.}
\endgroup
