# Supplementary material for: Evolving Loop Programs: Discovering How Frozen Transformers Should Loop
Source: arXiv:2611.41108 source file (2026-12-03)
Supplement: Supplementary file 12 [file appendix_related_work.tex]

\section{Extended Related Work}
\label{sec:supp_related_work}

This section expands Section~2 of the main paper with a broader synthesis of looped-transformer foundations, dynamic depth architectures, inference-time compute scaling and caching, autoregressive video rollouts, and LLM-guided algorithm discovery.

\subsection{Looped Transformers, Weight Sharing, and Latent Recurrent Depth}
\label{sec:supp_rw_looped}

\paragraph{Foundations of weight tying and continuous computation.}
Increasing effective depth without growing parameter counts traces back to recurrent and adaptive computation in sequence models. Adaptive Computation Time~(ACT)~\citesupp{graves2016act} equips recurrent networks with a learned halting unit to execute variable numbers of transition steps per input, while PonderNet~\citesupp{banino2021pondernet} reformulates adaptive halting as a probabilistic geometric process with unbiased low-variance gradient estimators. Within Transformer architectures, Universal Transformers~\cite{dehghani2019universal} replace distinct layers with a shared parallel-in-time recurrent block paired with dynamic halting, and ALBERT~\citesupp{lan2020albert} demonstrates that cross-layer parameter sharing substantially shrinks encoder memory while preserving downstream accuracy. Pushing parameter tying to the infinite-depth limit, Deep Equilibrium Models~(DEQ)~\citesupp{bai2019deq} bypass fixed unrolling during training by solving directly for a fixed-point representation $\mathbf{z}^{\star} = f_{\theta}(\mathbf{z}^{\star}, \mathbf{x})$ via root-finding and differentiating through the equilibrium point via implicit differentiation. Complementing discrete equilibrium formulations, Neural Ordinary Differential Equations~(Neural~ODEs)~\citesupp{chen2018neuralode} reinterpret residual transitions as continuous-time vector fields integrated by adaptive numerical solvers; this differential perspective directly illuminates why discovered \papershort{} rules replace naive fixed-point steps with higher-order Runge--Kutta, Adams--Bashforth, or hyperspherical geodesic transitions. On the theoretical side, Levine et~al.~\cite{levine2020limits} establish when depth efficiency outstrips width in self-attention networks, framing why iterative refinement within a block can express compositions unreachable in a single shallow pass.

\paragraph{Expressivity, optimization dynamics, and generalization of looped transformers.}
Recent theoretical and mechanistic work studies what algorithms looped transformers naturally learn and implement in context. Giannou et~al.~\citesupp{giannou2023looped} construct explicit weight configurations showing that shallow Transformers executed inside an iterative loop act as general-purpose programmable computers capable of running multi-step linear algebra and control-flow routines. For in-context learning, Yang et~al.~\citesupp{yang2024looped} show empirically that looped Transformers outperform matched-parameter deep Transformers at learning iterative optimization algorithms across diverse function classes, while Gatmiry et~al.~\citesupp{gatmiry2024loopedgd} prove that weight-tied looped Transformers can represent multi-step preconditioned gradient descent with exponentially better depth efficiency than non-looped counterparts. Investigating out-of-distribution scaling, Fan et~al.~\citesupp{fan2025lengthgen} demonstrate that adaptive loop iteration substantially improves algorithmic length generalization when test instances require more computational steps than seen during training. From a systems and training-cost standpoint, Xiong et~al.~\cite{xiong2026truncate} analyze scaling laws under truncated backpropagation through time~(TBPTT), characterizing how training compute and memory trade off against recurrent unroll length during pretraining.

\paragraph{Pretrained looped backbones and training-free test-time looping.}
Building on these insights, a wave of pretrained models explicitly builds recurrent depth into large language, diffusion, and world-model architectures. In language modeling, Huginn~\cite{geiping2025recurrent} scales latent-space reasoning by iterating a weight-tied recurrent core between fixed prelude and coda stacks, Ouro~\cite{zhu2025ouro} optimizes adaptive recurrent depth allocation during large-scale pretraining, Mixture-of-Recursions~\cite{bae2025mixture} couples parameter sharing with token-level recursive depth routing, and Dory1.0-4B~\citesupp{fishman2026dory} trains an open-weight $4$B normalized-GPT natively with elastic recurrent depth. Addressing the conversion cost of existing pretrained models, Relaxed Recursive Transformers~\citesupp{bae2025relaxed} initialize weight-tied blocks from standard LLMs and recover specialization with lightweight layer-wise LoRA adapters, Inner Thinking Transformer~\citesupp{chen2025itt} elicits adaptive latent thinking via residual routing over shared layers, and Coconut~\citesupp{hao2025coconut} feeds continuous hidden states directly back as thought tokens instead of projecting every reasoning step to vocabulary logits. To stabilize multi-pass feedback, Rectified Looped Transformer~\cite{li2026rectified} interpolates intermediate states toward predicted recurrent endpoints. In visual and embodied domains, Looped-DiT~\cite{chng2026looped} trains diffusion Transformers with weight-tied core blocks, intermediate step supervision, and inner-loop attention regulation; LiFT~\cite{derakhshani2026lift} supervises a shared flow Transformer along targets parameterized by continuous computational depth; and LoopWM~\cite{lu2026loopedworld} trains interactive world models with variable test-time loop depth. Finally, training-free looping methods inject recurrence into \emph{frozen, unlooped} checkpoints: Training-Free Looped Transformers~\cite{chen2026trainingfreelooped} formulate hidden-state repetition as damped pseudo-time residual steps, Yan et~al.~\cite{yan2026trainingfree} introduce LoopGuidance and block-band repetition for flow-matching generators, and GramLoop~\cite{chen2026gramloop} gates spatial feature replay using Gram-matrix consistency.

\subsection{Dynamic Depth, Early Exiting, and Conditional Computation}
\label{sec:supp_rw_dynamic}

Rather than repeating layers to deepen computation, a complementary line of work skips layers on easy tokens or samples to reduce average cost. In language models, CALM~\citesupp{schuster2022calm} attaches per-token confidence classifiers to enable calibrated early exiting during autoregressive decoding while preserving consistency across KV states of skipped upper layers. LayerSkip~\citesupp{elhoushi2024layerskip} trains transformers with structured layer dropout and an early-exit loss so lower layers can draft tokens verified via self-speculative decoding against the remaining layers. Mixture-of-Depths~(MoD)~\citesupp{raposo2024mod} replaces fixed uniform computation with a fixed per-layer compute budget routed to the top-$k$ selected tokens, later unified with parameter-shared recursion in Mixture-of-Recursions~\cite{bae2025mixture}. Our evaluated programs can combine repeated computation with skipping or reuse while retaining frozen backbone weights.

\subsection{Test-Time Compute Scaling and Inference-Time Diffusion Acceleration}
\label{sec:supp_rw_tts}

\paragraph{Test-time compute in language reasoning.}
Scaling inference compute beyond greedy single-pass decoding has become central to LLM reasoning. Explicit token-space scaling began with Chain-of-Thought prompting~\citesupp{wei2022cot} and evolved into large-scale outcome-verifiable RL policies such as DeepSeek-R1~\citesupp{deepseek2025r1}, which allocate long explicit reasoning chains to difficult problems. Snell et~al.~\citesupp{snell2025testtime} systematically compare proposal, verifier, and sequential revision strategies, proving that compute-optimal test-time allocation can outperform scaling model parameters by several-fold. Whereas token-level test-time scaling pays $O(L_{\mathrm{cot}})$ autoregressive decoding steps and KV-cache growth per trace, recurrent-depth models~\cite{geiping2025recurrent,zhu2025ouro,li2026rectified} and \papershort{}'s loop programs operate in \emph{continuous latent depth}. Appendix~\ref{sec:supp_dory} evaluates recurrent-depth programs on Dory1.0-4B.

\paragraph{Diffusion test-time scaling, fast solvers, and feature caching.}
In visual generative models, Ma et~al.~\citesupp{ma2025scalingdiff} scale test-time compute by pairing best-of-$N$ and zero-order noise search with domain verifiers, complementing Self-Guided~\cite{hu2023selfguided} and token-sparse~\cite{krause2026guiding} guidance mechanisms. Orthogonal to outer search over initial noises, fast numerical integrators such as DPM-Solver~\citesupp{lu2022dpmsolver} and UniPC~\citesupp{zhao2023unipc} reduce outer NFEs through exponential integrators and unified predictor--corrector schemes. Training-free caching further amortizes repeated denoiser calls across timesteps: DeepCache~\citesupp{ma2024deepcache} reuses high-level U-Net features along skip branches across consecutive steps, TeaCache~\citesupp{liu2025teacache} dynamically schedules video-diffusion feature reuse from timestep-modulated embedding shifts, and TaylorSeer~\citesupp{liu2025taylorseer} replaces naive feature copying with Taylor-series forecasting of intermediate Transformer activations. Our search may edit reuse rules jointly with recurrent updates; the diagnostic evidence and resulting programs are documented in Appendices~\ref{sec:supp_search_design}--\ref{sec:supp_observations}.

\subsection{Autoregressive Video Diffusion and Long-Horizon Consistency}
\label{sec:supp_rw_video}

Generating minute-scale or cyclic camera-revisit videos requires bridging the mismatch between parallel bidirectional diffusion training and causal chunk-wise autoregressive rollout. Diffusion Forcing~\citesupp{chen2024diffusionforcing} introduces independent per-frame noise levels so trajectories can mix planning, stabilization, and streaming causal decoding, while History-Guided Video Diffusion~\citesupp{song2025history} extends arbitrary-length history conditioning to stabilize transitions and long-horizon memory. To achieve real-time streaming synthesis, CausVid~\citesupp{yin2025causvid} distills bidirectional video teachers into few-step causal autoregressive generators, Self-Forcing~\cite{huang2025selfforcing} rolls out self-generated frames during distribution-matching training to curb exposure bias, and LongLive~1.0/2.0~\cite{yang2026longlive,chen2026longlive2} scale interactive KV-cached chunk streaming with FP4 kernel optimizations. MosaiChunk and RememBench~\cite{zhang2026mosaichunk} establish standardized camera-departure and camera-revisit benchmarks alongside spatiotemporal KV memory compositing, while MemFlow~\citesupp{ji2025memflow} evaluates $60$\,s six-prompt narrative generation with adaptive memory. We evaluate inference-time loop programs on frozen LongLive and Self-Forcing checkpoints on both RememBench and MemFlow; their cache protocols are summarized in Prompts~4c--4d.

\subsection{Neural Architecture Search and LLM-Guided Program Discovery}
\label{sec:supp_rw_search}

Automated network and algorithm design traditionally framed structural search over differentiable continuous relaxations such as DARTS~\citesupp{liu2019darts} or discrete black-box evolutionary controllers that optimize static architecture topologies requiring full training from scratch. With the advent of coding-capable LLMs, evolutionary program search operates directly over readable, executable source code: FunSearch~\cite{romeraparedes2024funsearch} couples LLM mutators with island-based evolutionary evaluators to uncover new combinatorial bounds and online bin-packing heuristics, AlphaEvolve~\cite{novikov2025alphaevolve} scales full-codebase evolution to hardware kernels and scheduling algorithms, EoH~\cite{liu2024eoh} and ReEvo~\cite{ye2024reevo} co-evolve natural-language algorithmic concepts and reflective feedback, Eureka~\cite{ma2024eureka} synthesizes reinforcement-learning reward functions via vectorized fitness feedback, and Automated Design of Agentic Systems~(ADAS)~\citesupp{hu2025adas} searches over complete executable agent control flows alongside domain-specific pipelines like DS-Agent~\cite{guo2024dsagent} and PromptAgent~\cite{wang2024promptagent}. Moving from blind scalar score evaluation toward mechanistic inspection, OPAL~\cite{bai2026reactive} equips a coding agent to inspect neural training diagnostics and rewrite optimizers online, while OODA-Tool~\cite{guo2026oodatool} structures multi-turn action generation around explicit controller-verified state transitions. Our search edits inference programs between experiments with frozen weights. Selected programs subsequently execute without further calls to the search LLM.
