# Supplementary material for: Evolving Loop Programs: Discovering How Frozen Transformers Should Loop
Source: arXiv:2611.41108 source file (2026-12-03)
Supplement: Supplementary file 13 [file appendix_search_design.tex]

\FloatBarrier
\section{Search Design and Search-Target Calibration}
\label{sec:supp_search_design}

This section expands the search-design comparisons in RQ2. We compare search spaces, diagnostics, search LLMs, and objectives, add an initial search context ($\mathcal{C}_0$) ablation on $60$\,s multi-prompt video, and examine search-target calibration for image diffusion and autoregressive text reasoning. A search target is the quality--cost reference presented to the LLM during search. It is distinct from the fixed hypervolume reference point used to compute Pareto hypervolume. The image and text studies use different tasks and scoring protocols, so their target shifts and outcomes are interpreted separately.

\subsection{Complete Frozen Loop Programs}
\label{sec:supp_programs}
Table~\ref{tab:supp_searched_solutions} expands the two examples in
Table~\ref{tab:searched_solutions} to eight backbones, adding Dory1.0-4B~\citesupp{fishman2026dory} alongside unlooped image, video, and text backbones; Self-Forcing~1.3B uses the minimal loop-only interface summarized in Prompt~4c and Table~\ref{tab:supp_exp_settings}. Read each row
from the operating priority through loop structure, state-update dynamics,
and execution control. Across all eight backbones, discovered programs converge on a shared mechanistic principle: they concentrate recurrence inside middle semantic blocks during high-noise or multi-step reasoning stages, while pairing it with modality-specific state transitions and memory controls---cross-step correction or residual reuse in image diffusion, deferred final-pass KV commits in autoregressive video and text rollouts, and geodesic/spherical state extrapolation in pretrained looped models. All rules describe frozen programs replayed
without further search-LLM calls; the complete settings retain the
backbone-specific mechanisms omitted from the compact main-paper table.

\begin{table*}[!htbp]
\centering
\caption{\textbf{\rqhighlight{2}{\papershort{} discovers programs with distinct loop structures, state-update dynamics, and execution controls across backbones.}} Rules summarize the frozen operating points reported in Tables~\ref{tab:main_comparison}, \ref{tab:memflow_context}, \ref{tab:video_vbench}, \ref{tab:supp_dory_gen}, and~\ref{tab:supp_dory_stem4145}, plus the LongLive~1.0 setting in Table~\ref{tab:searched_solutions} from the additional window/depth study; $s$ denotes outer sampling steps.}
\label{tab:supp_searched_solutions}
\footnotesize
\setlength{\tabcolsep}{3pt}
\renewcommand{\arraystretch}{1.15}
\setlength{\aboverulesep}{0pt}
\setlength{\belowrulesep}{0pt}
\setlength{\extrarowheight}{1.6pt}
\begin{tabular*}{\textwidth}{@{\extracolsep{\fill}}>{\raggedright\arraybackslash}p{0.120\textwidth} >{\raggedright\arraybackslash}p{0.135\textwidth} >{\raggedright\arraybackslash}p{0.095\textwidth} | >{\raggedright\arraybackslash}p{0.183\textwidth} >{\raggedright\arraybackslash}p{0.205\textwidth} >{\raggedright\arraybackslash}p{0.180\textwidth}@{}}
\toprule
\textbf{Task} & \textbf{Backbone} & \textbf{Priority} & \textbf{Loop structure} & \shortstack[l]{\textbf{State-update dynamics}} & \textbf{Execution control} \\[1.6pt]
\midrule
Image generation & Scale-RAE~\cite{tong2026scaling} & Speed ($10s$) /\newline Quality ($14s$) & Layerwise dense loop on blocks $12$--$27$ of $32$ ($K{=}2$) & Damped Euler ($\Delta\mathbf h {=} 0.5(B_l(\mathbf h){-}\mathbf h)$) + output LoopGuidance ($w{=}3.0$) & Early half ($t/(T{-}1){\le}0.5$); skip $D_{\mathrm{ref}}$ if $K_t{=}0$; interval-$2$ $D_{\mathrm{ref}}$ refresh + $1$-step $\Delta_{\mathrm{cached}}$ \\[2.5pt]
Image generation & RAE~\cite{leng2026diffusionbench} & Speed ($6s$) /\newline Quality ($10s$) & Modality-split sparse loop on encoder blocks $19$--$22$ of $28$ ($K{=}4$; image queries at $k{=}1..3$) & Split Euler ($\lambda/K{=}0.25$) with cached $\Delta_{\mathrm{cond}}$ on text/time + LoopGuidance ($w{=}15$/$12$) & Early half ($t/(T{-}1){\le}0.5$); share unlooped prefix blocks $0$--$18$ across $D_{\mathrm{ref}}$ and $D_{\mathrm{loop}}$ \\[2.5pt]
Image generation\newline (pretrained loops) & Looped-DiT-B32~\cite{chng2026looped} & Speed ($14s$) /\newline Quality ($25s$) & Adaptive $K_t{\in}\{4,2\}$ ($48$ passes) or full $K_t{=}4$ ($100$ passes) on $5$-block core & Dual-stream latent extrapolation ($\alpha{=}0.20$/$0.22$); cached $\Delta_{2\to 4}$ (Speed); damped/tapered $x_0$ AB2 ($\beta{=}0.32$) & Curvature-warped SNR schedule ($s{=}1.38$/$1.30$); symmetric $4/2$ stride (age ${\le}2$); cached text preamble \\[2.5pt]
Text reasoning & Qwen3-4B~\cite{yang2025qwen3} & Micro /\newline Macro & Non-overlapping dual window ($54$ vs.\ $36$ layers): $[14]\,{+}\,[15..18]$ and $[25..28]$ ($K{=}3$) & Post-$L_{14}$ tapered RK3 ($H{=}1.12,\tau{=}0.20$, norm $\gamma{=}0.25$) in W1; anchored Ralston RK3 in W2 & Full-token FP32 state updates; read-only intermediate RK probes (\texttt{use\_cache=False}), single KV commit \\[2.5pt]
Text reasoning\newline (pretrained loops) & Dory1.0-4B~\citesupp{fishman2026dory} & STEM ($K{=}2$/$3$/$4$) /\newline Open ($K{=}2$) & Weight-tied elastic recurrent block; span recurrence ($K{=}2$ STEM) or matched $K{\in}\{2,3,4\}$ passes & STEM: spherical velocity extrapolation + calibrated scaling ($K{=}3$); annealed input injection, rate scaling \& continuation ($K{=}4$). Open: geodesic extrapolation after pass~$2$ & Matched-$K$ compute ($1.17\times$ speedup at $K{=}2$ STEM); converged last-loop or per-loop KV states on open-ended decoding \\[2.5pt]
Long video\newline generation & LongLive 2.0 5B~\cite{chen2026longlive2} & w/ Ours\newline (consistency) & Contiguous windowwise loop over causal Wan-DiT blocks $11$--$18$ of $30$ ($K{=}6$) & Windowwise Euler ($K{=}6$):\newline $\Delta\mathbf x^{(r)}{=}\tfrac{1}{6}(W(\mathbf x^{(r)}){-}\mathbf x^{(r)})$ & First $3$ of $4$ chunk-wise UniPC steps ($t{\in}\{999,937,833\}$); defer causal KV commit to final pass $r{=}5$ \\[2.5pt]
Long video\newline ($60$\,s multi-prompt) & LongLive 2.0 5B~\cite{chen2026longlive2} & Minimal:\newline Qual.\ / Speed & Cross-attention sublayer loop on $12$ blocks ($8$--$10,12,13,15,17,18,21$--$24$; $K{=}2$) & Temporally decoupled orthogonal updates ($\lambda{=}0.22$/$0.25$; motion gain $1.02$/$1.045$) & Steps $\{1,2\}$; opening-segment scale $0.15\times$; Speed keeps $4$ steps on $18$ anchor chunks, $3$ on $27$ steady chunks \\[2.5pt]
Long video\newline ($60$\,s multi-prompt) & LongLive 2.0 5B~\cite{chen2026longlive2} & Matched:\newline Qual.\ / Speed & Coupled dual windows $[13..15]$ and $[16..18]$ ($K{=}2$) & Windowwise Euler ($\lambda{=}0.5$, norm blend $0.5$) with step temporal/velocity weighting & Steps $\{0,1\}$; Speed drops step $t{=}937$ on $24$ steady interior chunks ($4$ per $10$\,s segment) \\[2.5pt]
Long video\newline generation & LongLive 1.0 1.3B~\cite{yang2026longlive} & Highest CLIP\newline in window/\newline depth study & Contiguous windowwise loop over causal blocks $12$--$18$ of $30$ ($K{=}4$) & Windowwise Euler:\newline $\Delta\mathbf x^{(r)}{=}\tfrac{1}{4}(W(\mathbf x^{(r)}){-}\mathbf x^{(r)})$ & Loop only at denoising steps $\{0,1\}$ of $4$; defer causal KV commit to final pass $r{=}3$ \\[2.5pt]
Short video\newline generation & Wan2.1-1.3B~\cite{wan2025wan} & Speed ($26s$) /\newline Quality ($50s$) & Speed: cond.\ cross-attention on $10$--$13$ ($K{=}3$); Quality: $3$ windows $[[10,11],[12,13],[18,19]]$ ($K{=}2$) & Speed: convex ODE weights $[0.2,0.3,0.5]$; Quality: spacetime curvature-lookahead RK2 ($[0.63,0.37]$) & Speed: $t/T{\in}[0.05,0.40)$, CFG decay $6.5{\to}4.0$ + interval-$5$ reuse; Quality: $t/T{\in}[0,0.46)$, shift $7.5$ \\[1.6pt]
\bottomrule
\end{tabular*}
\end{table*}

\paragraph{Middle-band and slightly post-center loop placement.}
Across Tables~\ref{tab:supp_searched_solutions} and~\ref{tab:longlive10_loop_variants}(b), discovered loops consistently avoid input/output boundary layers and cluster at or slightly past network center---aligning with middle-depth looping in frozen language models~\cite{chen2026trainingfreelooped} while exposing a finer post-center sweet spot. The cleanest controlled evidence comes from the fixed-width, fixed-$K$ LongLive~1.0 sweep (Table~\ref{tab:longlive10_loop_variants}(a)): shifting the same seven-block window just one block deeper past center ($11$--$17 \to 12$--$18$ of $30$) improves both semantic alignment (CLIP) and perceptual revisit fidelity (LPIPS), whereas an earlier band ($9$--$15$) maximizes local smoothness (TempSSIM), showing that optimal placement within the middle band is metric-dependent. Unlooped backbones across modalities echo this pattern---Self-Forcing ($14$--$19/30$), Scale-RAE ($12$--$27/32$), RAE ($19$--$22/28$), and Qwen3-4B (a central window plus blocks $25$--$28/36$)---though Qwen3-4B's gain reflects its combined dual-window RK3 edit relative to Fixed Loop~\cite{chen2026trainingfreelooped} rather than an isolated window shift.

\paragraph{Representative frozen loop programs.}
The listings below distill three frozen programs from Table~\ref{tab:supp_searched_solutions} (for Scale-RAE Speed, Looped-DiT-B32 Speed, and LongLive~2.0~5B) to illustrate how discovered rules jointly coordinate loop structure, state-update dynamics, and execution controls at deployment without calls to the search LLM.

\begin{lpsprompt}{Frozen Program 1: Scale-RAE 10-step Speed (\texttt{step10\_open\_r6\_euler2\_lg300\_reuse2\_s10})}
# Deployed inside Euler sampling over steps t_idx = 0..9 (total T = 10)
w, interval, reuse_scale = 3.0, 2, 1.0
delta_cache, refresh_step = None, -999

for t_idx in range(T):
    if t_idx / max(T - 1, 1) <= 0.5:  # Early active loop window; repeat blocks 12..27 with K=2
        def loop_forward(x_t, cond):
            h = prefix_blocks(0..11)(x_t, cond)
            for l in range(12, 28):
                for k in range(2):  # Damped Euler step size lambda/K = 0.5
                    h = h + 0.5 * (block[l](h) - h)
            return suffix_blocks(28..31)(h)

        if delta_cache is None or (t_idx - refresh_step) >= interval:
            d_ref = unlooped_forward(x_t, cond)
            d_loop = loop_forward(x_t, cond)
            delta_cache, refresh_step = (d_loop - d_ref).detach(), t_idx
            pred = d_ref + w * delta_cache
        else:  # Skip reference pass on odd steps; reuse cached correction
            d_loop = loop_forward(x_t, cond)
            pred = d_loop + (w - 1.0) * reuse_scale * delta_cache
    else:  # Skip loops & reference pass in late steps (K_t = 0)
        pred = unlooped_forward(x_t, cond)
    x_t = euler_step(x_t, pred, t_idx)
\end{lpsprompt}

\begin{lpsprompt}{Frozen Program 2: Looped-DiT-B32 14-step Speed (\texttt{step14\_open\_r1\_s1\_s14\_rescache\_cap8})}
# Curvature-warped SNR schedule (s=1.38) over 14 steps; 48 total conditional core passes
res_cache, cache_step = {}, {}
prev_pred = None
txt_pre, pos_emb = precompute_text_preamble(prompt)  # Cached across all timesteps

for idx, (t0, dt_ratio) in enumerate(warped_snr_schedule(steps=14, s=1.38)):
    n_cond = 4 if (idx in refresh_steps or t0 < low_t) else 2  # Adaptive K_t in {4, 2}
    img, txt = pre_blocks(x_t, txt_pre, pos_emb)
    hist_img, hist_txt = [img], [txt]
    for r in range(1, n_cond + 1):
        prev_img, prev_txt = img, txt
        img, txt = run_weight_tied_core(img, txt)  # 5 weight-tied blocks
        hist_img.append(img); hist_txt.append(txt)
    if n_cond == 4:
        if 0.12 <= t0 < 0.90:  # Dual-stream latent extrapolation on full refresh
            img = img + 0.20 * (img - prev_img)
            txt = txt + 0.20 * (txt - prev_txt)
        res_cache[2], cache_step[2] = (img - hist_img[2], txt - hist_txt[2]), idx
    elif 2 in res_cache and (idx - cache_step[2]) <= 2:  # Bounded residual reuse (age <= 2)
        d_img, d_txt = res_cache[2]
        img, txt = img + res_weight * d_img, txt + res_weight * d_txt
    pred = post_blocks(img, txt)
    if prev_pred is not None:  # Tapered x0 second-order AB2 update
        pred = pred + (0.32 * taper(t0) * dt_ratio) * (pred - prev_pred)
    prev_pred = pred
    x_t = step_update(x_t, pred, idx)
\end{lpsprompt}

\begin{lpsprompt}{Frozen Program 3: LongLive 2.0 5B Consistency (\texttt{r08\_ww\_layers11\_18\_steps012\_k6})}
# Autoregressive 12-chunk UniPC rollout; shift=5 noise schedule [999, 937, 833, 624]
for chunk in range(12):
    x_c = init_chunk_noise(chunk)
    for step_idx in range(4):
        x = prefix_blocks(0..10)(x_c, causal_kv_cache, write_kv=True)
        if step_idx in (0, 1, 2):  # Contiguous middle window blocks 11..18, K=6
            for r in range(6):
                commit_kv = (r == 5)  # Defer KV cache writes until final loop pass
                x_w = window_blocks(11..18)(x, causal_kv_cache, write_kv=commit_kv)
                x = x + (x_w - x) / 6.0  # Step-normalized windowwise Euler update
        else:  # Step 3 (t=624) executes unlooped
            x = window_blocks(11..18)(x, causal_kv_cache, write_kv=True)
        x_c = unipc_step(x_c, suffix_blocks(19..29)(x, write_kv=True), step_idx)
\end{lpsprompt}

\FloatBarrier
\subsection{Representative Summaries and Replay Records}
\label{sec:supp_selection_records}
The image-search coordinator requests quality-, speed-, and
balanced-priority representatives in the search LLM's final summary.
This is a recommendation based on the accumulated evidence, rather than
an implemented universal weighted-score maximizer or tie-breaking rule.
The named operating points in the result tables identify particular
frozen programs; Pareto membership alone does not determine these names.

For Scale-RAE, the saved two-anchor \texttt{Gemini-4-Argon}
final summary recommends the $15$-step candidate
\nolinkurl{step15_open_r6_step15_ce2_b12_30_t0_58_e30_a54_g075}
for high development GenEval at above-baseline speed; its full-benchmark
replay reproduces $57.30/79.64$ GenEval/DPG, matching the Speed row in
Table~\ref{tab:ablation_agent_target}.

For RAE, the replay manifest identifies
\nolinkurl{step6_r7_b19_22_condition_reuse_k4_lg15} (Speed) and
\nolinkurl{step10_r7_b19_22_condition_reuse_k4_lg12} (Quality),
both frozen from the Round~7 source snapshot (SHA-256:
\nolinkurl{f6a53bf1791cbcba8c78464f74984473831611c0b6613d7f1f45acdb5b902dbf}).
Full-benchmark replay reproduces their Table~\ref{tab:main_results}
GenEval/DPG pairs ($44.42/74.96$ and $44.94/74.47$).
Appendix~\ref{sec:supp_exp_settings} summarizes the selection notes and
reproduction settings across all backbones.

\subsection{Recorded Search LLM Episode on Scale-RAE}
\label{sec:supp_agent_episode}
Figure~\ref{fig:supp_agent_reasoning_full} records a complete Scale-RAE decision episode (\texttt{GPT-6-Astra}, rounds 4--6), linking diagnostic falsification, executable code edits, and controlled evaluation. Across $208$ image-step observations from $32$ images, looped and reference predictions at the same step have high cosine similarity ($0.994$--$0.995$), yet reusing their LoopGuidance correction from two steps back incurs $0.86$--$1.10$ relative error versus $0.56$--$0.73$ from one step back, falsifying lag-$\ge\!2$ caching and linear extrapolation despite high cosine alignment (a,b). In the resulting $10$-step edit (c), all ten image updates still run---five with fresh looped predictions followed by five unlooped steps---while extra reference calls during loop-active steps drop from five to three by reusing the prior correction at odd steps. In a separate matched $12$-step test with three reference calls (d), reusing rather than omitting corrections at skipped-reference steps raises development GenEval from $60.23$ to $64.14$ ($+3.91$\,pp), yielding the Speed and Quality programs in Table~\ref{tab:main_results}. This episode illustrates within-step computation changes rather than step reduction or an isolated diagnostics ablation.

\begin{figure*}[!htbp]
\centering
\input{figs/fig_agent_reasoning}
\caption{\textbf{\rqhighlight{2}{Recorded Search LLM reasoning links diagnostic falsification, executable code edits, and controlled evaluation.}} In the Scale-RAE search (\texttt{GPT-6-Astra}, Round~4 probe to Round~6), a collector written by the search LLM falsifies lag-$\ge\!2$ caching and linear extrapolation despite $0.995$ output alignment (a,b), motivating one-step correction reuse with fresh $D_{\mathrm{loop}}$ passes (c) that outperforms a matched-call omission control and yields the Speed and Quality programs in Table~\ref{tab:main_results} (d).}
\label{fig:supp_agent_reasoning_full}
\label{fig:agent_reasoning_example}
\end{figure*}
\FloatBarrier

\subsection{Search Space, Diagnostics, Search LLMs, and Objectives}
\label{sec:supp_search_ablations}

\Cref{tab:supp_agent_pareto_balanced} expands \cref{tab:ablation_search_mode,tab:ablation_agent_target,tab:rae_single_metric_search} with Balanced programs, step counts, development latency-based Pareto hypervolume gain ($\Delta\mathrm{HV}$), FLOPs speedups relative to standard inference (Base) and Loop~+~LG (w/ LG), and explicit $1{,}298$-prompt held-out scores ($441$ GenEval, $857$ DPG-Bench). Panel~(a) unifies the search-space and diagnostic-access comparisons: Configuration Search varies a predefined configuration space using fixed probes, whereas \papershort{} also edits executable rules with or without programmable diagnostics. Panels~(b) and~(c) expand the search-LLM and objective comparisons following the RQ2 protocol.

Table~\ref{tab:supp_agent_pareto_balanced} separates development and held-out performance for the image-search ablations. The complementary initial-search-context ablation on $60$\,s multi-prompt video appears in Section~\ref{sec:supp_context_ablation}. These comparisons identify useful choices within the evaluated settings, without establishing a universal relation between panel size and allowable program edits.

Latency $\Delta\mathrm{HV}$ in~(a) is the increase over the shared initial anchors, using GenEval, DPG, and measured latency speedup; timing covers denoising with cached conditioning at batch $8$, while replay TFLOPs use separate cost accounting. The scores-only search has the largest development latency HV gain ($1.192$ versus $0.946$ with diagnostics), despite lower full-benchmark GenEval. The held-out ($441$ GenEval, $857$ DPG) and full-benchmark ($553$ GenEval, $1{,}065$ DPG) scores are shown separately. Parenthesized factors beside TFLOPs in~(b) are speedups over the $25$-step Baseline. Rankings are within each panel.

\begin{table*}[!htbp]
\centering
\caption{\textbf{\rqhighlight{2}{Search space, diagnostic access, search LLMs, and objectives govern both held-out generalization and full-benchmark trade-offs on Scale-RAE.}} Panels~(a)--(c) expand Table~\ref{tab:agent_pareto} with Balanced programs, development latency-based HV gain, FLOPs speedups, and $1{,}298$-prompt held-out scores ($441$ GenEval, $857$ DPG-Bench). Gray shading: our full method; \textbf{bold}/\underline{underlined}: best/second-best within each panel.}
\label{tab:supp_agent_pareto_balanced}
\begin{subtable}[t]{\textwidth}
\centering
\caption{\textbf{Search Space and Diagnostic Access (Scale-RAE).}}
\label{tab:supp_ablation_diagnostics}
\setlength{\tabcolsep}{3.0pt}
\renewcommand{\arraystretch}{1.10}
\scriptsize
\begin{tabular*}{\textwidth}{@{\extracolsep{\fill}}l c l c | c | c c | c c | r c@{}}
\toprule
\multirow{2}{*}{\textbf{Search variant}} & \multirow{2}{*}{\textbf{Diag.}} & \multirow{2}{*}{\textbf{Priority}} & \multirow{2}{*}{\textbf{\#step}} & \multirow{2}{*}{\shortstack{\textbf{Latency}\\\textbf{$\Delta$HV $\uparrow$}}} & \multicolumn{2}{c|}{\textbf{Held-out (\%) $\uparrow$}} & \multicolumn{2}{c|}{\textbf{Full (\%) $\uparrow$}} & \multirow{2}{*}{\textbf{TFLOPs $\downarrow$}} & \textbf{Speedup $\uparrow$} \\
\cmidrule(lr){6-7}\cmidrule(lr){8-9}
 & & & & & \textbf{GenEval} & \textbf{DPG} & \textbf{GenEval} & \textbf{DPG} & & \textbf{(Base / w/ LG)} \\
\midrule
\multirow{2}{*}{Configuration Search} & \multirow{2}{*}{\cmark}
 & Speed & 10 & \multirow{2}{*}{0.764} & 53.83 & 79.21 & 55.05 & 79.45 & \underline{17.34} & \underline{$1.82\times$} / \underline{$5.05\times$} \\
 & & Quality & 10 & & 58.35 & 80.10 & 59.88 & \underline{80.26} & 29.97 & $1.05\times$ / $2.92\times$ \\
\midrule
\multirow{2}{*}{\papershort{} w/o Diagnostics} & \multirow{2}{*}{\xmark}
 & Speed & 8 & \multirow{2}{*}{\textbf{1.192}} & 50.71 & 79.75 & 52.41 & 80.05 & \textbf{11.99} & $\boldsymbol{2.63\times}$ / $\boldsymbol{7.31\times}$ \\
 & & Quality & 14 & & 56.37 & 79.62 & 57.63 & 79.68 & 22.08 & $1.43\times$ / $3.97\times$ \\
\midrule
\rowcolor{gray!12}
 & & Speed & 10 & & \textbf{59.24} & 80.07 & \underline{60.54} & 80.19 & 19.56 & $1.61\times$ / $4.48\times$ \\
\rowcolor{gray!12}
 & & Balanced & 12 & & 56.89 & \underline{80.14} & 58.28 & \textbf{80.41} & 22.71 & $1.39\times$ / $3.86\times$ \\
\rowcolor{gray!12}
\multirow{-3}{*}{\papershort{} (Ours)} & \multirow{-3}{*}{\cmark} & Quality & 14 & \underline{0.946} & \underline{58.76} & \textbf{80.18} & \textbf{60.98} & 80.19 & 27.13 & $1.16\times$ / $3.23\times$ \\
\bottomrule
\end{tabular*}
\end{subtable}
\par\medskip
\begin{subtable}[t]{\textwidth}
\centering
\caption{\textbf{Search LLM: \texttt{GPT-6-Astra} vs.~\texttt{Gemini-4-Argon}.}}
\setlength{\tabcolsep}{4.5pt}
\renewcommand{\arraystretch}{1.10}
\scriptsize
\begin{tabular*}{\textwidth}{@{\extracolsep{\fill}}l l r | c c | c c | r@{}}
\toprule
\multirow{2}{*}{\textbf{Search LLM}} & \multirow{2}{*}{\textbf{Priority}} & \multirow{2}{*}{\textbf{\#step}} & \multicolumn{2}{c|}{\textbf{Held-out (\%) $\uparrow$}} & \multicolumn{2}{c|}{\textbf{Full (\%) $\uparrow$}} & \multirow{2}{*}{\textbf{TFLOPs $\downarrow$ (vs.\ Base)}} \\
\cmidrule(lr){4-5}\cmidrule(lr){6-7}
 & & & \textbf{GenEval} & \textbf{DPG} & \textbf{GenEval} & \textbf{DPG} & \\
\midrule
\multirow{3}{*}{\texttt{GPT-6-Astra}}
 & Speed & 10 & \textbf{59.24} & 80.07 & \underline{60.54} & \underline{80.19} & \textbf{19.56} ($\boldsymbol{1.61\times}$) \\
 & Balanced & 12 & 56.89 & \underline{80.14} & 58.28 & \textbf{80.41} & \underline{22.71} (\underline{$1.39\times$}) \\
 & Quality & 14 & \underline{58.76} & \textbf{80.18} & \textbf{60.98} & \underline{80.19} & 27.13 ($1.16\times$) \\
\midrule
\multirow{2}{*}{\texttt{Gemini-4-Argon}}
 & Speed & 15 & 55.53 & 79.41 & 57.30 & 79.64 & 25.53 ($1.24\times$) \\
 & Quality & 25 & 57.27 & 79.86 & 58.48 & 80.18 & 41.85 ($0.75\times$) \\
\bottomrule
\end{tabular*}
\end{subtable}
\par\medskip
\begin{subtable}[t]{\textwidth}
\centering
\caption{\textbf{Search Objectives: Joint vs.~Single-Metric.} GenEval-only was selected among three held-out replays; its held-out score is selection evidence, not independent confirmation.}
\setlength{\tabcolsep}{4.5pt}
\renewcommand{\arraystretch}{1.10}
\scriptsize
\begin{tabular*}{\textwidth}{@{\extracolsep{\fill}}l r | c c | c c | r c@{}}
\toprule
\multirow{2}{*}{\textbf{Setting}} & \multirow{2}{*}{\textbf{\#step}} & \multicolumn{2}{c|}{\textbf{Held-out (\%) $\uparrow$}} & \multicolumn{2}{c|}{\textbf{Full (\%) $\uparrow$}} & \multirow{2}{*}{\textbf{TFLOPs $\downarrow$}} & \textbf{Speedup $\uparrow$} \\
\cmidrule(lr){3-4}\cmidrule(lr){5-6}
 & & \textbf{GenEval} & \textbf{DPG} & \textbf{GenEval} & \textbf{DPG} & & \textbf{(Base / w/ LG)} \\
\midrule
Baseline~\cite{tong2026scaling} & 25 & 51.14 & 77.12 & 51.64 & 77.21 & 31.58 & $1.00\times$ / $2.77\times$ \\
Loop w/o LG~\cite{yan2026trainingfree} & 25 & 56.35 & 80.08 & 57.04 & 80.00 & 56.04 & $0.56\times$ / $1.56\times$ \\
Loop + LG~\cite{yan2026trainingfree} & 25 & 57.90 & 79.63 & 58.56 & 79.71 & 87.62 & $0.36\times$ / $1.00\times$ \\
\midrule
Joint (Speed) & 10 & \underline{59.24} & 80.07 & 60.54 & 80.19 & \textbf{19.56} & $\boldsymbol{1.61\times}$ / $\boldsymbol{4.48\times}$ \\
Joint (Balanced) & 12 & 56.89 & 80.14 & 58.28 & \underline{80.41} & \underline{22.71} & \underline{$1.39\times$} / \underline{$3.86\times$} \\
Joint (Quality) & 14 & 58.76 & \underline{80.18} & \underline{60.98} & 80.19 & 27.13 & $1.16\times$ / $3.23\times$ \\
\midrule
GenEval only & 20 & \textbf{61.77} & 80.04 & \textbf{63.15} & 80.15 & --- & --- \\
DPG only & 20 & 54.79 & \textbf{80.43} & 56.09 & \textbf{80.61} & --- & --- \\
\bottomrule
\end{tabular*}
\end{subtable}
\end{table*}

\paragraph{Single-objective search settings.}
The GenEval-only and DPG-only searches use \texttt{GPT-6-Astra}, the same two measured anchors as joint search, and $80$ candidates each, with development panels of $112$ GenEval and $208$ DPG-Bench prompts, respectively. The GenEval-only row reports the $20$-step blocks $12$--$27$ program selected among three held-out replays; the DPG-only row uses the development-set winner. Both are evaluated on full GenEval ($553$ prompts) and DPG-Bench ($1{,}065$ prompts) at seed $42$; joint rows reuse the programs in Table~\ref{tab:main_results}.

\FloatBarrier
\subsection{Initial Search Context Ablation on \texorpdfstring{$60$\,s}{60 s} Multi-Prompt Video}
\label{sec:supp_context_ablation}

Does supplying a search LLM with algorithmic hints and starter operators accelerate discovery, or bias it away from architecture-native mechanisms? To isolate how the initial search context $\mathcal{C}_0$ ($\mathcal{C}_r$ at $r{=}0$ in Equation~\eqref{eq:program_evolution})---specifically natural-language \emph{prompt guidance} and a \emph{starter operator library}---shapes discovered programs on an already distilled $4$-step backbone, we conduct a $2{\times}2$ ablation on $100$ $60$\,s six-prompt MemFlow narratives~\citesupp{ji2025memflow} with LongLive~2.0~5B~\cite{chen2026longlive2} (Tables~\ref{tab:memflow_context}--\ref{tab:supp_memflow_splits}). All four regimes share the same backbone, $20$-search / $80$-held-out split, $32$-candidate budget under \texttt{Gemini-4-Argon}, programmable diagnostics, and evaluation protocol:
(i)~\emph{Minimal context} gives neutral task instructions with an empty program template;
(ii)~\emph{Matched prior} pairs concise algorithmic guidance (loop-compensated step reduction, selective token looping, adaptive scheduling, and cached residual reuse) with a starter operator library adapted from our image experiments (Euler, Heun, and Midpoint integrators, token-selection masks, and block/window loop primitives; Prompt~4d in Appendix~\ref{sec:supp_prompts});
(iii)~\emph{Guidance only} supplies the algorithmic guidance without starter operators; and
(iv)~\emph{Library only} supplies the starter library without algorithmic guidance.
Across the rest of the paper, \emph{both} coupled context poles are deployed according to domain characteristics: video and world-model searches almost all use \textbf{Minimal context}, whereas image diffusion and text-reasoning backbones mostly use \textbf{Matched priors} (Table~\ref{tab:supp_exp_settings}).

\begin{table*}[!htbp]
\centering
\newcommand{\dpos}[1]{\,{\tiny\textcolor{green!50!black}{(#1)}}}
\newcommand{\dneg}[1]{\,{\tiny\textcolor{red!75!black}{(#1)}}}
\newcommand{\clow}[1]{\textcolor{black!50}{#1}}
\caption{\textbf{\rqhighlight{2}{Initial search context steers $60$\,s multi-prompt video trade-offs across $100$ MemFlow narratives (LongLive~2.0~5B).}} Columns align with MemFlow's protocol~\citesupp{ji2025memflow} plus analytical denoiser TFLOPs and FLOPs speedup over the native $4$-step baseline ($30{,}086$\,TFLOPs over $45$ chunks; gray text). Gray shading highlights the two coupled regimes (Minimal and Matched prior). Parentheses report signed deltas vs.\ the native baseline (\textcolor{green!50!black}{gains} / \textcolor{red!75!black}{regressions}); CLIP cells below baseline are muted. Minimal context and Matched prior exhibit complementary strengths, whereas uncoupled partial priors collapse quality at speed or induce template inertia.}
\label{tab:memflow_context}
\renewcommand{\arraystretch}{1.04}
\scriptsize
\setlength{\tabcolsep}{1.6pt}
\begin{tabular*}{\textwidth}{@{\extracolsep{\fill}}c c l | r c | c c c | c c c c c c@{}}
\toprule
\multicolumn{2}{@{}c}{\textbf{Context} $\mathcal{C}_0$} & \multirow{2}{*}{\textbf{Regime / Priority}} & \multirow{2}{*}{\textbf{TFLOPs $\downarrow$}} & \multirow{2}{*}{\textbf{Speedup $\uparrow$}} & \multicolumn{3}{c|}{\textbf{VBench-Long ($\uparrow$)}} & \multicolumn{6}{c@{}}{\textbf{CLIP Score ($\uparrow$)}} \\
\cmidrule(r){1-2} \cmidrule(lr){6-8} \cmidrule(l){9-14}
\textbf{Guid.} & \textbf{Lib.} & & & & \textbf{Quality} & \textbf{Cons.} & \textbf{Aesth.} & \textbf{0--10s} & \textbf{10--20s} & \textbf{20--30s} & \textbf{30--40s} & \textbf{40--50s} & \textbf{50--60s} \\
\midrule
\textcolor{black!55}{---} & \textcolor{black!55}{---} & \textcolor{black!55}{Native Baseline (4-step)} & \textcolor{black!55}{30{,}086} & \textcolor{black!55}{$1.00\times$} & \textcolor{black!55}{83.51} & \textcolor{black!55}{97.17} & \textcolor{black!55}{57.73} & \textcolor{black!55}{27.77} & \textcolor{black!55}{24.77} & \textcolor{black!55}{24.47} & \textcolor{black!55}{24.66} & \textcolor{black!55}{24.04} & \textcolor{black!55}{23.84} \\
\midrule
\rowcolor{gray!12}[0pt][0pt]
\xmark & \xmark & Minimal --- Quality & 30{,}442 & $0.99\times$ & 83.84\dpos{+0.33} & 97.15\dneg{-0.02} & 58.28\dpos{+0.55} & 27.77 & \clow{24.66} & 24.82 & 25.04 & 24.73 & 24.30 \\
\rowcolor{gray!12}[0pt][0pt]
\xmark & \xmark & Minimal --- Speed & 26{,}766 & $1.12\times$ & 83.60\dpos{+0.09} & 97.22\dpos{+0.05} & 58.32\dpos{+0.59} & \clow{27.76} & \clow{24.72} & 24.67 & 24.72 & 24.56 & 24.36 \\
\midrule
\rowcolor{gray!12}[0pt][0pt]
\cmark & \cmark & Matched --- Quality & 32{,}493 & $0.93\times$ & 83.75\dpos{+0.24} & 97.25\dpos{+0.08} & 58.29\dpos{+0.56} & 27.93 & 25.28 & 25.25 & 25.09 & 24.60 & 24.28 \\
\rowcolor{gray!12}[0pt][0pt]
\cmark & \cmark & Matched --- Speed & 29{,}225 & $1.03\times$ & 83.20\dneg{-0.31} & 97.28\dpos{+0.11} & 57.30\dneg{-0.43} & 27.92 & 25.10 & 24.90 & 25.30 & 24.76 & 24.25 \\
\midrule
\cmark & \xmark & Guidance only --- Quality & 29{,}447 & $1.02\times$ & 83.63\dpos{+0.12} & 97.14\dneg{-0.03} & 58.36\dpos{+0.63} & \clow{27.76} & 24.82 & 24.94 & 25.40 & 24.85 & 24.56 \\
\cmark & \xmark & Guidance only --- Speed & 24{,}321 & $1.24\times$ & 81.20\dneg{-2.31} & 96.49\dneg{-0.67} & 55.45\dneg{-2.28} & 28.27 & 25.59 & 25.66 & 25.42 & 24.89 & 24.53 \\
\midrule
\xmark & \cmark & Library only --- Quality & 31{,}094 & $0.97\times$ & 83.67\dpos{+0.16} & 97.14\dneg{-0.03} & 57.99\dpos{+0.26} & 27.77 & 24.78 & 24.60 & 24.81 & 24.30 & 23.95 \\
\xmark & \cmark & Library only --- Speed & 27{,}605 & $1.09\times$ & 83.27\dneg{-0.24} & 96.96\dneg{-0.21} & 57.32\dneg{-0.41} & 27.77 & 24.89 & 25.00 & 25.35 & 25.04 & 24.17 \\
\bottomrule
\end{tabular*}
\end{table*}

\paragraph{1. Minimal context uncovers architecture-native efficiency obscured by cross-domain templates.}
Without preconceived operators, diagnostic-led search asks \emph{where} long-horizon drift originates rather than how to adapt an image-diffusion recipe. On causal video diffusion, Round~$0$ probes pinpoint two structural properties: semantic drift concentrates at cross-attention layers across prompt transitions, while steady interior chunks converge early. Because cross-attention costs only $7.3\%$ of a full CausalWan block ($13.8\times$ cheaper than repeating causal self-attention and FFN), looping only cross-attention with temporally decoupled orthogonal updates reinforces text grounding at negligible overhead ($+1.2\%$ FLOPs for Quality), preserving enough compute margin for segment-aware step reduction on steady interior chunks. Minimal context is therefore the only regime whose Speed program accelerates inference ($1.12\times$ FLOPs speedup) without sacrificing visual quality ($+0.09$) or temporal consistency ($+0.05$; Table~\ref{tab:memflow_context}).

\paragraph{2. Matched priors trade structural novelty for reliable exploitation of known dynamics.}
Pairing algorithmic guidance with compatible ODE and window primitives steers search away from sublayer invention and toward coupled full-block temporal-velocity windows. This inductive bias pays off on horizon-wide prompt adherence and stability---Matched Quality is the only quality-preserving regime that improves every $10$\,s CLIP interval ($+0.48$ mean) alongside top consistency ($97.25$)---yet full-block repetition locks in higher compute cost ($+8.0\%$ FLOPs) and narrows the safety margin for step reduction (Matched Speed drops Quality by $-0.31$). Minimal context and Matched prior thus form \emph{complementary operating modes}: minimal priors excel when architecture-specific bottlenecks differ from prior domains, whereas matched priors excel when transferred dynamical primitives align with the target objective.

\paragraph{3. Guidance and starter operators must be coupled; partial priors fail asymmetrically.}
Decoupling the two context axes degrades the quality--compute frontier in opposite ways. \emph{Guidance only} creates an execution gap: the search knows which acceleration levers to attempt (step truncation, block skipping) but lacks calibrated stabilizing operators, so pushing for speed causes severe visual collapse ($-2.31$ Quality) even while inflating CLIP alignment and aggregate 5D hypervolume ($+30.9\%$)---a cautionary example of how uncalibrated multi-objective hypervolume can reward degenerate corner solutions. Conversely, \emph{Library only} induces \emph{template inertia}: anchored to pre-built primitives with fewer exploratory diagnostics, search makes conservative quality edits and resorts to brittle final-step block reuse under speed pressure ($-0.24$ Quality, $-0.21$ Consistency).

\paragraph{4. Held-out transfer and the necessity of joint schedule--loop co-design.}
Table~\ref{tab:supp_memflow_splits} confirms that the qualitative separation across regimes transfers cleanly from the $20$-video development panel to the $80$ unseen held-out narratives, with both coupled regimes sustaining positive held-out hypervolume over the native baseline ($+11.0\%$ Minimal, $+9.0\%$ Matched). Comparing against the restricted fixed-schedule comparators further isolates why joint search over schedules and update rules is essential: fixing the $4$-step schedule forces search into heavier full-block loops that raise compute by $11$--$16\%$ and consistently erode temporal consistency (down to $-0.22$) to gain visual quality, whereas open program search coordinates sublayer recurrence with segment-aware step allocation.

\begin{table*}[!htbp]
\centering
\caption{\textbf{\rqhighlight{2}{Held-out ($80$) and full ($100$) breakdown for the $60$\,s MemFlow initial search context study (LongLive~2.0~5B).}} Expands Table~\ref{tab:memflow_context} with $80$-video unseen confirmation alongside full-$100$-video VBench-Long scores, mean CLIP ViT-L/14, and denoiser TFLOPs. Gray shading highlights the two coupled regimes (Minimal and Matched prior); \textcolor{red!75!black}{red} marks VBench-Long regressions below the native baseline. Fixed-schedule comparators search only the loop update rule under a fixed $4$-step schedule and a 3D quality-only objective.}
\label{tab:supp_memflow_splits}
\footnotesize
\setlength{\tabcolsep}{3.5pt}
\renewcommand{\arraystretch}{1.08}
\begin{tabular*}{\textwidth}{@{\extracolsep{\fill}}l | c c c c | c c c c r@{}}
\toprule
\multirow{2}{*}{\textbf{Regime / Priority}} & \multicolumn{4}{c|}{\textbf{Held-out ($80$ Videos) ($\uparrow$)}} & \multicolumn{5}{c}{\textbf{Full ($100$ Videos) ($\uparrow$ except TFLOPs)}} \\
\cmidrule(lr){2-5}\cmidrule(lr){6-10}
 & \textbf{Qual.} & \textbf{Cons.} & \textbf{Aesth.} & \textbf{CLIP L/14} & \textbf{Qual.} & \textbf{Cons.} & \textbf{Aesth.} & \textbf{CLIP L/14} & \textbf{TFLOPs (Spd.)} \\
\midrule
Native Baseline (4-step) & 83.49 & 97.17 & 57.72 & 24.91 & 83.51 & 97.17 & 57.73 & 24.93 & 30{,}086 ($1.00\times$) \\
\midrule
\rowcolor{gray!12}
Minimal --- Quality & 83.89 & \textcolor{red!75!black}{97.14} & 58.39 & 25.14 & 83.84 & \textcolor{red!75!black}{97.15} & 58.28 & 25.22 & 30{,}442 ($0.99\times$) \\
\rowcolor{gray!12}
Minimal --- Speed & 83.71 & 97.22 & 58.53 & 25.05 & 83.60 & 97.22 & 58.32 & 25.13 & 26{,}766 ($1.12\times$) \\
\midrule
\rowcolor{gray!12}
Matched --- Quality & 83.70 & 97.26 & 58.56 & 25.54 & 83.75 & 97.25 & 58.29 & 25.41 & 32{,}493 ($0.93\times$) \\
\rowcolor{gray!12}
Matched --- Speed & \textcolor{red!75!black}{83.20} & 97.26 & \textcolor{red!75!black}{57.50} & 25.32 & \textcolor{red!75!black}{83.20} & 97.28 & \textcolor{red!75!black}{57.30} & 25.37 & 29{,}225 ($1.03\times$) \\
\midrule
Guidance only --- Quality & 83.68 & \textcolor{red!75!black}{97.14} & 58.50 & 25.39 & 83.63 & \textcolor{red!75!black}{97.14} & 58.36 & 25.39 & 29{,}447 ($1.02\times$) \\
Guidance only --- Speed & \textcolor{red!75!black}{81.26} & \textcolor{red!75!black}{96.51} & \textcolor{red!75!black}{55.68} & 25.71 & \textcolor{red!75!black}{81.20} & \textcolor{red!75!black}{96.49} & \textcolor{red!75!black}{55.45} & 25.73 & 24{,}321 ($1.24\times$) \\
\midrule
Library only --- Quality & 83.68 & 97.17 & 58.03 & 24.98 & 83.67 & \textcolor{red!75!black}{97.14} & 57.99 & 25.03 & 31{,}094 ($0.97\times$) \\
Library only --- Speed & \textcolor{red!75!black}{83.35} & \textcolor{red!75!black}{96.96} & \textcolor{red!75!black}{57.19} & 25.34 & \textcolor{red!75!black}{83.27} & \textcolor{red!75!black}{96.96} & \textcolor{red!75!black}{57.32} & 25.37 & 27{,}605 ($1.09\times$) \\
\midrule
Fixed-sched.\ (Win.\ 11--18) & 83.88 & \textcolor{red!75!black}{97.10} & 58.50 & 24.84 & 83.90 & \textcolor{red!75!black}{97.13} & 58.43 & 24.90 & 33{,}295 ($0.90\times$) \\
Fixed-sched.\ (Blk.\ 12--22) & 83.92 & \textcolor{red!75!black}{96.96} & 58.12 & 25.19 & 83.87 & \textcolor{red!75!black}{96.95} & 57.91 & 25.22 & 34{,}899 ($0.86\times$) \\
\bottomrule
\end{tabular*}
\end{table*}

\subsection{Target Strength in Image Generation}
\label{sec:supp_rae_synthetic_targets}

\Cref{tab:supp_rae_synthetic_target_ablation} expands \cref{tab:rae_synthetic_target_ablation} with the True Speed and $15$-step Ultra Balanced programs and separate development, held-out, and full results. Compare target settings within each split: Development is the search panel, and Full includes both development and held-out prompts. The original target coordinates allow the compact target strength percentages to be interpreted; the split columns test whether the selected trade-offs persist beyond search.

\paragraph{Target strength.}
For compact reporting in \cref{tab:rae_synthetic_target_ablation}, target strength is the mean relative increase in the search target's three coordinates: GenEval $G$, DPG $D$, and latency speedup $s$ in the search prompt. Here $s=\tau_{\mathrm{base}}/\tau$, where $\tau$ is warm inference time per image; it is not the FLOPs ratio reported in the replay columns. With target $\mathbf a=(G,D,s)$ and the measured True target $\mathbf a^{\mathrm{True}}$, we report
\begin{equation}
\text{Target strength}(\mathbf a)=\frac{1}{3}\sum_{j=1}^{3}\left(\frac{a_j}{a_j^{\mathrm{True}}}-1\right)\times100\%.
\end{equation}
The original target coordinates in \cref{tab:supp_rae_synthetic_target_ablation} give $0.00\%$ (True), $17.86\%$ (Strong), and $29.28\%$ (Ultra). These percentages use the rounded table values and summarize shifts that differ across objectives. They change the search target shown to the search LLM, not the fixed hypervolume reference point.

Each \texttt{Gemini-4-Argon} search evaluates $80$ candidates on $320$ development prompts, followed by replay on $1{,}298$ held-out prompts and all $1{,}618$ prompts. The target columns retain the original GenEval/DPG/latency-speedup coordinates. Replay TFLOPs and FLOPs speedups are computed separately from the latency signal shown to the search LLM. The Scale-RAE frontier and hypervolume summaries use the recorded development latencies. The Strong-target program uses uncached $20$-step guidance ($44.17$\,TFLOPs). Ultra-target programs use strided LoopGuidance with cross-step velocity-delta reuse ($16.09$--$31.23$\,TFLOPs).

\begin{table*}[!htbp]
\centering
\caption{\textbf{\rqhighlight{2}{Stronger search targets lift held-out GenEval and expand lower-compute trade-offs on Scale-RAE.}} Target $s$ denotes latency speedup; replay Speedup denotes FLOPs speedup. Development, held-out, and full-benchmark scores are shown separately. Target strength percentages in Table~\ref{tab:rae_synthetic_target_ablation} summarize the coordinate shifts.}
\label{tab:supp_rae_synthetic_target_ablation}
\footnotesize
\setlength{\tabcolsep}{2.8pt}
\begin{tabular}{@{}l c l r | c c | c c | c c | r c@{}}
\toprule
\multirow{2}{*}{\textbf{Method}} & \textbf{Search Target} & \multirow{2}{*}{\textbf{Priority}} & \multirow{2}{*}{\textbf{\#step}} & \multicolumn{2}{c|}{\textbf{Development (\%) $\uparrow$}} & \multicolumn{2}{c|}{\textbf{Held-out (\%) $\uparrow$}} & \multicolumn{2}{c|}{\textbf{Full (\%) $\uparrow$}} & \multirow{2}{*}{\textbf{TFLOPs $\downarrow$}} & \textbf{Speedup $\uparrow$} \\
\cmidrule(lr){5-6}\cmidrule(lr){7-8}\cmidrule(lr){9-10}
 & \textbf{(G / D / $\boldsymbol{s}$)} & & & \textbf{GenEval} & \textbf{DPG} & \textbf{GenEval} & \textbf{DPG} & \textbf{GenEval} & \textbf{DPG} &  & \textbf{(Base / w/ LG)} \\
\midrule
Baseline~\cite{tong2026scaling} & --- & --- & 25 & 53.80 & 77.55 & 51.14 & 77.12 & 51.64 & 77.21 & 31.58 & $1.00\times$ / $2.77\times$ \\
Loop w/o LG~\cite{yan2026trainingfree} & --- & --- & 25 & 59.88 & 79.70 & 56.35 & 80.08 & 57.04 & 80.00 & 56.04 & $0.56\times$ / $1.56\times$ \\
Loop + LG~\cite{yan2026trainingfree} & --- & --- & 25 & 60.42 & 80.06 & 57.90 & 79.63 & 58.56 & 79.71 & 87.62 & $0.36\times$ / $1.00\times$ \\
\midrule
\multirow{2}{*}{Ours (True)} & \multirow{2}{*}{$59.88$ / $79.70$ / $0.56\times$} & Speed & 15 & 64.50 & 80.60 & 55.53 & 79.41 & 57.30 & 79.64 & \underline{25.53} & \underline{$1.24\times$} / \underline{$3.43\times$} \\
 & & Quality & 25 & 63.38 & \underline{81.52} & 57.27 & 79.86 & 58.48 & 80.18 & 41.85 & $0.75\times$ / $2.09\times$ \\
Ours (Strong) & $65.17$ / $81.21$ / $0.80\times$ & Quality & 20 & 66.45 & \textbf{81.64} & \textbf{59.53} & 80.21 & 61.03 & \underline{80.49} & 44.17 & $0.72\times$ / $1.98\times$ \\
\midrule
\rowcolor{gray!12}
 & & \textbf{Speed} & 9 & 60.60 & 81.07 & 57.70 & \underline{80.24} & 58.32 & 80.40 & \textbf{16.09} & $\boldsymbol{1.96\times}$ / $\boldsymbol{5.45\times}$ \\
\rowcolor{gray!12}
 & & \textbf{Balanced} & 15 & \underline{68.74} & 80.95 & \underline{59.45} & \textbf{80.45} & \underline{61.47} & \textbf{80.55} & 27.73 & $1.14\times$ / $3.16\times$ \\
\rowcolor{gray!12}
\multirow{-3}{*}{Ours (Ultra)} & \multirow{-3}{*}{$71.31$ / $83.26$ / $0.92\times$} & \textbf{Quality} & 16 & \textbf{70.49} & 80.84 & 59.29 & 80.08 & \textbf{61.63} & 80.22 & 31.23 & $1.01\times$ / $2.81\times$ \\
\bottomrule
\end{tabular}
\end{table*}

Comparing True, Strong, and Ultra in Table~\ref{tab:supp_rae_synthetic_target_ablation} shows how target ambition steers algorithmic exploration when substantial efficiency headroom exists. Under the unshifted True target, search settles conservatively on standard multi-step schedules with modest held-out GenEval; raising the target to Strong pushes held-out GenEval to the highest value in this sweep ($59.53$), but still relies on costly uncached guidance ($44.17$\,TFLOPs). Only under the ambitious Ultra target does search break out of conservative schedules---discovering strided LoopGuidance with cross-step velocity-delta reuse that expands the lower-compute frontier (down to $16.09$\,TFLOPs, a $1.96\times$ speedup over Baseline and $5.45\times$ over Loop~+~LG) while achieving the top held-out DPG-Bench score at Balanced. Because Strong retains a slight held-out GenEval edge whereas Ultra unlocks much faster operating points, the preferred target depends on the deployment priority.

\FloatBarrier
\subsection{Search-Target Calibration in Autoregressive Text Reasoning}
\label{sec:supp_llm_pressure}

\Cref{tab:llm_pressure_ablation} expands the text-reasoning target study in RQ2 and RQ4. Read panel (a) as development ($829$ questions) and full-benchmark individual scores, and panel (b) as separate $3{,}316$-question held-out and $4{,}145$-question full-benchmark aggregates. Each \texttt{Gemini-4-Argon} search evaluates $80$ candidates on $829$ development questions, then replays frozen programs on all $4{,}145$ questions. The target is development Acc Norm, with shifts in percentage points rather than the three-coordinate target strength percentage for image diffusion. Non-looped is standard Qwen3-4B inference; Fixed Loop follows Training-Free Looped Transformers~\cite{chen2026trainingfreelooped}. Ours (True) is the instance-weighted (Micro) program from the True-target search; it is distinct from the task-balanced (Macro) program shown as Ours in \cref{tab:llm_reasoning} and \cref{tab:supp_llm_representatives}.

Unlike multi-step image diffusion, a frozen unlooped language model evaluated on discrete multiple-choice questions operates within a much tighter test-time gain envelope. In this regime, the grounded True target generalizes best to the $3{,}316$ unseen questions---leading held-out Micro Acc, Macro Domain, and full-set decision margin---whereas artificially inflated targets ($+1.57$ to $+6.03$\,pp) induce classic development-set overfitting: development accuracy ticks upward under Strong, yet every shifted target drops below both True and Fixed Loop on held-out Micro Acc (${\sim}0.4$\,pp drop). Together, Sections~\ref{sec:supp_rae_synthetic_targets} and~\ref{sec:supp_llm_pressure} establish a unified calibration principle: \emph{search targets should match the domain's available algorithmic headroom}---aspirational targets catalyze structural shortcuts in high-headroom multi-step diffusion, whereas grounded targets safeguard generalization in tighter discrete-reasoning regimes.

\begin{table*}[!htbp]
\centering
\caption{\textbf{\rqhighlight{2}{Measured (True) search targets generalize best on Qwen3-4B, illustrating domain-dependent target calibration.}} Panel~(a) reports development ($829$) and full-benchmark individual scores; panel~(b) contrasts $3{,}316$-question held-out aggregates against full $4{,}145$-question aggregates. Target shifts are percentage points, unlike the relative target strength percentages for image generation. \textbf{Bold}/\underline{underlined}: best/second-best per column.}
\label{tab:llm_pressure_ablation}
\begin{subtable}[t]{\textwidth}
\centering
\caption{\textbf{Development and Individual-Benchmark Scores.}}
\footnotesize
\setlength{\tabcolsep}{2.8pt}
\begin{tabular}{@{}l c | c c | c c c c c@{}}
\toprule
\multirow{2}{*}{\textbf{Method}} & \textbf{Search Target} & \multicolumn{2}{c|}{\textbf{Development (\%) $\uparrow$}} & \shortstack{\textbf{MMLU-}\\\textbf{STEM}} & \shortstack{\textbf{GPQA-}\\\textbf{Main}} & \multicolumn{2}{c}{\textbf{ARC-Challenge (\%) $\uparrow$}} & \textbf{SciQ} \\
\cmidrule(lr){3-4}\cmidrule(lr){7-8}
 & \shortstack{\textbf{(Acc Norm \%,}\\$\boldsymbol{\Delta}$\textbf{)}} & \textbf{Acc} & \textbf{Acc Norm} & \textbf{Acc (\%) $\uparrow$} & \textbf{Acc (\%) $\uparrow$} & \textbf{Acc} & \textbf{Acc Norm} & \textbf{Acc (\%) $\uparrow$} \\
\midrule
Non-looped~\cite{yang2025qwen3} & --- & 63.33 & 63.93 & 62.43 & 31.92 & 50.60 & \underline{54.18} & 95.70 \\
Fixed Loop~\cite{chen2026trainingfreelooped} & --- & 64.17 & 65.50 & 64.20 & 33.26 & \textbf{51.71} & \textbf{54.95} & \underline{96.20} \\
\midrule
\rowcolor{gray!12}
Ours (True) & $65.50$ ($+0.00$) & 66.10 & \textbf{67.31} & \textbf{64.85} & \underline{34.60} & \underline{51.54} & \textbf{54.95} & \textbf{96.50} \\
Ours (Mild) & $67.07$ ($+1.57$) & \underline{66.22} & \textbf{67.31} & 64.66 & \textbf{34.82} & 51.02 & 53.67 & 96.00 \\
Ours (Strong) & $68.52$ ($+3.02$) & \textbf{66.47} & \underline{67.19} & \underline{64.79} & 34.38 & 51.02 & 53.24 & 96.10 \\
Ours (Extreme) & $71.53$ ($+6.03$) & 65.50 & 67.07 & 64.59 & \underline{34.60} & 50.60 & 53.67 & 96.10 \\
\bottomrule
\end{tabular}
\end{subtable}
\par\medskip
\begin{subtable}[t]{\textwidth}
\centering
\caption{\textbf{Held-Out ($3{,}316$ Unseen Questions) vs.\ Full-Benchmark ($4{,}145$ Questions) Aggregate Scores.} Accuracies are percentages; Margin is dimensionless.}
\scriptsize
\setlength{\tabcolsep}{3.0pt}
\begin{tabular*}{\textwidth}{@{\extracolsep{\fill}}l | c c c c | c c c c c@{}}
\toprule
\multirow{2}{*}{\textbf{Method}} & \multicolumn{4}{c|}{\textbf{Held-out ($3{,}316$) (\%) $\uparrow$}} & \multicolumn{5}{c}{\textbf{Full ($4{,}145$) $\uparrow$}} \\
\cmidrule(lr){2-5}\cmidrule(lr){6-10}
 & \shortstack{\textbf{Micro}\\\textbf{Acc}} & \shortstack{\textbf{Micro}\\\textbf{Acc Norm}} & \shortstack{\textbf{Macro}\\\textbf{Group}} & \shortstack{\textbf{Macro}\\\textbf{Domain}} & \shortstack{\textbf{Micro}\\\textbf{Acc}} & \shortstack{\textbf{Micro}\\\textbf{Acc Norm}} & \shortstack{\textbf{Macro}\\\textbf{Group}} & \shortstack{\textbf{Macro}\\\textbf{Domain}} & \textbf{Margin $\uparrow$} \\
\midrule
Non-looped~\cite{yang2025qwen3} & 63.93 & 64.35 & 60.24 & 58.46 & 63.81 & 64.27 & 60.16 & 58.37 & 0.2919 \\
Fixed Loop~\cite{chen2026trainingfreelooped} & \underline{65.26} & \textbf{65.77} & \textbf{61.60} & 59.81 & 65.04 & \underline{65.72} & 61.34 & 59.60 & \underline{0.3132} \\
\midrule
\rowcolor{gray!12}
Ours (True) & \textbf{65.29} & \underline{65.71} & \underline{61.53} & \textbf{60.16} & \textbf{65.45} & \textbf{66.03} & \textbf{61.87} & \underline{60.46} & \textbf{0.3204} \\
Ours (Mild) & 64.87 & 65.29 & 61.16 & 59.96 & 65.14 & 65.69 & \underline{61.63} & 60.40 & 0.3080 \\
Ours (Strong) & 64.84 & 65.17 & 61.18 & 59.84 & \underline{65.16} & 65.57 & 61.57 & 60.25 & 0.3128 \\
Ours (Extreme) & 64.87 & 65.23 & 61.10 & \underline{60.11} & 64.99 & 65.60 & 61.47 & \textbf{60.51} & 0.3092 \\
\bottomrule
\end{tabular*}
\end{subtable}
\end{table*}
