# Supplementary material for: Evolving Loop Programs: Discovering How Frozen Transformers Should Loop
Source: arXiv:2611.41108 source file (2026-12-03)
Supplement: Supplementary file 14 [file appendix_vocabulary.tex]

\section{Vocabulary and Terminology}
\label{sec:supp_vocabulary}

Table~\ref{tab:terminology} distinguishes search, execution, and evaluation terms. The method and its notation are defined in Section~\ref{sec:method}.

\begin{nolinenumbers}
\begingroup
\small
\setlength{\tabcolsep}{6pt}
\renewcommand{\arraystretch}{1.12}
\begin{longtable}{@{}>{\raggedright\arraybackslash}p{0.245\textwidth} >{\raggedright\arraybackslash}p{\dimexpr0.755\textwidth-12pt\relax}@{}}
\caption{\textbf{Key distinctions used throughout the supplement.} Program definitions and the search procedure follow Section~\ref{sec:method}.}\label{tab:terminology}\\
\toprule
\textbf{Term / compact label} & \textbf{Meaning and usage in this paper} \\
\midrule
\endfirsthead
\multicolumn{2}{l}{\textbf{Table~\thetable\ (continued): Vocabulary and terminology}}\\
\toprule
\textbf{Term / compact label} & \textbf{Meaning and usage in this paper} \\
\midrule
\endhead
\midrule
\multicolumn{2}{r}{\emph{Continued on the next page}}\\
\endfoot
\bottomrule
\endlastfoot
Search round / loop pass / sampling step & A search round proposes and evaluates programs. A loop pass repeats a transformer block group; a sampling step advances diffusion and may contain several loop passes. \\
Frozen weights / frozen program & Backbone weights remain fixed during search and deployment. After selection, code and parameters are also fixed; runtime states still evolve. \\
Core Passes & Total passes through the Looped-DiT core across sampling steps, per reported branch: $\sum_t K_t$. \\
Dev. / Held-out / Full & Dev. guides search; held-out inputs are excluded from candidate search. Full includes development examples where specified. Selection using held-out scores is disclosed separately in Table~\ref{tab:supp_agent_pareto_balanced}(c). \\
Anchor / target / HV reference & Anchors are measured programs. Targets are desired scores supplied to the LLM. The hypervolume (HV) reference is fixed for reporting and is not changed by target shifts. \\
Target strength & Mean relative image-target increase over True across GenEval, DPG, and search-time latency speedup, in percent. Text-target shifts are reported separately in percentage points. \\
FLOPs speedup / latency speedup & Baseline-to-program ratios using operation count and measured runtime, respectively. Neither includes search cost. \\
Native / Full reference / Priority & Native is the pretrained loop configuration; Full reference is its full-budget setting, not an evaluation split. Priority identifies a selected program, not a universal selection formula. \\
Initial search context ($\mathcal{C}_0$) / Context-coupling & Initial instructions and starter operators in Eq.~\eqref{eq:program_evolution} ($\mathcal{C}_r$ at $r{=}0$). Coupled poles pair neutral instructions with an empty program template (\emph{Minimal context}) or concise algorithmic guidance with a starter operator library (\emph{Matched prior}); uncoupled partial priors supply only one component. \\
\end{longtable}
\endgroup
\end{nolinenumbers}
